# Supplementary material for: ThreadBench: Benchmarking Realism in Agentic Simulation of Real-world Discussions
Source: arXiv:2606.14715 source file (2026-10-10)
Supplement: Supplementary file 1 [file appendix_unified_baseline_pvalue_table.tex]

\clearpage
\begin{landscape}
{\scriptsize
\setlength{\tabcolsep}{2.6pt}

% [inline block 0: 2 envs, 64405 chars -> data_tex | \begin{longtable}{@{}L{1.50cm}L{3.00cm}L{3.10cm}*{4}{r}@{}} \caption{Unified OASIS baseline p-value comparison on MiroBe...]

}
\end{landscape}
