# Supplementary material for: ThreadBench: Benchmarking Realism in Agentic Simulation of Real-world Discussions
Source: arXiv:2606.14715 source file (2026-10-10)
Supplement: Supplementary file 2 [file A1-mirobench_appendix_full_table.tex]

% Generated by experiments/reddit_multidomain_baselines/scripts/
%   make_appendix_full_tables.py from artifacts/.../summary/holdout_all_arms.csv,
%   the same file Table 2 is built from.
\begin{table*}[p]
\centering
\large\setlength{\tabcolsep}{4.5pt}\renewcommand{\arraystretch}{0.90}
\caption{Distributional similarity between simulated and real discussions for every arm we ran, over the same held-out real population as Table~\ref{tab:holdout_pvalues}. Each cell gives MWU $p$-value/KS $p$-value; a metric passes when both exceed $\alpha=0.05$ (in bold). \textbf{Non-rej.} is the percentage of the 24 tests (12 metrics $\times$ 2 tests) that do not reject.}
\label{tab:full_domain_metric_comparison}
\resizebox{\textwidth}{!}{%
\begin{tabular}{@{}lll|ccc|ccc|cc|cccc|c@{}}
\toprule
& & & \multicolumn{3}{c}{\textit{Uniformity}} & \multicolumn{3}{c}{\textit{Interaction}} & \multicolumn{2}{c}{\textit{Expression}} & \multicolumn{4}{c}{\textit{Tone}} & \\
\cmidrule(lr){4-6}\cmidrule(lr){7-9}\cmidrule(lr){10-11}\cmidrule(lr){12-15}
\textbf{Domain} & \textbf{Method} & \textbf{Model} & \rotatebox{90}{Self-BLEU} & \rotatebox{90}{Self-BERT} & \rotatebox{90}{Sem.Cos} & \rotatebox{90}{Depth} & \rotatebox{90}{Virality} & \rotatebox{90}{Len.CV} & \rotatebox{90}{Story} & \rotatebox{90}{Emotion} & \rotatebox{90}{Polite} & \rotatebox{90}{Neutral} & \rotatebox{90}{Impolite} & \rotatebox{90}{Disagr.} & \textbf{Non-rej.} \\
\midrule
\multirow{10}{*}{\rotatebox{90}{\textbf{Camera}}} & \multirow{3}{*}{OASIS} & \texttt{DeepSeek-V4.1-Flash} & \textcolor{black!45}{$<$.01/$<$.01} & \textcolor{black!45}{$<$.01/$<$.01} & \textcolor{black!45}{$<$.01/$<$.01} & \textcolor{black!45}{$<$.01/$<$.01} & \textcolor{black!45}{$<$.01/$<$.01} & \textcolor{black!45}{$<$.01/$<$.01} & \textcolor{black!45}{$<$.01/$<$.01} & \textcolor{black!45}{$<$.01/$<$.01} & \textcolor{black!45}{$<$.01/$<$.01} & \textcolor{black!45}{$<$.01/$<$.01} & \textcolor{black!45}{.08/.03} & \textbf{.46/.06} & \textcolor{black!55}{12\%} \\
 &  & \texttt{gpt-5.4-mini} & \textcolor{black!45}{$<$.01/$<$.01} & \textcolor{black!45}{$<$.01/$<$.01} & \textcolor{black!45}{$<$.01/$<$.01} & \textcolor{black!45}{$<$.01/$<$.01} & \textcolor{black!45}{$<$.01/$<$.01} & \textcolor{black!45}{$<$.01/$<$.01} & \textcolor{black!45}{$<$.01/$<$.01} & \textcolor{black!45}{$<$.01/$<$.01} & \textcolor{black!45}{$<$.01/$<$.01} & \textcolor{black!45}{$<$.01/$<$.01} & \textcolor{black!45}{$<$.01/$<$.01} & \textcolor{black!45}{$<$.01/$<$.01} & \textcolor{black!55}{0\%} \\
 &  & \texttt{gpt-4o-mini} & \textcolor{black!45}{$<$.01/$<$.01} & \textcolor{black!45}{$<$.01/$<$.01} & \textcolor{black!45}{$<$.01/$<$.01} & \textcolor{black!45}{$<$.01/$<$.01} & \textcolor{black!45}{$<$.01/$<$.01} & \textcolor{black!45}{$<$.01/$<$.01} & \textcolor{black!45}{$<$.01/$<$.01} & \textcolor{black!45}{$<$.01/$<$.01} & \textcolor{black!45}{$<$.01/$<$.01} & \textcolor{black!45}{$<$.01/$<$.01} & \textcolor{black!45}{$<$.01/$<$.01} & \textcolor{black!45}{$<$.01/$<$.01} & \textcolor{black!55}{0\%} \\
\cmidrule(l){2-16}
 & \multirow{4}{*}{SynthPAI} & \texttt{DeepSeek-V4.1-Flash} & \textcolor{black!45}{$<$.01/$<$.01} & \textcolor{black!45}{$<$.01/$<$.01} & \textbf{.08/.11} & \textcolor{black!45}{.01/$<$.01} & \textcolor{black!45}{.39/.03} & \textcolor{black!45}{$<$.01/$<$.01} & \textcolor{black!45}{$<$.01/$<$.01} & \textcolor{black!45}{$<$.01/$<$.01} & \textcolor{black!45}{$<$.01/$<$.01} & \textcolor{black!45}{$<$.01/$<$.01} & \textcolor{black!45}{$<$.01/$<$.01} & \textcolor{black!45}{$<$.01/$<$.01} & \textcolor{black!55}{12\%} \\
 &  & \texttt{gpt-5.4-mini} & \textcolor{black!45}{$<$.01/$<$.01} & \textcolor{black!45}{$<$.01/$<$.01} & \textbf{.55/.14} & \textcolor{black!45}{$<$.01/$<$.01} & \textcolor{black!45}{$<$.01/$<$.01} & \textcolor{black!45}{.46/$<$.01} & \textcolor{black!45}{$<$.01/$<$.01} & \textcolor{black!45}{$<$.01/$<$.01} & \textcolor{black!45}{$<$.01/$<$.01} & \textcolor{black!45}{.03/.07} & \textcolor{black!45}{$<$.01/$<$.01} & \textcolor{black!45}{$<$.01/$<$.01} & \textcolor{black!55}{17\%} \\
 &  & \texttt{gpt-4o-mini} & \textcolor{black!45}{$<$.01/$<$.01} & \textcolor{black!45}{$<$.01/$<$.01} & \textcolor{black!45}{$<$.01/$<$.01} & \textcolor{black!45}{.05/$<$.01} & \textbf{.85/.22} & \textcolor{black!45}{$<$.01/$<$.01} & \textcolor{black!45}{$<$.01/$<$.01} & \textcolor{black!45}{$<$.01/$<$.01} & \textbf{.07/.17} & \textcolor{black!45}{$<$.01/$<$.01} & \textcolor{black!45}{$<$.01/$<$.01} & \textcolor{black!45}{$<$.01/$<$.01} & \textcolor{black!55}{17\%} \\
 &  & \texttt{Gemini-2.5-Flash} & \textcolor{black!45}{$<$.01/$<$.01} & \textcolor{black!45}{$<$.01/$<$.01} & \textcolor{black!45}{$<$.01/$<$.01} & \textcolor{black!45}{$<$.01/$<$.01} & \textcolor{black!45}{$<$.01/$<$.01} & \textcolor{black!45}{$<$.01/$<$.01} & \textcolor{black!45}{$<$.01/$<$.01} & \textcolor{black!45}{$<$.01/$<$.01} & \textcolor{black!45}{$<$.01/$<$.01} & \textcolor{black!45}{$<$.01/.02} & \textcolor{black!45}{$<$.01/$<$.01} & \textcolor{black!45}{$<$.01/$<$.01} & \textcolor{black!55}{0\%} \\
\cmidrule(l){2-16}
 & \multirow{3}{*}{\textbf{ThreadPDG}} & \texttt{DeepSeek-V4.1-Flash} & \textbf{.44/.71} & \textbf{.92/.28} & \textbf{.68/.44} & \textbf{.86/.98} & \textbf{.81/.85} & \textbf{.21/.44} & \textbf{.15/.16} & \textbf{.50/.79} & \textbf{.76/.33} & \textbf{.15/.07} & \textcolor{black!45}{$<$.01/.05} & \textbf{.10/.09} & \textbf{96\%} \\
 &  & \texttt{gpt-5.4-mini} & \textcolor{black!45}{.12/.01} & \textbf{.27/.19} & \textbf{.72/.61} & \textbf{.98/.92} & \textbf{.70/.57} & \textbf{.70/.34} & \textbf{.17/.51} & \textbf{.65/.65} & \textcolor{black!45}{.02/$<$.01} & \textbf{.06/.20} & \textbf{.83/.90} & \textbf{.19/.37} & \textbf{88\%} \\
 &  & \texttt{gpt-4o-mini} & \textcolor{black!45}{.03/.02} & \textcolor{black!45}{$<$.01/$<$.01} & \textcolor{black!45}{$<$.01/$<$.01} & \textbf{.41/.37} & \textbf{.23/.23} & \textcolor{black!45}{$<$.01/$<$.01} & \textcolor{black!45}{$<$.01/$<$.01} & \textcolor{black!45}{$<$.01/$<$.01} & \textcolor{black!45}{$<$.01/$<$.01} & \textcolor{black!45}{$<$.01/$<$.01} & \textcolor{black!45}{$<$.01/$<$.01} & \textcolor{black!45}{$<$.01/$<$.01} & \textcolor{black!55}{17\%} \\
\midrule
\multirow{10}{*}{\rotatebox{90}{\textbf{Celebrity}}} & \multirow{3}{*}{OASIS} & \texttt{DeepSeek-V4.1-Flash} & \textcolor{black!45}{$<$.01/$<$.01} & \textcolor{black!45}{$<$.01/$<$.01} & \textcolor{black!45}{$<$.01/$<$.01} & \textcolor{black!45}{$<$.01/$<$.01} & \textcolor{black!45}{$<$.01/$<$.01} & \textcolor{black!45}{$<$.01/$<$.01} & \textcolor{black!45}{$<$.01/$<$.01} & \textcolor{black!45}{$<$.01/$<$.01} & \textcolor{black!45}{$<$.01/$<$.01} & \textcolor{black!45}{$<$.01/$<$.01} & \textbf{.67/.15} & \textcolor{black!45}{$<$.01/$<$.01} & \textcolor{black!55}{8\%} \\
 &  & \texttt{gpt-5.4-mini} & \textcolor{black!45}{$<$.01/$<$.01} & \textcolor{black!45}{$<$.01/$<$.01} & \textcolor{black!45}{$<$.01/$<$.01} & \textcolor{black!45}{$<$.01/$<$.01} & \textcolor{black!45}{$<$.01/$<$.01} & \textcolor{black!45}{$<$.01/$<$.01} & \textcolor{black!45}{$<$.01/$<$.01} & \textcolor{black!45}{$<$.01/$<$.01} & \textcolor{black!45}{$<$.01/$<$.01} & \textcolor{black!45}{$<$.01/$<$.01} & \textcolor{black!45}{$<$.01/$<$.01} & \textbf{.37/.27} & \textcolor{black!55}{8\%} \\
 &  & \texttt{gpt-4o-mini} & \textcolor{black!45}{$<$.01/$<$.01} & \textcolor{black!45}{$<$.01/$<$.01} & \textcolor{black!45}{$<$.01/$<$.01} & \textcolor{black!45}{$<$.01/$<$.01} & \textcolor{black!45}{$<$.01/$<$.01} & \textcolor{black!45}{$<$.01/$<$.01} & \textcolor{black!45}{$<$.01/$<$.01} & \textcolor{black!45}{$<$.01/$<$.01} & \textcolor{black!45}{$<$.01/$<$.01} & \textcolor{black!45}{$<$.01/$<$.01} & \textcolor{black!45}{$<$.01/$<$.01} & \textcolor{black!45}{.15/$<$.01} & \textcolor{black!55}{4\%} \\
\cmidrule(l){2-16}
 & \multirow{4}{*}{SynthPAI} & \texttt{DeepSeek-V4.1-Flash} & \textcolor{black!45}{$<$.01/$<$.01} & \textcolor{black!45}{$<$.01/$<$.01} & \textcolor{black!45}{$<$.01/$<$.01} & \textcolor{black!45}{$<$.01/$<$.01} & \textcolor{black!45}{$<$.01/$<$.01} & \textcolor{black!45}{$<$.01/$<$.01} & \textcolor{black!45}{$<$.01/$<$.01} & \textcolor{black!45}{$<$.01/$<$.01} & \textcolor{black!45}{$<$.01/$<$.01} & \textcolor{black!45}{.02/.02} & \textcolor{black!45}{$<$.01/$<$.01} & \textcolor{black!45}{$<$.01/$<$.01} & \textcolor{black!55}{0\%} \\
 &  & \texttt{gpt-5.4-mini} & \textcolor{black!45}{$<$.01/$<$.01} & \textcolor{black!45}{$<$.01/$<$.01} & \textcolor{black!45}{$<$.01/$<$.01} & \textcolor{black!45}{$<$.01/$<$.01} & \textcolor{black!45}{$<$.01/$<$.01} & \textcolor{black!45}{.11/$<$.01} & \textcolor{black!45}{$<$.01/$<$.01} & \textcolor{black!45}{$<$.01/$<$.01} & \textcolor{black!45}{$<$.01/$<$.01} & \textcolor{black!45}{.02/$<$.01} & \textcolor{black!45}{$<$.01/$<$.01} & \textcolor{black!45}{.03/.02} & \textcolor{black!55}{4\%} \\
 &  & \texttt{gpt-4o-mini} & \textcolor{black!45}{$<$.01/$<$.01} & \textcolor{black!45}{$<$.01/$<$.01} & \textcolor{black!45}{$<$.01/$<$.01} & \textcolor{black!45}{$<$.01/$<$.01} & \textcolor{black!45}{$<$.01/$<$.01} & \textcolor{black!45}{$<$.01/$<$.01} & \textcolor{black!45}{$<$.01/$<$.01} & \textcolor{black!45}{$<$.01/$<$.01} & \textcolor{black!45}{$<$.01/$<$.01} & \textcolor{black!45}{$<$.01/$<$.01} & \textcolor{black!45}{$<$.01/$<$.01} & \textcolor{black!45}{$<$.01/$<$.01} & \textcolor{black!55}{0\%} \\
 &  & \texttt{Gemini-2.5-Flash} & \textcolor{black!45}{$<$.01/$<$.01} & \textcolor{black!45}{$<$.01/$<$.01} & \textcolor{black!45}{$<$.01/$<$.01} & \textcolor{black!45}{$<$.01/$<$.01} & \textcolor{black!45}{$<$.01/$<$.01} & \textcolor{black!45}{$<$.01/$<$.01} & \textcolor{black!45}{$<$.01/$<$.01} & \textcolor{black!45}{$<$.01/$<$.01} & \textcolor{black!45}{$<$.01/$<$.01} & \textbf{.36/.08} & \textcolor{black!45}{$<$.01/$<$.01} & \textcolor{black!45}{.01/$<$.01} & \textcolor{black!55}{8\%} \\
\cmidrule(l){2-16}
 & \multirow{3}{*}{\textbf{ThreadPDG}} & \texttt{DeepSeek-V4.1-Flash} & \textbf{.77/.71} & \textbf{.77/.88} & \textbf{.90/.88} & \textbf{.58/.56} & \textbf{.30/.33} & \textbf{.05/.20} & \textbf{.56/.67} & \textbf{.67/.80} & \textbf{.72/.55} & \textbf{.68/.77} & \textbf{.69/.66} & \textbf{.78/.64} & \textbf{100\%} \\
 &  & \texttt{gpt-5.4-mini} & \textbf{.12/.12} & \textbf{.29/.70} & \textbf{.91/.79} & \textbf{.56/.50} & \textbf{.26/.22} & \textbf{.17/.11} & \textbf{.24/.53} & \textbf{.49/.52} & \textcolor{black!45}{.05/.06} & \textbf{.58/.45} & \textbf{.31/.43} & \textbf{.41/.62} & \textbf{96\%} \\
 &  & \texttt{gpt-4o-mini} & \textcolor{black!45}{$<$.01/$<$.01} & \textcolor{black!45}{$<$.01/$<$.01} & \textcolor{black!45}{$<$.01/$<$.01} & \textbf{.77/.71} & \textbf{.91/.83} & \textcolor{black!45}{.04/.05} & \textcolor{black!45}{$<$.01/.02} & \textcolor{black!45}{$<$.01/$<$.01} & \textcolor{black!45}{$<$.01/$<$.01} & \textcolor{black!45}{$<$.01/.01} & \textbf{.51/.92} & \textcolor{black!45}{$<$.01/$<$.01} & \textcolor{black!55}{29\%} \\
\midrule
\multirow{10}{*}{\rotatebox{90}{\textbf{Cellphone}}} & \multirow{3}{*}{OASIS} & \texttt{DeepSeek-V4.1-Flash} & \textcolor{black!45}{$<$.01/$<$.01} & \textcolor{black!45}{$<$.01/$<$.01} & \textcolor{black!45}{$<$.01/$<$.01} & \textcolor{black!45}{$<$.01/$<$.01} & \textcolor{black!45}{$<$.01/$<$.01} & \textcolor{black!45}{$<$.01/$<$.01} & \textcolor{black!45}{$<$.01/$<$.01} & \textcolor{black!45}{$<$.01/$<$.01} & \textcolor{black!45}{$<$.01/$<$.01} & \textcolor{black!45}{$<$.01/$<$.01} & \textcolor{black!45}{$<$.01/$<$.01} & \textbf{.87/.90} & \textcolor{black!55}{8\%} \\
 &  & \texttt{gpt-5.4-mini} & \textcolor{black!45}{$<$.01/$<$.01} & \textcolor{black!45}{$<$.01/$<$.01} & \textcolor{black!45}{$<$.01/$<$.01} & \textcolor{black!45}{$<$.01/$<$.01} & \textcolor{black!45}{$<$.01/$<$.01} & \textcolor{black!45}{$<$.01/$<$.01} & \textcolor{black!45}{$<$.01/$<$.01} & \textcolor{black!45}{$<$.01/$<$.01} & \textcolor{black!45}{$<$.01/$<$.01} & \textcolor{black!45}{$<$.01/$<$.01} & \textcolor{black!45}{$<$.01/$<$.01} & \textbf{.93/.20} & \textcolor{black!55}{8\%} \\
 &  & \texttt{gpt-4o-mini} & \textcolor{black!45}{$<$.01/$<$.01} & \textcolor{black!45}{$<$.01/$<$.01} & \textcolor{black!45}{$<$.01/$<$.01} & \textcolor{black!45}{$<$.01/$<$.01} & \textcolor{black!45}{$<$.01/$<$.01} & \textcolor{black!45}{$<$.01/$<$.01} & \textcolor{black!45}{$<$.01/$<$.01} & \textcolor{black!45}{.05/$<$.01} & \textcolor{black!45}{$<$.01/$<$.01} & \textcolor{black!45}{$<$.01/$<$.01} & \textcolor{black!45}{$<$.01/$<$.01} & \textcolor{black!45}{.05/.01} & \textcolor{black!55}{8\%} \\
\cmidrule(l){2-16}
 & \multirow{4}{*}{SynthPAI} & \texttt{DeepSeek-V4.1-Flash} & \textcolor{black!45}{$<$.01/$<$.01} & \textcolor{black!45}{$<$.01/$<$.01} & \textbf{.17/.12} & \textcolor{black!45}{$<$.01/$<$.01} & \textcolor{black!45}{$<$.01/$<$.01} & \textcolor{black!45}{$<$.01/$<$.01} & \textcolor{black!45}{$<$.01/$<$.01} & \textcolor{black!45}{.17/.03} & \textcolor{black!45}{$<$.01/$<$.01} & \textcolor{black!45}{$<$.01/$<$.01} & \textcolor{black!45}{$<$.01/$<$.01} & \textcolor{black!45}{$<$.01/$<$.01} & \textcolor{black!55}{12\%} \\
 &  & \texttt{gpt-5.4-mini} & \textcolor{black!45}{$<$.01/$<$.01} & \textcolor{black!45}{$<$.01/$<$.01} & \textbf{.64/.06} & \textcolor{black!45}{$<$.01/$<$.01} & \textcolor{black!45}{$<$.01/$<$.01} & \textcolor{black!45}{.07/$<$.01} & \textcolor{black!45}{$<$.01/$<$.01} & \textcolor{black!45}{$<$.01/$<$.01} & \textcolor{black!45}{$<$.01/$<$.01} & \textcolor{black!45}{$<$.01/$<$.01} & \textcolor{black!45}{$<$.01/$<$.01} & \textcolor{black!45}{$<$.01/$<$.01} & \textcolor{black!55}{12\%} \\
 &  & \texttt{gpt-4o-mini} & \textcolor{black!45}{$<$.01/$<$.01} & \textcolor{black!45}{$<$.01/$<$.01} & \textcolor{black!45}{$<$.01/$<$.01} & \textcolor{black!45}{$<$.01/$<$.01} & \textbf{.63/.26} & \textcolor{black!45}{$<$.01/$<$.01} & \textcolor{black!45}{$<$.01/$<$.01} & \textcolor{black!45}{.11/$<$.01} & \textcolor{black!45}{$<$.01/$<$.01} & \textcolor{black!45}{$<$.01/$<$.01} & \textcolor{black!45}{$<$.01/$<$.01} & \textcolor{black!45}{$<$.01/$<$.01} & \textcolor{black!55}{12\%} \\
 &  & \texttt{Gemini-2.5-Flash} & \textcolor{black!45}{$<$.01/$<$.01} & \textcolor{black!45}{$<$.01/$<$.01} & \textcolor{black!45}{$<$.01/$<$.01} & \textcolor{black!45}{$<$.01/$<$.01} & \textcolor{black!45}{$<$.01/$<$.01} & \textcolor{black!45}{$<$.01/$<$.01} & \textcolor{black!45}{$<$.01/$<$.01} & \textcolor{black!45}{.90/.03} & \textcolor{black!45}{$<$.01/$<$.01} & \textcolor{black!45}{$<$.01/$<$.01} & \textcolor{black!45}{$<$.01/$<$.01} & \textcolor{black!45}{$<$.01/$<$.01} & \textcolor{black!55}{4\%} \\
\cmidrule(l){2-16}
 & \multirow{3}{*}{\textbf{ThreadPDG}} & \texttt{DeepSeek-V4.1-Flash} & \textbf{.09/.42} & \textbf{.23/.33} & \textbf{.90/.35} & \textbf{.43/.41} & \textbf{.20/.43} & \textcolor{black!45}{.07/$<$.01} & \textbf{.78/.42} & \textbf{.12/.08} & \textbf{.18/.15} & \textbf{.97/1.0} & \textbf{.05/.13} & \textcolor{black!45}{$<$.01/.01} & \textbf{88\%} \\
 &  & \texttt{gpt-5.4-mini} & \textcolor{black!45}{$<$.01/.04} & \textbf{.95/.70} & \textbf{.13/.41} & \textbf{.76/.70} & \textbf{.91/.93} & \textbf{.31/.49} & \textbf{.92/.88} & \textbf{.84/.55} & \textcolor{black!45}{$<$.01/$<$.01} & \textbf{.26/.12} & \textbf{.17/.33} & \textbf{.17/.27} & \textbf{83\%} \\
 &  & \texttt{gpt-4o-mini} & \textbf{.55/.72} & \textcolor{black!45}{$<$.01/$<$.01} & \textcolor{black!45}{$<$.01/$<$.01} & \textbf{.07/.16} & \textcolor{black!45}{.01/.04} & \textcolor{black!45}{$<$.01/$<$.01} & \textcolor{black!45}{$<$.01/.06} & \textcolor{black!45}{$<$.01/$<$.01} & \textbf{.46/.29} & \textbf{.20/.15} & \textcolor{black!45}{.02/.02} & \textbf{.10/.07} & \textcolor{black!55}{46\%} \\
\midrule
\multirow{10}{*}{\rotatebox{90}{\textbf{Game}}} & \multirow{3}{*}{OASIS} & \texttt{DeepSeek-V4.1-Flash} & \textbf{.07/.18} & \textcolor{black!45}{$<$.01/$<$.01} & \textcolor{black!45}{$<$.01/$<$.01} & \textcolor{black!45}{$<$.01/$<$.01} & \textcolor{black!45}{$<$.01/$<$.01} & \textcolor{black!45}{$<$.01/$<$.01} & \textcolor{black!45}{$<$.01/$<$.01} & \textcolor{black!45}{$<$.01/$<$.01} & \textcolor{black!45}{$<$.01/$<$.01} & \textcolor{black!45}{$<$.01/$<$.01} & \textcolor{black!45}{$<$.01/$<$.01} & \textbf{.08/.08} & \textcolor{black!55}{17\%} \\
 &  & \texttt{gpt-5.4-mini} & \textcolor{black!45}{$<$.01/$<$.01} & \textcolor{black!45}{$<$.01/$<$.01} & \textcolor{black!45}{$<$.01/$<$.01} & \textcolor{black!45}{$<$.01/$<$.01} & \textcolor{black!45}{$<$.01/$<$.01} & \textcolor{black!45}{$<$.01/$<$.01} & \textcolor{black!45}{$<$.01/$<$.01} & \textcolor{black!45}{$<$.01/$<$.01} & \textcolor{black!45}{$<$.01/$<$.01} & \textcolor{black!45}{$<$.01/$<$.01} & \textcolor{black!45}{$<$.01/$<$.01} & \textcolor{black!45}{.20/.02} & \textcolor{black!55}{4\%} \\
 &  & \texttt{gpt-4o-mini} & \textcolor{black!45}{$<$.01/$<$.01} & \textcolor{black!45}{$<$.01/$<$.01} & \textcolor{black!45}{$<$.01/$<$.01} & \textcolor{black!45}{$<$.01/$<$.01} & \textcolor{black!45}{$<$.01/$<$.01} & \textcolor{black!45}{$<$.01/$<$.01} & \textcolor{black!45}{$<$.01/$<$.01} & \textcolor{black!45}{$<$.01/$<$.01} & \textcolor{black!45}{$<$.01/$<$.01} & \textcolor{black!45}{$<$.01/$<$.01} & \textcolor{black!45}{$<$.01/$<$.01} & \textcolor{black!45}{$<$.01/$<$.01} & \textcolor{black!55}{0\%} \\
\cmidrule(l){2-16}
 & \multirow{4}{*}{SynthPAI} & \texttt{DeepSeek-V4.1-Flash} & \textcolor{black!45}{$<$.01/$<$.01} & \textcolor{black!45}{$<$.01/$<$.01} & \textcolor{black!45}{$<$.01/$<$.01} & \textcolor{black!45}{$<$.01/$<$.01} & \textcolor{black!45}{$<$.01/$<$.01} & \textcolor{black!45}{$<$.01/$<$.01} & \textcolor{black!45}{$<$.01/$<$.01} & \textcolor{black!45}{$<$.01/$<$.01} & \textcolor{black!45}{$<$.01/$<$.01} & \textcolor{black!45}{$<$.01/$<$.01} & \textcolor{black!45}{$<$.01/$<$.01} & \textbf{.08/.07} & \textcolor{black!55}{8\%} \\
 &  & \texttt{gpt-5.4-mini} & \textcolor{black!45}{$<$.01/$<$.01} & \textcolor{black!45}{$<$.01/$<$.01} & \textbf{.07/.07} & \textcolor{black!45}{$<$.01/$<$.01} & \textcolor{black!45}{$<$.01/$<$.01} & \textcolor{black!45}{.04/$<$.01} & \textcolor{black!45}{$<$.01/$<$.01} & \textcolor{black!45}{$<$.01/$<$.01} & \textcolor{black!45}{$<$.01/$<$.01} & \textbf{.37/.63} & \textcolor{black!45}{$<$.01/$<$.01} & \textcolor{black!45}{.02/$<$.01} & \textcolor{black!55}{17\%} \\
 &  & \texttt{gpt-4o-mini} & \textcolor{black!45}{$<$.01/$<$.01} & \textcolor{black!45}{$<$.01/$<$.01} & \textcolor{black!45}{$<$.01/$<$.01} & \textcolor{black!45}{$<$.01/$<$.01} & \textcolor{black!45}{.48/.01} & \textcolor{black!45}{$<$.01/$<$.01} & \textcolor{black!45}{$<$.01/$<$.01} & \textcolor{black!45}{$<$.01/$<$.01} & \textcolor{black!45}{$<$.01/$<$.01} & \textcolor{black!45}{$<$.01/$<$.01} & \textcolor{black!45}{$<$.01/$<$.01} & \textcolor{black!45}{$<$.01/$<$.01} & \textcolor{black!55}{4\%} \\
 &  & \texttt{Gemini-2.5-Flash} & \textcolor{black!45}{$<$.01/$<$.01} & \textcolor{black!45}{$<$.01/$<$.01} & \textcolor{black!45}{$<$.01/$<$.01} & \textcolor{black!45}{$<$.01/$<$.01} & \textcolor{black!45}{$<$.01/$<$.01} & \textcolor{black!45}{$<$.01/$<$.01} & \textcolor{black!45}{$<$.01/$<$.01} & \textcolor{black!45}{$<$.01/$<$.01} & \textcolor{black!45}{$<$.01/$<$.01} & \textcolor{black!45}{$<$.01/$<$.01} & \textcolor{black!45}{$<$.01/$<$.01} & \textcolor{black!45}{$<$.01/$<$.01} & \textcolor{black!55}{0\%} \\
\cmidrule(l){2-16}
 & \multirow{3}{*}{\textbf{ThreadPDG}} & \texttt{DeepSeek-V4.1-Flash} & \textbf{.75/.51} & \textbf{.11/.08} & \textbf{.15/.45} & \textbf{.18/.28} & \textcolor{black!45}{.03/.05} & \textbf{.71/.69} & \textbf{.71/.91} & \textbf{.30/.22} & \textbf{.17/.05} & \textbf{.60/.63} & \textbf{.88/.36} & \textcolor{black!45}{$<$.01/$<$.01} & \textbf{83\%} \\
 &  & \texttt{gpt-5.4-mini} & \textbf{.36/.72} & \textcolor{black!45}{.03/.02} & \textbf{.29/.63} & \textbf{.19/.29} & \textcolor{black!45}{.07/.03} & \textbf{.22/.29} & \textbf{.93/1.0} & \textbf{.70/.53} & \textcolor{black!45}{.03/.02} & \textbf{.63/.89} & \textbf{.46/.53} & \textcolor{black!45}{$<$.01/$<$.01} & \textbf{71\%} \\
 &  & \texttt{gpt-4o-mini} & \textcolor{black!45}{$<$.01/$<$.01} & \textcolor{black!45}{$<$.01/$<$.01} & \textcolor{black!45}{$<$.01/$<$.01} & \textbf{.06/.07} & \textcolor{black!45}{.01/.03} & \textcolor{black!45}{$<$.01/$<$.01} & \textbf{.69/.84} & \textcolor{black!45}{$<$.01/$<$.01} & \textcolor{black!45}{$<$.01/$<$.01} & \textcolor{black!45}{.02/.04} & \textcolor{black!45}{$<$.01/$<$.01} & \textbf{.67/.53} & \textcolor{black!55}{25\%} \\
\midrule
\multirow{10}{*}{\rotatebox{90}{\textbf{Health Issue}}} & \multirow{3}{*}{OASIS} & \texttt{DeepSeek-V4.1-Flash} & \textcolor{black!45}{$<$.01/$<$.01} & \textcolor{black!45}{$<$.01/$<$.01} & \textcolor{black!45}{$<$.01/$<$.01} & \textcolor{black!45}{$<$.01/$<$.01} & \textcolor{black!45}{$<$.01/$<$.01} & \textcolor{black!45}{$<$.01/$<$.01} & \textcolor{black!45}{.02/.15} & \textcolor{black!45}{$<$.01/$<$.01} & \textbf{.08/.09} & \textcolor{black!45}{$<$.01/$<$.01} & \textcolor{black!45}{$<$.01/$<$.01} & \textcolor{black!45}{$<$.01/$<$.01} & \textcolor{black!55}{12\%} \\
 &  & \texttt{gpt-5.4-mini} & \textcolor{black!45}{$<$.01/$<$.01} & \textcolor{black!45}{$<$.01/$<$.01} & \textcolor{black!45}{$<$.01/$<$.01} & \textcolor{black!45}{$<$.01/$<$.01} & \textcolor{black!45}{$<$.01/$<$.01} & \textcolor{black!45}{$<$.01/$<$.01} & \textcolor{black!45}{$<$.01/$<$.01} & \textcolor{black!45}{$<$.01/$<$.01} & \textcolor{black!45}{$<$.01/$<$.01} & \textcolor{black!45}{$<$.01/$<$.01} & \textcolor{black!45}{$<$.01/$<$.01} & \textbf{.51/.10} & \textcolor{black!55}{8\%} \\
 &  & \texttt{gpt-4o-mini} & \textcolor{black!45}{$<$.01/$<$.01} & \textcolor{black!45}{$<$.01/$<$.01} & \textcolor{black!45}{$<$.01/$<$.01} & \textcolor{black!45}{$<$.01/$<$.01} & \textcolor{black!45}{$<$.01/$<$.01} & \textcolor{black!45}{$<$.01/$<$.01} & \textcolor{black!45}{$<$.01/$<$.01} & \textcolor{black!45}{$<$.01/$<$.01} & \textcolor{black!45}{$<$.01/$<$.01} & \textcolor{black!45}{$<$.01/$<$.01} & \textcolor{black!45}{$<$.01/$<$.01} & \textbf{.79/.66} & \textcolor{black!55}{8\%} \\
\cmidrule(l){2-16}
 & \multirow{4}{*}{SynthPAI} & \texttt{DeepSeek-V4.1-Flash} & \textcolor{black!45}{$<$.01/$<$.01} & \textcolor{black!45}{$<$.01/$<$.01} & \textbf{.47/.57} & \textcolor{black!45}{$<$.01/$<$.01} & \textcolor{black!45}{$<$.01/$<$.01} & \textcolor{black!45}{$<$.01/$<$.01} & \textcolor{black!45}{$<$.01/$<$.01} & \textbf{.49/.19} & \textcolor{black!45}{$<$.01/$<$.01} & \textcolor{black!45}{$<$.01/$<$.01} & \textcolor{black!45}{$<$.01/$<$.01} & \textcolor{black!45}{$<$.01/$<$.01} & \textcolor{black!55}{17\%} \\
 &  & \texttt{gpt-5.4-mini} & \textcolor{black!45}{$<$.01/$<$.01} & \textcolor{black!45}{$<$.01/$<$.01} & \textbf{.43/.57} & \textcolor{black!45}{$<$.01/$<$.01} & \textcolor{black!45}{$<$.01/$<$.01} & \textcolor{black!45}{.66/$<$.01} & \textcolor{black!45}{$<$.01/$<$.01} & \textcolor{black!45}{$<$.01/$<$.01} & \textcolor{black!45}{$<$.01/$<$.01} & \textcolor{black!45}{.13/.02} & \textcolor{black!45}{$<$.01/$<$.01} & \textcolor{black!45}{$<$.01/$<$.01} & \textcolor{black!55}{17\%} \\
 &  & \texttt{gpt-4o-mini} & \textcolor{black!45}{$<$.01/$<$.01} & \textcolor{black!45}{$<$.01/$<$.01} & \textcolor{black!45}{$<$.01/$<$.01} & \textcolor{black!45}{$<$.01/$<$.01} & \textcolor{black!45}{$<$.01/$<$.01} & \textcolor{black!45}{$<$.01/$<$.01} & \textcolor{black!45}{$<$.01/$<$.01} & \textcolor{black!45}{$<$.01/$<$.01} & \textcolor{black!45}{$<$.01/$<$.01} & \textcolor{black!45}{$<$.01/$<$.01} & \textcolor{black!45}{$<$.01/$<$.01} & \textcolor{black!45}{$<$.01/$<$.01} & \textcolor{black!55}{0\%} \\
 &  & \texttt{Gemini-2.5-Flash} & \textcolor{black!45}{$<$.01/$<$.01} & \textcolor{black!45}{$<$.01/$<$.01} & \textcolor{black!45}{$<$.01/$<$.01} & \textcolor{black!45}{$<$.01/$<$.01} & \textcolor{black!45}{$<$.01/$<$.01} & \textcolor{black!45}{$<$.01/$<$.01} & \textcolor{black!45}{$<$.01/$<$.01} & \textbf{.49/.09} & \textcolor{black!45}{$<$.01/$<$.01} & \textcolor{black!45}{$<$.01/$<$.01} & \textcolor{black!45}{$<$.01/$<$.01} & \textcolor{black!45}{$<$.01/$<$.01} & \textcolor{black!55}{8\%} \\
\cmidrule(l){2-16}
 & \multirow{3}{*}{\textbf{ThreadPDG}} & \texttt{DeepSeek-V4.1-Flash} & \textcolor{black!45}{.02/.02} & \textcolor{black!45}{.02/.14} & \textbf{.40/.53} & \textbf{.48/.23} & \textbf{.39/.72} & \textbf{.74/.36} & \textbf{.37/.72} & \textbf{.35/.36} & \textcolor{black!45}{$<$.01/$<$.01} & \textcolor{black!45}{.03/.11} & \textcolor{black!45}{$<$.01/$<$.01} & \textbf{.29/.23} & \textbf{67\%} \\
 &  & \texttt{gpt-5.4-mini} & \textbf{.44/.11} & \textbf{.92/.96} & \textbf{.21/.25} & \textbf{.47/.23} & \textbf{.41/.70} & \textcolor{black!45}{.22/.04} & \textbf{.76/.82} & \textbf{.06/.09} & \textcolor{black!45}{$<$.01/$<$.01} & \textcolor{black!45}{.02/.08} & \textcolor{black!45}{.05/.16} & \textbf{.34/.16} & \textbf{79\%} \\
 &  & \texttt{gpt-4o-mini} & \textcolor{black!45}{.01/$<$.01} & \textcolor{black!45}{$<$.01/$<$.01} & \textcolor{black!45}{$<$.01/$<$.01} & \textbf{.42/.26} & \textbf{.41/.67} & \textcolor{black!45}{$<$.01/$<$.01} & \textcolor{black!45}{$<$.01/.04} & \textcolor{black!45}{$<$.01/$<$.01} & \textcolor{black!45}{$<$.01/$<$.01} & \textbf{.27/.36} & \textcolor{black!45}{$<$.01/$<$.01} & \textcolor{black!45}{.01/.02} & \textcolor{black!55}{25\%} \\
\midrule
\multirow{10}{*}{\rotatebox{90}{\textbf{Movies}}} & \multirow{3}{*}{OASIS} & \texttt{DeepSeek-V4.1-Flash} & \textcolor{black!45}{$<$.01/$<$.01} & \textcolor{black!45}{$<$.01/$<$.01} & \textcolor{black!45}{$<$.01/$<$.01} & \textcolor{black!45}{$<$.01/$<$.01} & \textcolor{black!45}{$<$.01/$<$.01} & \textcolor{black!45}{$<$.01/$<$.01} & \textbf{.12/.13} & \textcolor{black!45}{$<$.01/$<$.01} & \textcolor{black!45}{$<$.01/$<$.01} & \textcolor{black!45}{$<$.01/$<$.01} & \textbf{.34/.70} & \textcolor{black!45}{.02/.07} & \textcolor{black!55}{21\%} \\
 &  & \texttt{gpt-5.4-mini} & \textcolor{black!45}{$<$.01/$<$.01} & \textcolor{black!45}{$<$.01/$<$.01} & \textcolor{black!45}{$<$.01/$<$.01} & \textcolor{black!45}{$<$.01/$<$.01} & \textcolor{black!45}{$<$.01/$<$.01} & \textcolor{black!45}{$<$.01/$<$.01} & \textcolor{black!45}{$<$.01/$<$.01} & \textcolor{black!45}{$<$.01/$<$.01} & \textcolor{black!45}{$<$.01/$<$.01} & \textcolor{black!45}{$<$.01/$<$.01} & \textcolor{black!45}{$<$.01/$<$.01} & \textcolor{black!45}{.02/$<$.01} & \textcolor{black!55}{0\%} \\
 &  & \texttt{gpt-4o-mini} & \textcolor{black!45}{$<$.01/$<$.01} & \textcolor{black!45}{$<$.01/$<$.01} & \textcolor{black!45}{$<$.01/$<$.01} & \textcolor{black!45}{$<$.01/$<$.01} & \textcolor{black!45}{$<$.01/$<$.01} & \textcolor{black!45}{$<$.01/$<$.01} & \textcolor{black!45}{$<$.01/$<$.01} & \textcolor{black!45}{$<$.01/$<$.01} & \textcolor{black!45}{$<$.01/$<$.01} & \textcolor{black!45}{$<$.01/$<$.01} & \textcolor{black!45}{$<$.01/$<$.01} & \textcolor{black!45}{.08/$<$.01} & \textcolor{black!55}{4\%} \\
\cmidrule(l){2-16}
 & \multirow{4}{*}{SynthPAI} & \texttt{DeepSeek-V4.1-Flash} & \textcolor{black!45}{$<$.01/$<$.01} & \textcolor{black!45}{$<$.01/$<$.01} & \textcolor{black!45}{.03/.04} & \textcolor{black!45}{$<$.01/$<$.01} & \textcolor{black!45}{$<$.01/$<$.01} & \textcolor{black!45}{$<$.01/$<$.01} & \textcolor{black!45}{$<$.01/$<$.01} & \textbf{.55/.72} & \textcolor{black!45}{$<$.01/$<$.01} & \textcolor{black!45}{$<$.01/$<$.01} & \textcolor{black!45}{$<$.01/$<$.01} & \textcolor{black!45}{$<$.01/$<$.01} & \textcolor{black!55}{8\%} \\
 &  & \texttt{gpt-5.4-mini} & \textcolor{black!45}{$<$.01/$<$.01} & \textcolor{black!45}{$<$.01/$<$.01} & \textbf{.07/.17} & \textcolor{black!45}{$<$.01/$<$.01} & \textcolor{black!45}{$<$.01/$<$.01} & \textcolor{black!45}{.01/$<$.01} & \textcolor{black!45}{.04/.13} & \textcolor{black!45}{$<$.01/$<$.01} & \textcolor{black!45}{$<$.01/$<$.01} & \textcolor{black!45}{$<$.01/$<$.01} & \textcolor{black!45}{$<$.01/$<$.01} & \textcolor{black!45}{$<$.01/$<$.01} & \textcolor{black!55}{12\%} \\
 &  & \texttt{gpt-4o-mini} & \textcolor{black!45}{$<$.01/$<$.01} & \textcolor{black!45}{$<$.01/$<$.01} & \textcolor{black!45}{$<$.01/$<$.01} & \textcolor{black!45}{$<$.01/$<$.01} & \textcolor{black!45}{.08/$<$.01} & \textcolor{black!45}{$<$.01/$<$.01} & \textcolor{black!45}{$<$.01/$<$.01} & \textcolor{black!45}{.02/.06} & \textcolor{black!45}{$<$.01/$<$.01} & \textcolor{black!45}{$<$.01/$<$.01} & \textcolor{black!45}{$<$.01/$<$.01} & \textcolor{black!45}{$<$.01/$<$.01} & \textcolor{black!55}{8\%} \\
 &  & \texttt{Gemini-2.5-Flash} & \textcolor{black!45}{$<$.01/$<$.01} & \textcolor{black!45}{$<$.01/$<$.01} & \textcolor{black!45}{$<$.01/$<$.01} & \textcolor{black!45}{$<$.01/$<$.01} & \textcolor{black!45}{$<$.01/$<$.01} & \textcolor{black!45}{$<$.01/$<$.01} & \textcolor{black!45}{$<$.01/$<$.01} & \textcolor{black!45}{.11/.03} & \textcolor{black!45}{$<$.01/$<$.01} & \textcolor{black!45}{$<$.01/$<$.01} & \textcolor{black!45}{$<$.01/$<$.01} & \textcolor{black!45}{$<$.01/$<$.01} & \textcolor{black!55}{4\%} \\
\cmidrule(l){2-16}
 & \multirow{3}{*}{\textbf{ThreadPDG}} & \texttt{DeepSeek-V4.1-Flash} & \textbf{.97/.42} & \textbf{.78/.70} & \textbf{.82/.88} & \textbf{.72/.61} & \textbf{.28/.36} & \textcolor{black!45}{$<$.01/$<$.01} & \textbf{.47/.56} & \textbf{.80/.96} & \textbf{.58/.47} & \textbf{.77/.94} & \textcolor{black!45}{.02/.09} & \textbf{.36/.13} & \textbf{88\%} \\
 &  & \texttt{gpt-5.4-mini} & \textbf{.13/.08} & \textbf{.31/.64} & \textbf{.38/.38} & \textbf{.61/.34} & \textbf{.19/.25} & \textbf{.07/.05} & \textbf{.67/.65} & \textbf{.73/.76} & \textcolor{black!45}{.01/.01} & \textbf{.33/.37} & \textbf{.09/.15} & \textbf{.50/.11} & \textbf{92\%} \\
 &  & \texttt{gpt-4o-mini} & \textcolor{black!45}{$<$.01/$<$.01} & \textcolor{black!45}{$<$.01/$<$.01} & \textcolor{black!45}{$<$.01/$<$.01} & \textbf{.43/.36} & \textcolor{black!45}{.05/.14} & \textcolor{black!45}{.03/.04} & \textbf{.30/.15} & \textcolor{black!45}{$<$.01/.04} & \textcolor{black!45}{$<$.01/$<$.01} & \textcolor{black!45}{$<$.01/$<$.01} & \textbf{.08/.15} & \textcolor{black!45}{$<$.01/$<$.01} & \textcolor{black!55}{29\%} \\
\midrule
\multirow{10}{*}{\rotatebox{90}{\textbf{News}}} & \multirow{3}{*}{OASIS} & \texttt{DeepSeek-V4.1-Flash} & \textcolor{black!45}{$<$.01/$<$.01} & \textcolor{black!45}{$<$.01/$<$.01} & \textcolor{black!45}{$<$.01/$<$.01} & \textcolor{black!45}{$<$.01/$<$.01} & \textcolor{black!45}{$<$.01/$<$.01} & \textcolor{black!45}{$<$.01/$<$.01} & \textcolor{black!45}{$<$.01/$<$.01} & \textcolor{black!45}{$<$.01/$<$.01} & \textcolor{black!45}{$<$.01/$<$.01} & \textcolor{black!45}{$<$.01/$<$.01} & \textcolor{black!45}{.43/$<$.01} & \textbf{.50/.09} & \textcolor{black!55}{12\%} \\
 &  & \texttt{gpt-5.4-mini} & \textcolor{black!45}{$<$.01/$<$.01} & \textcolor{black!45}{$<$.01/$<$.01} & \textcolor{black!45}{$<$.01/$<$.01} & \textcolor{black!45}{$<$.01/$<$.01} & \textcolor{black!45}{$<$.01/$<$.01} & \textcolor{black!45}{$<$.01/$<$.01} & \textcolor{black!45}{$<$.01/$<$.01} & \textcolor{black!45}{$<$.01/$<$.01} & \textcolor{black!45}{$<$.01/$<$.01} & \textcolor{black!45}{$<$.01/$<$.01} & \textcolor{black!45}{$<$.01/$<$.01} & \textcolor{black!45}{$<$.01/$<$.01} & \textcolor{black!55}{0\%} \\
 &  & \texttt{gpt-4o-mini} & \textcolor{black!45}{$<$.01/$<$.01} & \textcolor{black!45}{$<$.01/$<$.01} & \textcolor{black!45}{$<$.01/$<$.01} & \textcolor{black!45}{$<$.01/$<$.01} & \textcolor{black!45}{$<$.01/$<$.01} & \textcolor{black!45}{$<$.01/$<$.01} & \textcolor{black!45}{$<$.01/$<$.01} & \textcolor{black!45}{$<$.01/$<$.01} & \textcolor{black!45}{$<$.01/$<$.01} & \textcolor{black!45}{$<$.01/$<$.01} & \textcolor{black!45}{$<$.01/$<$.01} & \textcolor{black!45}{.02/$<$.01} & \textcolor{black!55}{0\%} \\
\cmidrule(l){2-16}
 & \multirow{4}{*}{SynthPAI} & \texttt{DeepSeek-V4.1-Flash} & \textcolor{black!45}{$<$.01/$<$.01} & \textcolor{black!45}{$<$.01/$<$.01} & \textcolor{black!45}{$<$.01/$<$.01} & \textcolor{black!45}{$<$.01/$<$.01} & \textcolor{black!45}{$<$.01/$<$.01} & \textcolor{black!45}{$<$.01/$<$.01} & \textcolor{black!45}{$<$.01/$<$.01} & \textcolor{black!45}{$<$.01/$<$.01} & \textcolor{black!45}{$<$.01/$<$.01} & \textcolor{black!45}{$<$.01/$<$.01} & \textcolor{black!45}{$<$.01/$<$.01} & \textcolor{black!45}{$<$.01/$<$.01} & \textcolor{black!55}{0\%} \\
 &  & \texttt{gpt-5.4-mini} & \textcolor{black!45}{$<$.01/$<$.01} & \textcolor{black!45}{$<$.01/$<$.01} & \textcolor{black!45}{.03/$<$.01} & \textcolor{black!45}{$<$.01/$<$.01} & \textcolor{black!45}{$<$.01/$<$.01} & \textcolor{black!45}{$<$.01/$<$.01} & \textcolor{black!45}{.01/.05} & \textcolor{black!45}{$<$.01/$<$.01} & \textcolor{black!45}{$<$.01/$<$.01} & \textcolor{black!45}{$<$.01/$<$.01} & \textcolor{black!45}{$<$.01/$<$.01} & \textcolor{black!45}{.05/.02} & \textcolor{black!55}{8\%} \\
 &  & \texttt{gpt-4o-mini} & \textcolor{black!45}{$<$.01/$<$.01} & \textcolor{black!45}{$<$.01/$<$.01} & \textcolor{black!45}{$<$.01/$<$.01} & \textcolor{black!45}{$<$.01/$<$.01} & \textbf{.44/.37} & \textcolor{black!45}{$<$.01/$<$.01} & \textcolor{black!45}{$<$.01/$<$.01} & \textbf{.46/.54} & \textcolor{black!45}{$<$.01/$<$.01} & \textcolor{black!45}{$<$.01/$<$.01} & \textcolor{black!45}{$<$.01/$<$.01} & \textcolor{black!45}{$<$.01/$<$.01} & \textcolor{black!55}{17\%} \\
 &  & \texttt{Gemini-2.5-Flash} & \textcolor{black!45}{$<$.01/$<$.01} & \textcolor{black!45}{$<$.01/$<$.01} & \textcolor{black!45}{$<$.01/$<$.01} & \textcolor{black!45}{$<$.01/$<$.01} & \textcolor{black!45}{$<$.01/$<$.01} & \textcolor{black!45}{$<$.01/$<$.01} & \textcolor{black!45}{$<$.01/$<$.01} & \textcolor{black!45}{$<$.01/$<$.01} & \textcolor{black!45}{$<$.01/$<$.01} & \textcolor{black!45}{$<$.01/$<$.01} & \textcolor{black!45}{$<$.01/$<$.01} & \textcolor{black!45}{$<$.01/$<$.01} & \textcolor{black!55}{0\%} \\
\cmidrule(l){2-16}
 & \multirow{3}{*}{\textbf{ThreadPDG}} & \texttt{DeepSeek-V4.1-Flash} & \textbf{.13/.16} & \textbf{.63/.74} & \textcolor{black!45}{.01/.02} & \textbf{.38/.36} & \textbf{.78/.29} & \textcolor{black!45}{$<$.01/$<$.01} & \textbf{.14/.19} & \textbf{.55/.83} & \textbf{.09/.07} & \textcolor{black!45}{.02/.07} & \textcolor{black!45}{$<$.01/$<$.01} & \textcolor{black!45}{.01/$<$.01} & \textbf{62\%} \\
 &  & \texttt{gpt-5.4-mini} & \textbf{.42/.65} & \textbf{.20/.38} & \textbf{.35/.53} & \textbf{.57/.59} & \textbf{.99/.57} & \textbf{.45/.57} & \textbf{.92/1.0} & \textbf{.21/.20} & \textcolor{black!45}{$<$.01/$<$.01} & \textcolor{black!45}{$<$.01/.03} & \textcolor{black!45}{$<$.01/$<$.01} & \textbf{.12/.06} & \textbf{75\%} \\
 &  & \texttt{gpt-4o-mini} & \textcolor{black!45}{$<$.01/$<$.01} & \textcolor{black!45}{$<$.01/$<$.01} & \textcolor{black!45}{$<$.01/$<$.01} & \textbf{.45/.66} & \textbf{.94/.54} & \textcolor{black!45}{$<$.01/$<$.01} & \textbf{.69/.91} & \textcolor{black!45}{$<$.01/$<$.01} & \textcolor{black!45}{$<$.01/$<$.01} & \textcolor{black!45}{$<$.01/$<$.01} & \textbf{.54/.45} & \textcolor{black!45}{$<$.01/$<$.01} & \textcolor{black!55}{33\%} \\
\midrule
\multirow{10}{*}{\rotatebox{90}{\textbf{TV Series}}} & \multirow{3}{*}{OASIS} & \texttt{DeepSeek-V4.1-Flash} & \textcolor{black!45}{$<$.01/$<$.01} & \textcolor{black!45}{$<$.01/$<$.01} & \textcolor{black!45}{$<$.01/$<$.01} & \textcolor{black!45}{$<$.01/$<$.01} & \textcolor{black!45}{$<$.01/$<$.01} & \textcolor{black!45}{$<$.01/$<$.01} & \textcolor{black!45}{$<$.01/$<$.01} & \textcolor{black!45}{$<$.01/$<$.01} & \textcolor{black!45}{$<$.01/$<$.01} & \textcolor{black!45}{$<$.01/$<$.01} & \textbf{.09/.33} & \textbf{.83/.82} & \textcolor{black!55}{17\%} \\
 &  & \texttt{gpt-5.4-mini} & \textcolor{black!45}{$<$.01/$<$.01} & \textcolor{black!45}{$<$.01/$<$.01} & \textcolor{black!45}{$<$.01/$<$.01} & \textcolor{black!45}{$<$.01/$<$.01} & \textcolor{black!45}{$<$.01/$<$.01} & \textcolor{black!45}{$<$.01/$<$.01} & \textcolor{black!45}{$<$.01/$<$.01} & \textcolor{black!45}{$<$.01/$<$.01} & \textcolor{black!45}{$<$.01/$<$.01} & \textcolor{black!45}{$<$.01/$<$.01} & \textcolor{black!45}{$<$.01/$<$.01} & \textcolor{black!45}{$<$.01/$<$.01} & \textcolor{black!55}{0\%} \\
 &  & \texttt{gpt-4o-mini} & \textcolor{black!45}{$<$.01/$<$.01} & \textcolor{black!45}{$<$.01/$<$.01} & \textcolor{black!45}{$<$.01/$<$.01} & \textcolor{black!45}{$<$.01/$<$.01} & \textcolor{black!45}{$<$.01/$<$.01} & \textcolor{black!45}{$<$.01/$<$.01} & \textcolor{black!45}{$<$.01/$<$.01} & \textcolor{black!45}{$<$.01/$<$.01} & \textcolor{black!45}{$<$.01/$<$.01} & \textcolor{black!45}{$<$.01/$<$.01} & \textcolor{black!45}{$<$.01/$<$.01} & \textcolor{black!45}{$<$.01/$<$.01} & \textcolor{black!55}{0\%} \\
\cmidrule(l){2-16}
 & \multirow{4}{*}{SynthPAI} & \texttt{DeepSeek-V4.1-Flash} & \textcolor{black!45}{$<$.01/$<$.01} & \textcolor{black!45}{$<$.01/$<$.01} & \textcolor{black!45}{$<$.01/$<$.01} & \textcolor{black!45}{$<$.01/$<$.01} & \textcolor{black!45}{$<$.01/$<$.01} & \textcolor{black!45}{$<$.01/$<$.01} & \textcolor{black!45}{$<$.01/$<$.01} & \textbf{.87/.09} & \textcolor{black!45}{$<$.01/$<$.01} & \textcolor{black!45}{$<$.01/$<$.01} & \textcolor{black!45}{$<$.01/$<$.01} & \textcolor{black!45}{$<$.01/$<$.01} & \textcolor{black!55}{8\%} \\
 &  & \texttt{gpt-5.4-mini} & \textcolor{black!45}{$<$.01/$<$.01} & \textcolor{black!45}{$<$.01/$<$.01} & \textcolor{black!45}{$<$.01/$<$.01} & \textcolor{black!45}{$<$.01/$<$.01} & \textcolor{black!45}{$<$.01/$<$.01} & \textcolor{black!45}{.07/$<$.01} & \textcolor{black!45}{$<$.01/$<$.01} & \textcolor{black!45}{$<$.01/$<$.01} & \textcolor{black!45}{$<$.01/$<$.01} & \textcolor{black!45}{$<$.01/$<$.01} & \textcolor{black!45}{$<$.01/$<$.01} & \textcolor{black!45}{$<$.01/$<$.01} & \textcolor{black!55}{4\%} \\
 &  & \texttt{gpt-4o-mini} & \textcolor{black!45}{$<$.01/$<$.01} & \textcolor{black!45}{$<$.01/$<$.01} & \textcolor{black!45}{$<$.01/$<$.01} & \textcolor{black!45}{$<$.01/$<$.01} & \textcolor{black!45}{$<$.01/$<$.01} & \textcolor{black!45}{$<$.01/$<$.01} & \textcolor{black!45}{$<$.01/$<$.01} & \textcolor{black!45}{.79/.03} & \textcolor{black!45}{$<$.01/$<$.01} & \textcolor{black!45}{$<$.01/$<$.01} & \textcolor{black!45}{$<$.01/$<$.01} & \textcolor{black!45}{$<$.01/$<$.01} & \textcolor{black!55}{4\%} \\
 &  & \texttt{Gemini-2.5-Flash} & \textcolor{black!45}{.80/$<$.01} & \textcolor{black!45}{$<$.01/$<$.01} & \textcolor{black!45}{$<$.01/$<$.01} & \textcolor{black!45}{$<$.01/$<$.01} & \textcolor{black!45}{$<$.01/$<$.01} & \textcolor{black!45}{$<$.01/$<$.01} & \textcolor{black!45}{$<$.01/$<$.01} & \textbf{.91/.07} & \textcolor{black!45}{$<$.01/$<$.01} & \textcolor{black!45}{$<$.01/$<$.01} & \textcolor{black!45}{$<$.01/$<$.01} & \textcolor{black!45}{$<$.01/$<$.01} & \textcolor{black!55}{12\%} \\
\cmidrule(l){2-16}
 & \multirow{3}{*}{\textbf{ThreadPDG}} & \texttt{DeepSeek-V4.1-Flash} & \textbf{.27/.31} & \textbf{.08/.09} & \textbf{.46/.44} & \textbf{.51/.25} & \textbf{.63/.76} & \textcolor{black!45}{$<$.01/$<$.01} & \textbf{.58/.46} & \textbf{.96/.21} & \textbf{.61/.72} & \textbf{.20/.34} & \textbf{.08/.41} & \textbf{.65/.90} & \textbf{92\%} \\
 &  & \texttt{gpt-5.4-mini} & \textcolor{black!45}{$<$.01/$<$.01} & \textbf{.24/.36} & \textbf{1.0/.70} & \textbf{.46/.35} & \textbf{.58/.74} & \textbf{.06/.16} & \textbf{.74/.77} & \textbf{.38/.06} & \textbf{.19/.14} & \textbf{.43/.30} & \textbf{.70/.86} & \textbf{.26/.42} & \textbf{92\%} \\
 &  & \texttt{gpt-4o-mini} & \textcolor{black!45}{$<$.01/$<$.01} & \textcolor{black!45}{$<$.01/$<$.01} & \textcolor{black!45}{$<$.01/$<$.01} & \textbf{.61/.33} & \textbf{.82/.89} & \textbf{.05/.11} & \textcolor{black!45}{.08/.04} & \textcolor{black!45}{$<$.01/$<$.01} & \textcolor{black!45}{$<$.01/$<$.01} & \textcolor{black!45}{$<$.01/.03} & \textbf{.18/.15} & \textcolor{black!45}{$<$.01/$<$.01} & \textcolor{black!55}{38\%} \\
\bottomrule
\end{tabular}
}
\end{table*}
