# Supplementary material for: ThreadBench: Benchmarking Realism in Agentic Simulation of Real-world Discussions
Source: arXiv:2606.14715 source file (2026-10-10)
Supplement: Supplementary file 3 [file appendix.tex]

\input{sections/reddit_appendix_generated_real}

\section{Broader Impacts}
\label{app:broader_impacts}

MiroBench aims to improve the evaluation of LLM-based social simulation.
It can help researchers measure whether generated discussions match real Reddit discussions beyond surface fluency, and may support safer uses such as testing moderation tools, studying discussion dynamics, and evaluating multi-agent systems.

However, more realistic social simulation also creates risks.
Generated discussions could be misused to create fake engagement, coordinated opinions, or misleading social signals.
Simulations may also reproduce biases in the source data or present simplified versions of human behavior.
For these reasons, MiroBench should be used for evaluation and diagnosis, not for generating deceptive online activity.

Future work should combine automatic metrics with human review, bias analysis, and clear reporting of data sources and simulator settings.
Simulated discussions should be clearly labeled, especially if they are shared or used outside controlled research settings.
\newpage

\section{Limitation and Future work}
\label{app:limitations}

MiroBench provides a focused benchmark for evaluating Reddit discussion simulation, but it has several limitations.
First, the current benchmark covers five product-related Reddit domains.
These domains provide a controlled setting for comparing real and generated discussions, but they do not cover all types of online communities.
Future work can extend MiroBench to broader domains, such as politics, health, education, entertainment, and local communities.

Second, our metrics focus on observable discussion patterns, including repetition, semantic uniformity, storyness, toxicity, aggression, and thread structure.
These metrics capture important differences between real and generated discussions, but they do not fully measure factual correctness, user intent, persuasion, long-term community dynamics, or social influence.
Future work can add task-specific metrics and human evaluation to better understand these aspects.

Third, our calibration study only explores prompt-level changes.
This makes the method lightweight and easy to apply, but it also limits how much the simulator can improve.
Future work can study stronger calibration methods, such as persona distribution learning, automatic prompt optimization, retrieval-based grounding, or fine-tuning on real discussion patterns.

Finally, MiroBench evaluates generated discussions against historical Reddit data.
This is useful for measuring distributional realism, but it does not guarantee that a simulator will behave realistically in live or changing online environments.
Future work can evaluate simulators under temporal shifts, new product releases, and interactive feedback from real users.

\newpage

\newpage
\section{Repeated-Sampling Real-vs.-Real p-Value Counts}
\label{app:repeated_pvalues}
For each domain and metric, we repeatedly split the real threads into a sample of 10 threads and the remaining real threads, and compared the two subsets 200 times. Across all domains and core metrics in this study, the Mann--Whitney U p-value exceeded 0.05 in 95.2\% of repeats on average, and the Kolmogorov--Smirnov p-value exceeded 0.05 in 95.2\% of repeats on average. Because same-domain real-vs.-real comparisons should mostly fail to reject, these counts provide an empirical sanity check that the benchmark strata are internally coherent and that average type-I error stays close to the conventional 5\% testing threshold. This appendix reports the per-domain counts referenced in Section~\ref{sec:scoring}.

\subsection{Camera}
\begin{table}[H]
\centering
\scriptsize
\setlength{\tabcolsep}{4pt}
\renewcommand{\arraystretch}{0.95}
\resizebox{\linewidth}{!}{%
\begin{tabular}{lcccc}
\toprule
Metric & Med. MWU $p$ & MWU $p \geq 0.05$ & Med. KS $p$ & KS $p \geq 0.05$\\
\midrule
\texttt{self\_bleu\_4} & 0.517 & 193/200 (96.5\%) & 0.545 & 190/200 (95.0\%)\\
\texttt{self\_bertscore\_mean\_f1} & 0.584 & 191/200 (95.5\%) & 0.514 & 191/200 (95.5\%)\\
\texttt{semantic\_mean\_cosine} & 0.505 & 195/200 (97.5\%) & 0.553 & 192/200 (96.0\%)\\
\texttt{mean\_story\_probability} & 0.518 & 190/200 (95.0\%) & 0.505 & 190/200 (95.0\%)\\
\texttt{toxicity\_mean} & 0.489 & 192/200 (96.0\%) & 0.506 & 193/200 (96.5\%)\\
\texttt{severe\_toxicity\_mean} & 0.554 & 191/200 (95.5\%) & 0.525 & 188/200 (94.0\%)\\
\texttt{obscene\_mean} & 0.505 & 192/200 (96.0\%) & 0.482 & 192/200 (96.0\%)\\
\texttt{threat\_mean} & 0.467 & 189/200 (94.5\%) & 0.477 & 185/200 (92.5\%)\\
\texttt{aggression\_score\_mean} & 0.477 & 188/200 (94.0\%) & 0.454 & 187/200 (93.5\%)\\
\texttt{length\_std} & 0.476 & 194/200 (97.0\%) & 0.541 & 190/200 (95.0\%)\\
\texttt{length\_cv} & 0.502 & 192/200 (96.0\%) & 0.544 & 194/200 (97.0\%)\\
\texttt{avg\_depth} & 0.488 & 190/200 (95.0\%) & 0.492 & 186/200 (93.0\%)\\
\texttt{structural\_virality} & 0.474 & 190/200 (95.0\%) & 0.566 & 193/200 (96.5\%)\\
\bottomrule
\end{tabular}%
}
\caption{Repeated real-vs.-real p-value counts for the camera domain. Each row uses 200 repeated comparisons between a 10-thread real sample and the remaining same-domain real threads.}
\label{tab:appendix_pvalues_camera}
\end{table}

\subsection{Cellphone}
\begin{table}[H]
\centering
\scriptsize
\setlength{\tabcolsep}{4pt}
\renewcommand{\arraystretch}{0.95}
\resizebox{\linewidth}{!}{%
\begin{tabular}{lcccc}
\toprule
Metric & Med. MWU $p$ & MWU $p \geq 0.05$ & Med. KS $p$ & KS $p \geq 0.05$\\
\midrule
\texttt{self\_bleu\_4} & 0.562 & 194/200 (97.0\%) & 0.572 & 197/200 (98.5\%)\\
\texttt{self\_bertscore\_mean\_f1} & 0.511 & 186/200 (93.0\%) & 0.521 & 186/200 (93.0\%)\\
\texttt{semantic\_mean\_cosine} & 0.525 & 190/200 (95.0\%) & 0.551 & 196/200 (98.0\%)\\
\texttt{mean\_story\_probability} & 0.494 & 192/200 (96.0\%) & 0.508 & 189/200 (94.5\%)\\
\texttt{toxicity\_mean} & 0.537 & 187/200 (93.5\%) & 0.506 & 186/200 (93.0\%)\\
\texttt{severe\_toxicity\_mean} & 0.471 & 190/200 (95.0\%) & 0.512 & 189/200 (94.5\%)\\
\texttt{obscene\_mean} & 0.475 & 192/200 (96.0\%) & 0.501 & 194/200 (97.0\%)\\
\texttt{threat\_mean} & 0.573 & 194/200 (97.0\%) & 0.545 & 190/200 (95.0\%)\\
\texttt{aggression\_score\_mean} & 0.519 & 193/200 (96.5\%) & 0.540 & 192/200 (96.0\%)\\
\texttt{length\_std} & 0.451 & 188/200 (94.0\%) & 0.473 & 191/200 (95.5\%)\\
\texttt{length\_cv} & 0.507 & 193/200 (96.5\%) & 0.502 & 189/200 (94.5\%)\\
\texttt{avg\_depth} & 0.517 & 192/200 (96.0\%) & 0.524 & 196/200 (98.0\%)\\
\texttt{structural\_virality} & 0.484 & 196/200 (98.0\%) & 0.595 & 195/200 (97.5\%)\\
\bottomrule
\end{tabular}%
}
\caption{Repeated real-vs.-real p-value counts for the cellphone domain. Each row uses 200 repeated comparisons between a 10-thread real sample and the remaining same-domain real threads.}
\label{tab:appendix_pvalues_cellphone}
\end{table}

\subsection{Credit Card}
\begin{table}[H]
\centering
\scriptsize
\setlength{\tabcolsep}{4pt}
\renewcommand{\arraystretch}{0.95}
\resizebox{\linewidth}{!}{%
\begin{tabular}{lcccc}
\toprule
Metric & Med. MWU $p$ & MWU $p \geq 0.05$ & Med. KS $p$ & KS $p \geq 0.05$\\
\midrule
\texttt{self\_bleu\_4} & 0.515 & 192/200 (96.0\%) & 0.476 & 194/200 (97.0\%)\\
\texttt{self\_bertscore\_mean\_f1} & 0.505 & 195/200 (97.5\%) & 0.535 & 195/200 (97.5\%)\\
\texttt{semantic\_mean\_cosine} & 0.530 & 191/200 (95.5\%) & 0.471 & 189/200 (94.5\%)\\
\texttt{mean\_story\_probability} & 0.514 & 190/200 (95.0\%) & 0.498 & 194/200 (97.0\%)\\
\texttt{toxicity\_mean} & 0.478 & 190/200 (95.0\%) & 0.424 & 194/200 (97.0\%)\\
\texttt{severe\_toxicity\_mean} & 0.444 & 188/200 (94.0\%) & 0.451 & 187/200 (93.5\%)\\
\texttt{obscene\_mean} & 0.461 & 185/200 (92.5\%) & 0.488 & 188/200 (94.0\%)\\
\texttt{threat\_mean} & 0.450 & 186/200 (93.0\%) & 0.478 & 189/200 (94.5\%)\\
\texttt{aggression\_score\_mean} & 0.459 & 197/200 (98.5\%) & 0.463 & 195/200 (97.5\%)\\
\texttt{length\_std} & 0.525 & 191/200 (95.5\%) & 0.527 & 188/200 (94.0\%)\\
\texttt{length\_cv} & 0.486 & 185/200 (92.5\%) & 0.463 & 188/200 (94.0\%)\\
\texttt{avg\_depth} & 0.536 & 193/200 (96.5\%) & 0.608 & 193/200 (96.5\%)\\
\texttt{structural\_virality} & 0.495 & 191/200 (95.5\%) & 0.574 & 193/200 (96.5\%)\\
\bottomrule
\end{tabular}%
}
\caption{Repeated real-vs.-real p-value counts for the credit card domain. Each row uses 200 repeated comparisons between a 10-thread real sample and the remaining same-domain real threads.}
\label{tab:appendix_pvalues_credit_card}
\end{table}

\subsection{Headphones}
\begin{table}[H]
\centering
\scriptsize
\setlength{\tabcolsep}{4pt}
\renewcommand{\arraystretch}{0.95}
\resizebox{\linewidth}{!}{%
\begin{tabular}{lcccc}
\toprule
Metric & Med. MWU $p$ & MWU $p \geq 0.05$ & Med. KS $p$ & KS $p \geq 0.05$\\
\midrule
\texttt{self\_bleu\_4} & 0.472 & 189/200 (94.5\%) & 0.505 & 188/200 (94.0\%)\\
\texttt{self\_bertscore\_mean\_f1} & 0.495 & 186/200 (93.0\%) & 0.484 & 186/200 (93.0\%)\\
\texttt{semantic\_mean\_cosine} & 0.515 & 196/200 (98.0\%) & 0.500 & 192/200 (96.0\%)\\
\texttt{mean\_story\_probability} & 0.532 & 189/200 (94.5\%) & 0.525 & 191/200 (95.5\%)\\
\texttt{toxicity\_mean} & 0.427 & 183/200 (91.5\%) & 0.426 & 185/200 (92.5\%)\\
\texttt{severe\_toxicity\_mean} & 0.452 & 189/200 (94.5\%) & 0.464 & 192/200 (96.0\%)\\
\texttt{obscene\_mean} & 0.564 & 190/200 (95.0\%) & 0.552 & 190/200 (95.0\%)\\
\texttt{threat\_mean} & 0.537 & 190/200 (95.0\%) & 0.500 & 187/200 (93.5\%)\\
\texttt{aggression\_score\_mean} & 0.455 & 188/200 (94.0\%) & 0.475 & 183/200 (91.5\%)\\
\texttt{length\_std} & 0.484 & 190/200 (95.0\%) & 0.475 & 186/200 (93.0\%)\\
\texttt{length\_cv} & 0.510 & 185/200 (92.5\%) & 0.520 & 188/200 (94.0\%)\\
\texttt{avg\_depth} & 0.479 & 189/200 (94.5\%) & 0.557 & 192/200 (96.0\%)\\
\texttt{structural\_virality} & 0.476 & 195/200 (97.5\%) & 0.605 & 198/200 (99.0\%)\\
\bottomrule
\end{tabular}%
}
\caption{Repeated real-vs.-real p-value counts for the headphones domain. Each row uses 200 repeated comparisons between a 10-thread real sample and the remaining same-domain real threads.}
\label{tab:appendix_pvalues_headphones}
\end{table}

\subsection{Laptop}
\begin{table}[H]
\centering
\scriptsize
\setlength{\tabcolsep}{4pt}
\renewcommand{\arraystretch}{0.95}
\resizebox{\linewidth}{!}{%
\begin{tabular}{lcccc}
\toprule
Metric & Med. MWU $p$ & MWU $p \geq 0.05$ & Med. KS $p$ & KS $p \geq 0.05$\\
\midrule
\texttt{self\_bleu\_4} & 0.545 & 194/200 (97.0\%) & 0.571 & 195/200 (97.5\%)\\
\texttt{self\_bertscore\_mean\_f1} & 0.467 & 190/200 (95.0\%) & 0.497 & 190/200 (95.0\%)\\
\texttt{semantic\_mean\_cosine} & 0.527 & 187/200 (93.5\%) & 0.489 & 182/200 (91.0\%)\\
\texttt{mean\_story\_probability} & 0.513 & 191/200 (95.5\%) & 0.510 & 191/200 (95.5\%)\\
\texttt{toxicity\_mean} & 0.479 & 188/200 (94.0\%) & 0.532 & 186/200 (93.0\%)\\
\texttt{severe\_toxicity\_mean} & 0.538 & 188/200 (94.0\%) & 0.536 & 190/200 (95.0\%)\\
\texttt{obscene\_mean} & 0.545 & 189/200 (94.5\%) & 0.571 & 193/200 (96.5\%)\\
\texttt{threat\_mean} & 0.492 & 194/200 (97.0\%) & 0.562 & 191/200 (95.5\%)\\
\texttt{aggression\_score\_mean} & 0.475 & 188/200 (94.0\%) & 0.489 & 188/200 (94.0\%)\\
\texttt{length\_std} & 0.449 & 187/200 (93.5\%) & 0.485 & 187/200 (93.5\%)\\
\texttt{length\_cv} & 0.507 & 189/200 (94.5\%) & 0.514 & 190/200 (95.0\%)\\
\texttt{avg\_depth} & 0.507 & 194/200 (97.0\%) & 0.638 & 189/200 (94.5\%)\\
\texttt{structural\_virality} & 0.514 & 193/200 (96.5\%) & 0.616 & 192/200 (96.0\%)\\
\bottomrule
\end{tabular}%
}
\caption{Repeated real-vs.-real p-value counts for the laptop domain. Each row uses 200 repeated comparisons between a 10-thread real sample and the remaining same-domain real threads.}
\label{tab:appendix_pvalues_laptop}
\end{table}

\subsection{Metric-Level Real-vs.-Real Distance Statistics}
\label{app:repeated_distance_stats}
We also summarize the repeated real-vs.-real distance statistics computed from the same 200 resampling runs. Table~\ref{tab:appendix_distance_stats} averages each statistic over the five benchmark domains for each of the 13 core metrics. Because Wasserstein distance, quantile error, and absolute median gap are metric-scale dependent, these values should be interpreted within each metric rather than compared directly across unrelated metrics.

\begin{table}[H]
\centering
\scriptsize
\setlength{\tabcolsep}{4pt}
\renewcommand{\arraystretch}{0.92}
\resizebox{\linewidth}{!}{%
\begin{tabular}{lccccc}
\toprule
Metric & Mean $W_1$ & Mean quant. err. & Mean emp. fail & Mean abs. med. gap & Mean $|\delta_{\mathrm{Cliff}}|$\\
\midrule
\texttt{aggression\_score\_mean} & 0.0048 & 0.0035 & 0.0356 & 0.0022 & 0.1358\\
\texttt{avg\_depth} & 0.2425 & 0.2264 & 0.0380 & 0.2202 & 0.1304\\
\texttt{length\_cv} & 0.1295 & 0.1325 & 0.0271 & 0.0842 & 0.1332\\
\texttt{length\_std} & 10.1269 & 8.1864 & 0.0352 & 5.5420 & 0.1374\\
\texttt{mean\_story\_probability} & 0.0468 & 0.0422 & 0.0401 & 0.0388 & 0.1319\\
\texttt{obscene\_mean} & 0.0090 & 0.0064 & 0.0364 & 0.0014 & 0.1350\\
\texttt{self\_bertscore\_mean\_f1} & 0.0381 & 0.0436 & 0.0168 & 0.0072 & 0.1298\\
\texttt{self\_bleu\_4} & 0.0085 & 0.0066 & 0.0332 & 0.0034 & 0.1378\\
\texttt{semantic\_mean\_cosine} & 0.0442 & 0.0455 & 0.0328 & 0.0268 & 0.1266\\
\texttt{severe\_toxicity\_mean} & 0.0001 & 0.0001 & 0.0390 & 0.0000 & 0.1361\\
\texttt{structural\_virality} & 0.3861 & 0.3931 & 0.0353 & 0.2919 & 0.1297\\
\texttt{threat\_mean} & 0.0008 & 0.0003 & 0.0402 & 0.0000 & 0.1353\\
\texttt{toxicity\_mean} & 0.0142 & 0.0103 & 0.0355 & 0.0070 & 0.1359\\
\bottomrule
\end{tabular}%
}
\caption{Repeated real-vs.-real distance statistics averaged over the five benchmark domains for each core metric. Values are aggregated from the 200 repeated within-domain resampling comparisons used in the benchmark stability analysis.}
\label{tab:appendix_distance_stats}
\end{table}

\section{Unified OASIS Baseline Table}
\label{app:oasis_unified_baseline_table}
Section~\ref{sec:results} focuses on Mann--Whitney U and Kolmogorov--Smirnov $p$-values in the main paper. For completeness, this appendix reports the full unified baseline comparison across all five domains, all five currently evaluated models, and the 13 core metrics. Table~\ref{tab:appendix_oasis_baseline_full} adds Wasserstein distance, quantile error, empirical fail rate, and absolute Cliff's delta together with the same-domain repeated real-vs.-real reference values used for calibration.

\input{sections/appendix_unified_baseline_table}

\section{Per-Metric OASIS Baseline Comparisons}
\label{app:oasis_baseline_metric_tables}
Section~\ref{sec:results} summarizes the main p-value results, while Table~\ref{tab:appendix_oasis_baseline_full} provides the unified comparison across domains, models, and metrics. This section provides per-domain baseline tables for the GPT-family runs together with the same repeated real-vs.-real references used throughout the benchmark. For each domain, the tables compare GPT-4o-mini and GPT-5-mini against held-out real threads using MWU and KS $p$-values together with Wasserstein distance, quantile error, empirical fail rate, and absolute Cliff's delta. The final comparison block in each table reports the same-domain median real-vs.-real repeated-sample reference used to calibrate whether a baseline is still far from natural within-domain variation.

\subsection{Laptop}
\begin{table}[H]
\centering
\scriptsize
\setlength{\tabcolsep}{4pt}
\renewcommand{\arraystretch}{0.92}
\resizebox{\linewidth}{!}{%
\begin{tabular}{lcccccc}
\toprule
Metric & \multicolumn{2}{c}{GPT-4o-mini} & \multicolumn{2}{c}{GPT-5-mini} & \multicolumn{2}{c}{Repeated real-vs.-real}\\
\cmidrule(lr){2-3}\cmidrule(lr){4-5}\cmidrule(lr){6-7}
& MWU $p$ & KS $p$ & MWU $p$ & KS $p$ & Med. MWU $p$ & Med. KS $p$\\
\midrule
\texttt{self\_bleu\_4} & 1.9e-16 & 3.2e-31 & 6.1e-08 & 2.5e-11 & 0.516 & 0.710\\
\texttt{self\_bertscore\_mean\_f1} & 6.5e-17 & 1.4e-34 & 3.0e-09 & 2.4e-17 & 0.491 & 0.593\\
\texttt{semantic\_mean\_cosine} & 4.3e-17 & 1.4e-34 & 1.3e-10 & 4.6e-17 & 0.567 & 0.710\\
\texttt{mean\_story\_probability} & 3.4e-22 & 7.2e-24 & 3.8e-14 & 1.7e-16 & 0.516 & 0.710\\
\texttt{toxicity\_mean} & 1.9e-11 & 1.8e-11 & 0.707 & 0.024 & 0.441 & 0.475\\
\texttt{severe\_toxicity\_mean} & 1.2e-16 & 1.5e-18 & 0.377 & 0.042 & 0.516 & 0.710\\
\texttt{obscene\_mean} & 1.2e-10 & 1.6e-10 & 0.253 & 0.008 & 0.467 & 0.710\\
\texttt{threat\_mean} & 1.8e-17 & 7.5e-19 & 0.786 & 0.171 & 0.528 & 0.710\\
\texttt{aggression\_score\_mean} & 2.4e-11 & 1.4e-11 & 0.691 & 0.014 & 0.557 & 0.710\\
\texttt{length\_std} & 2.0e-08 & 1.6e-17 & 7.6e-04 & 8.2e-05 & 0.566 & 0.710\\
\texttt{length\_cv} & 3.4e-17 & 8.1e-33 & 1.0e-06 & 8.3e-09 & 0.482 & 0.710\\
\texttt{avg\_depth} & 1.0e-20 & 2.6e-28 & 7.0e-15 & 5.9e-16 & 0.471 & 0.710\\
\texttt{structural\_virality} & 4.6e-20 & 2.6e-28 & 1.3e-15 & 5.9e-16 & 0.452 & 0.710\\
\bottomrule
\end{tabular}%
}
\caption{Per-metric significance comparison for the laptop domain. Lower baseline $p$-values indicate that generated and held-out real threads remain easier to distinguish. The final block gives the same-domain median real-vs.-real repeated-sample reference from the 200 within-domain resampling runs.}
\label{tab:appendix_oasis_laptop_pvalues}
\end{table}

\begin{table}[H]
\centering
\scriptsize
\setlength{\tabcolsep}{4pt}
\renewcommand{\arraystretch}{0.92}
\resizebox{\linewidth}{!}{%
\begin{tabular}{lcccccccccccc}
\toprule
Metric & \multicolumn{4}{c}{GPT-4o-mini} & \multicolumn{4}{c}{GPT-5-mini} & \multicolumn{4}{c}{Repeated real-vs.-real}\\
\cmidrule(lr){2-5}\cmidrule(lr){6-9}\cmidrule(lr){10-13}
& $W_1$ & Quant. err. & Emp. fail & $|\delta_{\mathrm{Cliff}}|$ & $W_1$ & Quant. err. & Emp. fail & $|\delta_{\mathrm{Cliff}}|$ & Med. $W_1$ & Med. quant. err. & Med. emp. fail & Med. $|\delta_{\mathrm{Cliff}}|$\\
\midrule
\texttt{self\_bleu\_4} & 0.1096 & 0.1076 & 0.8431 & 0.7252 & 0.0424 & 0.0453 & 0.5088 & 0.6348 & 0.0088 & 0.0073 & 0.0e+00 & 0.1328\\
\texttt{self\_bertscore\_mean\_f1} & 0.2140 & 0.1903 & 0.8627 & 0.7367 & 0.1486 & 0.2074 & 0.8246 & 0.6952 & 0.0399 & 0.0563 & 0.0e+00 & 0.1216\\
\texttt{semantic\_mean\_cosine} & 0.4816 & 0.4461 & 0.8627 & 0.7411 & 0.3419 & 0.3449 & 0.8421 & 0.7532 & 0.0453 & 0.0479 & 0.0e+00 & 0.1184\\
\texttt{mean\_story\_probability} & 0.1720 & 0.1583 & 0.1176 & 0.8548 & 0.1458 & 0.1490 & 0.7895 & 0.8874 & 0.0509 & 0.0418 & 0.0e+00 & 0.1184\\
\texttt{toxicity\_mean} & 0.0240 & 0.0207 & 0.0784 & 0.5926 & 0.0059 & 0.0052 & 0.1053 & 0.0445 & 0.0140 & 0.0102 & 0.0e+00 & 0.1200\\
\texttt{severe\_toxicity\_mean} & 1.3e-04 & 5.1e-05 & 0.1176 & 0.7305 & 6.7e-05 & 6.6e-06 & 0.1053 & 0.1040 & 9.3e-05 & 4.2e-05 & 0.0e+00 & 0.1264\\
\texttt{obscene\_mean} & 0.0126 & 0.0097 & 0.0784 & 0.5688 & 0.0043 & 0.0019 & 0.1053 & 0.1342 & 0.0093 & 0.0059 & 0.0e+00 & 0.1224\\
\texttt{threat\_mean} & 4.1e-04 & 5.4e-05 & 0.1176 & 0.7506 & 6.9e-04 & 1.3e-04 & 0.1053 & 0.0322 & 5.0e-04 & 4.5e-05 & 0.0400 & 0.1200\\
\texttt{aggression\_score\_mean} & 0.0080 & 0.0068 & 0.0784 & 0.5897 & 0.0021 & 0.0016 & 0.1053 & 0.0469 & 0.0048 & 0.0034 & 0.0e+00 & 0.1280\\
\texttt{length\_std} & 18.81 & 17.51 & 0.0e+00 & 0.4946 & 28.65 & 32.06 & 0.0e+00 & 0.3945 & 7.610 & 7.163 & 0.0e+00 & 0.1056\\
\texttt{length\_cv} & 0.5559 & 0.5169 & 0.0e+00 & 0.7433 & 0.2897 & 0.2917 & 0.0e+00 & 0.5724 & 0.1225 & 0.1297 & 0.0e+00 & 0.1096\\
\texttt{avg\_depth} & 0.9650 & 0.8585 & 0.0784 & 0.8103 & 0.9565 & 0.9088 & 0.1579 & 0.8237 & 0.2262 & 0.2078 & 0.0400 & 0.1072\\
\texttt{structural\_virality} & 1.543 & 1.476 & 0.0e+00 & 0.7941 & 1.367 & 1.330 & 0.0e+00 & 0.7907 & 0.3424 & 0.3437 & 0.0e+00 & 0.1120\\
\bottomrule
\end{tabular}%
}
\caption{Per-metric discrepancy comparison for the laptop domain. Lower is better for all reported statistics. The final block gives the same-domain median real-vs.-real repeated-sample reference from the 200 within-domain resampling runs, which serves as the calibration target for judging whether a baseline is still outside normal within-domain variation.}
\label{tab:appendix_oasis_laptop_distances}
\end{table}

\subsection{Credit Card}
\begin{table}[H]
\centering
\scriptsize
\setlength{\tabcolsep}{4pt}
\renewcommand{\arraystretch}{0.92}
\resizebox{\linewidth}{!}{%
\begin{tabular}{lcccccc}
\toprule
Metric & \multicolumn{2}{c}{GPT-4o-mini} & \multicolumn{2}{c}{GPT-5-mini} & \multicolumn{2}{c}{Repeated real-vs.-real}\\
\cmidrule(lr){2-3}\cmidrule(lr){4-5}\cmidrule(lr){6-7}
& MWU $p$ & KS $p$ & MWU $p$ & KS $p$ & Med. MWU $p$ & Med. KS $p$\\
\midrule
\texttt{self\_bleu\_4} & 2.1e-33 & 6.6e-76 & 5.4e-15 & 7.9e-27 & 0.528 & 0.710\\
\texttt{self\_bertscore\_mean\_f1} & 7.3e-34 & 3.4e-105 & 1.2e-13 & 1.1e-25 & 0.525 & 0.710\\
\texttt{semantic\_mean\_cosine} & 7.8e-34 & 1.8e-98 & 1.6e-19 & 1.9e-35 & 0.449 & 0.710\\
\texttt{mean\_story\_probability} & 1.8e-27 & 1.7e-41 & 8.9e-11 & 1.6e-08 & 0.473 & 0.710\\
\texttt{toxicity\_mean} & 4.0e-14 & 1.3e-13 & 0.240 & 0.051 & 0.541 & 0.710\\
\texttt{severe\_toxicity\_mean} & 3.7e-25 & 1.1e-26 & 0.479 & 0.010 & 0.522 & 0.710\\
\texttt{obscene\_mean} & 2.9e-17 & 2.2e-16 & 0.729 & 0.010 & 0.473 & 0.710\\
\texttt{threat\_mean} & 1.7e-18 & 3.7e-21 & 1.9e-05 & 1.2e-04 & 0.528 & 0.710\\
\texttt{aggression\_score\_mean} & 1.1e-13 & 2.3e-13 & 0.260 & 0.058 & 0.509 & 0.710\\
\texttt{length\_std} & 4.5e-17 & 1.1e-29 & 1.8e-09 & 4.4e-14 & 0.506 & 0.710\\
\texttt{length\_cv} & 5.7e-24 & 1.7e-47 & 3.7e-21 & 5.4e-24 & 0.485 & 0.710\\
\texttt{avg\_depth} & 1.1e-23 & 6.4e-37 & 3.0e-31 & 1.9e-44 & 0.559 & 0.710\\
\texttt{structural\_virality} & 9.4e-24 & 6.4e-37 & 1.4e-29 & 1.9e-44 & 0.470 & 0.710\\
\bottomrule
\end{tabular}%
}
\caption{Per-metric significance comparison for the credit card domain. Lower baseline $p$-values indicate that generated and held-out real threads remain easier to distinguish. The final block gives the same-domain median real-vs.-real repeated-sample reference from the 200 within-domain resampling runs.}
\label{tab:appendix_oasis_credit_card_pvalues}
\end{table}

\begin{table}[H]
\centering
\scriptsize
\setlength{\tabcolsep}{4pt}
\renewcommand{\arraystretch}{0.92}
\resizebox{\linewidth}{!}{%
\begin{tabular}{lcccccccccccc}
\toprule
Metric & \multicolumn{4}{c}{GPT-4o-mini} & \multicolumn{4}{c}{GPT-5-mini} & \multicolumn{4}{c}{Repeated real-vs.-real}\\
\cmidrule(lr){2-5}\cmidrule(lr){6-9}\cmidrule(lr){10-13}
& $W_1$ & Quant. err. & Emp. fail & $|\delta_{\mathrm{Cliff}}|$ & $W_1$ & Quant. err. & Emp. fail & $|\delta_{\mathrm{Cliff}}|$ & Med. $W_1$ & Med. quant. err. & Med. emp. fail & Med. $|\delta_{\mathrm{Cliff}}|$\\
\midrule
\texttt{self\_bleu\_4} & 0.1361 & 0.1359 & 1.000 & 0.9928 & 0.0541 & 0.0512 & 0.4143 & 0.5865 & 0.0058 & 0.0047 & 0.0e+00 & 0.1008\\
\texttt{self\_bertscore\_mean\_f1} & 0.2568 & 0.2328 & 1.000 & 1.0000 & 0.1294 & 0.1682 & 0.6714 & 0.5562 & 0.0276 & 0.0148 & 0.0e+00 & 0.1088\\
\texttt{semantic\_mean\_cosine} & 0.5725 & 0.5686 & 1.000 & 0.9995 & 0.3389 & 0.3399 & 0.7857 & 0.6782 & 0.0423 & 0.0417 & 0.0400 & 0.1056\\
\texttt{mean\_story\_probability} & 0.1561 & 0.1490 & 0.3600 & 0.8952 & 0.0938 & 0.0911 & 0.4000 & 0.4865 & 0.0464 & 0.0419 & 0.0400 & 0.1104\\
\texttt{toxicity\_mean} & 0.0181 & 0.0150 & 0.0200 & 0.6234 & 0.0107 & 0.0120 & 0.1286 & 0.0881 & 0.0106 & 0.0082 & 0.0e+00 & 0.1168\\
\texttt{severe\_toxicity\_mean} & 7.6e-05 & 2.7e-05 & 0.4200 & 0.8544 & 7.2e-05 & 4.0e-05 & 0.1286 & 0.0532 & 6.4e-05 & 2.6e-05 & 0.0e+00 & 0.1168\\
\texttt{obscene\_mean} & 0.0097 & 0.0066 & 0.1200 & 0.6967 & 0.0089 & 0.0082 & 0.1000 & 0.0260 & 0.0067 & 0.0047 & 0.0e+00 & 0.1232\\
\texttt{threat\_mean} & 2.7e-04 & 3.7e-05 & 0.1000 & 0.7236 & 1.5e-04 & 2.7e-05 & 0.1714 & 0.3211 & 2.1e-04 & 2.6e-05 & 0.0e+00 & 0.1104\\
\texttt{aggression\_score\_mean} & 0.0060 & 0.0049 & 0.0200 & 0.6122 & 0.0036 & 0.0041 & 0.1143 & 0.0845 & 0.0037 & 0.0028 & 0.0e+00 & 0.1184\\
\texttt{length\_std} & 25.20 & 22.56 & 0.0e+00 & 0.6923 & 40.27 & 39.86 & 0.4714 & 0.4512 & 8.796 & 7.126 & 0.0e+00 & 0.1136\\
\texttt{length\_cv} & 0.5818 & 0.5632 & 0.0e+00 & 0.8324 & 0.4097 & 0.4113 & 0.0e+00 & 0.7083 & 0.1099 & 0.1050 & 0.0e+00 & 0.1120\\
\texttt{avg\_depth} & 0.9406 & 0.9133 & 0.0e+00 & 0.8242 & 1.084 & 1.009 & 0.1714 & 0.8640 & 0.2217 & 0.2014 & 0.0400 & 0.0944\\
\texttt{structural\_virality} & 1.688 & 1.642 & 0.0e+00 & 0.8242 & 1.746 & 1.645 & 0.0e+00 & 0.8359 & 0.3284 & 0.3347 & 0.0e+00 & 0.0984\\
\bottomrule
\end{tabular}%
}
\caption{Per-metric discrepancy comparison for the credit card domain. Lower is better for all reported statistics. The final block gives the same-domain median real-vs.-real repeated-sample reference from the 200 within-domain resampling runs, which serves as the calibration target for judging whether a baseline is still outside normal within-domain variation.}
\label{tab:appendix_oasis_credit_card_distances}
\end{table}

\subsection{Cellphone}
\begin{table}[H]
\centering
\scriptsize
\setlength{\tabcolsep}{4pt}
\renewcommand{\arraystretch}{0.92}
\resizebox{\linewidth}{!}{%
\begin{tabular}{lcccccc}
\toprule
Metric & \multicolumn{2}{c}{GPT-4o-mini} & \multicolumn{2}{c}{GPT-5-mini} & \multicolumn{2}{c}{Repeated real-vs.-real}\\
\cmidrule(lr){2-3}\cmidrule(lr){4-5}\cmidrule(lr){6-7}
& MWU $p$ & KS $p$ & MWU $p$ & KS $p$ & Med. MWU $p$ & Med. KS $p$\\
\midrule
\texttt{self\_bleu\_4} & 2.8e-22 & 6.3e-38 & 4.0e-11 & 8.6e-18 & 0.503 & 0.710\\
\texttt{self\_bertscore\_mean\_f1} & 4.2e-24 & 1.8e-44 & 8.8e-15 & 5.1e-24 & 0.475 & 0.710\\
\texttt{semantic\_mean\_cosine} & 7.9e-25 & 5.3e-48 & 7.4e-16 & 1.5e-26 & 0.482 & 0.475\\
\texttt{mean\_story\_probability} & 1.3e-27 & 1.2e-34 & 9.9e-17 & 2.1e-18 & 0.464 & 0.475\\
\texttt{toxicity\_mean} & 6.5e-26 & 1.7e-34 & 0.002 & 4.1e-04 & 0.516 & 0.710\\
\texttt{severe\_toxicity\_mean} & 3.3e-26 & 2.8e-34 & 0.002 & 6.4e-04 & 0.500 & 0.710\\
\texttt{obscene\_mean} & 2.3e-25 & 1.9e-33 & 0.002 & 3.3e-04 & 0.554 & 0.710\\
\texttt{threat\_mean} & 3.5e-25 & 7.5e-33 & 4.4e-05 & 3.6e-05 & 0.551 & 0.710\\
\texttt{aggression\_score\_mean} & 6.5e-26 & 4.7e-35 & 0.003 & 4.1e-04 & 0.541 & 0.710\\
\texttt{length\_std} & 1.2e-16 & 5.0e-29 & 3.3e-13 & 2.5e-17 & 0.491 & 0.475\\
\texttt{length\_cv} & 3.0e-22 & 1.0e-40 & 2.1e-14 & 2.0e-21 & 0.458 & 0.710\\
\texttt{avg\_depth} & 4.9e-22 & 3.6e-31 & 3.3e-18 & 6.2e-20 & 0.484 & 0.475\\
\texttt{structural\_virality} & 2.4e-21 & 3.6e-31 & 6.7e-19 & 6.2e-20 & 0.498 & 0.710\\
\bottomrule
\end{tabular}%
}
\caption{Per-metric significance comparison for the cellphone domain. Lower baseline $p$-values indicate that generated and held-out real threads remain easier to distinguish. The final block gives the same-domain median real-vs.-real repeated-sample reference from the 200 within-domain resampling runs.}
\label{tab:appendix_oasis_cellphone_pvalues}
\end{table}

\begin{table}[H]
\centering
\scriptsize
\setlength{\tabcolsep}{4pt}
\renewcommand{\arraystretch}{0.92}
\resizebox{\linewidth}{!}{%
\begin{tabular}{lcccccccccccc}
\toprule
Metric & \multicolumn{4}{c}{GPT-4o-mini} & \multicolumn{4}{c}{GPT-5-mini} & \multicolumn{4}{c}{Repeated real-vs.-real}\\
\cmidrule(lr){2-5}\cmidrule(lr){6-9}\cmidrule(lr){10-13}
& $W_1$ & Quant. err. & Emp. fail & $|\delta_{\mathrm{Cliff}}|$ & $W_1$ & Quant. err. & Emp. fail & $|\delta_{\mathrm{Cliff}}|$ & Med. $W_1$ & Med. quant. err. & Med. emp. fail & Med. $|\delta_{\mathrm{Cliff}}|$\\
\midrule
\texttt{self\_bleu\_4} & 0.0698 & 0.0771 & 0.4706 & 0.8353 & 0.0554 & 0.0658 & 0.1493 & 0.7158 & 0.0089 & 0.0069 & 0.0e+00 & 0.1320\\
\texttt{self\_bertscore\_mean\_f1} & 0.1892 & 0.2019 & 0.9412 & 0.8713 & 0.1405 & 0.1575 & 0.9104 & 0.8406 & 0.0385 & 0.0382 & 0.0e+00 & 0.1200\\
\texttt{semantic\_mean\_cosine} & 0.4742 & 0.5058 & 0.9412 & 0.8851 & 0.4511 & 0.4830 & 1.000 & 0.8740 & 0.0389 & 0.0397 & 0.0e+00 & 0.1160\\
\texttt{mean\_story\_probability} & 0.1943 & 0.1878 & 0.7647 & 0.9369 & 0.1430 & 0.1349 & 0.7015 & 0.9003 & 0.0433 & 0.0412 & 0.0e+00 & 0.1120\\
\texttt{toxicity\_mean} & 0.0222 & 0.0211 & 0.2941 & 0.9058 & 0.0253 & 0.0238 & 0.0896 & 0.3284 & 0.0084 & 0.0068 & 0.0e+00 & 0.1136\\
\texttt{severe\_toxicity\_mean} & 8.3e-05 & 3.2e-05 & 0.4706 & 0.9113 & 1.8e-04 & 1.4e-04 & 0.0597 & 0.3397 & 5.1e-05 & 2.3e-05 & 0.0e+00 & 0.1216\\
\texttt{obscene\_mean} & 0.0111 & 0.0104 & 0.3333 & 0.8955 & 0.0203 & 0.0154 & 0.0448 & 0.3415 & 0.0053 & 0.0049 & 0.0e+00 & 0.1144\\
\texttt{threat\_mean} & 2.7e-04 & 8.2e-05 & 0.4314 & 0.8920 & 1.4e-04 & 5.2e-05 & 0.1194 & 0.4430 & 1.4e-04 & 5.8e-05 & 0.0e+00 & 0.1040\\
\texttt{aggression\_score\_mean} & 0.0073 & 0.0068 & 0.2941 & 0.9058 & 0.0088 & 0.0080 & 0.0896 & 0.3212 & 0.0029 & 0.0025 & 0.0e+00 & 0.1168\\
\texttt{length\_std} & 26.51 & 23.73 & 0.0e+00 & 0.7127 & 44.75 & 45.88 & 0.7463 & 0.7893 & 9.183 & 7.239 & 0.0e+00 & 0.1192\\
\texttt{length\_cv} & 0.6811 & 0.6675 & 0.0e+00 & 0.8345 & 0.5006 & 0.5213 & 0.0597 & 0.8287 & 0.1211 & 0.1296 & 0.0e+00 & 0.1136\\
\texttt{avg\_depth} & 0.9221 & 0.8581 & 0.0784 & 0.8213 & 1.223 & 1.195 & 0.0896 & 0.8361 & 0.2115 & 0.2111 & 0.0e+00 & 0.1136\\
\texttt{structural\_virality} & 1.757 & 1.722 & 0.0e+00 & 0.8061 & 2.136 & 2.079 & 0.0e+00 & 0.8200 & 0.3649 & 0.3836 & 0.0e+00 & 0.1104\\
\bottomrule
\end{tabular}%
}
\caption{Per-metric discrepancy comparison for the cellphone domain. Lower is better for all reported statistics. The final block gives the same-domain median real-vs.-real repeated-sample reference from the 200 within-domain resampling runs, which serves as the calibration target for judging whether a baseline is still outside normal within-domain variation.}
\label{tab:appendix_oasis_cellphone_distances}
\end{table}

\subsection{Camera}
\begin{table}[H]
\centering
\scriptsize
\setlength{\tabcolsep}{4pt}
\renewcommand{\arraystretch}{0.92}
\resizebox{\linewidth}{!}{%
\begin{tabular}{lcccccc}
\toprule
Metric & \multicolumn{2}{c}{GPT-4o-mini} & \multicolumn{2}{c}{GPT-5-mini} & \multicolumn{2}{c}{Repeated real-vs.-real}\\
\cmidrule(lr){2-3}\cmidrule(lr){4-5}\cmidrule(lr){6-7}
& MWU $p$ & KS $p$ & MWU $p$ & KS $p$ & Med. MWU $p$ & Med. KS $p$\\
\midrule
\texttt{self\_bleu\_4} & 4.4e-25 & 4.7e-50 & 4.7e-24 & 2.2e-37 & 0.547 & 0.710\\
\texttt{self\_bertscore\_mean\_f1} & 3.9e-25 & 1.0e-47 & 2.9e-25 & 9.9e-47 & 0.485 & 0.475\\
\texttt{semantic\_mean\_cosine} & 1.6e-25 & 1.0e-48 & 2.7e-25 & 9.9e-47 & 0.506 & 0.593\\
\texttt{mean\_story\_probability} & 2.2e-19 & 2.1e-23 & 2.7e-28 & 4.6e-41 & 0.513 & 0.710\\
\texttt{toxicity\_mean} & 9.7e-08 & 1.4e-11 & 3.2e-05 & 2.9e-09 & 0.482 & 0.710\\
\texttt{severe\_toxicity\_mean} & 1.9e-05 & 1.8e-09 & 0.008 & 1.6e-06 & 0.500 & 0.710\\
\texttt{obscene\_mean} & 3.6e-09 & 7.9e-11 & 0.002 & 1.4e-07 & 0.519 & 0.710\\
\texttt{threat\_mean} & 0.642 & 0.096 & 0.005 & 2.9e-04 & 0.473 & 0.593\\
\texttt{aggression\_score\_mean} & 9.6e-08 & 1.1e-11 & 3.7e-05 & 2.9e-09 & 0.577 & 0.710\\
\texttt{length\_std} & 1.3e-21 & 7.9e-36 & 2.7e-07 & 9.4e-09 & 0.509 & 0.593\\
\texttt{length\_cv} & 3.2e-24 & 1.7e-46 & 3.0e-20 & 2.3e-27 & 0.544 & 0.710\\
\texttt{avg\_depth} & 3.6e-24 & 2.6e-37 & 8.3e-25 & 2.6e-37 & 0.462 & 0.475\\
\texttt{structural\_virality} & 7.4e-24 & 2.6e-37 & 7.4e-24 & 2.6e-37 & 0.508 & 0.710\\
\bottomrule
\end{tabular}%
}
\caption{Per-metric significance comparison for the camera domain. Lower baseline $p$-values indicate that generated and held-out real threads remain easier to distinguish. The final block gives the same-domain median real-vs.-real repeated-sample reference from the 200 within-domain resampling runs.}
\label{tab:appendix_oasis_camera_pvalues}
\end{table}

\begin{table}[H]
\centering
\scriptsize
\setlength{\tabcolsep}{4pt}
\renewcommand{\arraystretch}{0.92}
\resizebox{\linewidth}{!}{%
\begin{tabular}{lcccccccccccc}
\toprule
Metric & \multicolumn{4}{c}{GPT-4o-mini} & \multicolumn{4}{c}{GPT-5-mini} & \multicolumn{4}{c}{Repeated real-vs.-real}\\
\cmidrule(lr){2-5}\cmidrule(lr){6-9}\cmidrule(lr){10-13}
& $W_1$ & Quant. err. & Emp. fail & $|\delta_{\mathrm{Cliff}}|$ & $W_1$ & Quant. err. & Emp. fail & $|\delta_{\mathrm{Cliff}}|$ & Med. $W_1$ & Med. quant. err. & Med. emp. fail & Med. $|\delta_{\mathrm{Cliff}}|$\\
\midrule
\texttt{self\_bleu\_4} & 0.0960 & 0.0983 & 0.9400 & 0.8723 & 0.0629 & 0.0634 & 0.8200 & 0.8531 & 0.0058 & 0.0046 & 0.0e+00 & 0.1208\\
\texttt{self\_bertscore\_mean\_f1} & 0.1927 & 0.2030 & 0.9200 & 0.8733 & 0.1262 & 0.1324 & 0.9000 & 0.8757 & 0.0300 & 0.0173 & 0.0e+00 & 0.0880\\
\texttt{semantic\_mean\_cosine} & 0.4872 & 0.5197 & 0.9400 & 0.8806 & 0.4224 & 0.4476 & 0.9200 & 0.8762 & 0.0411 & 0.0410 & 0.0e+00 & 0.0920\\
\texttt{mean\_story\_probability} & 0.1034 & 0.1006 & 0.0600 & 0.7594 & 0.1189 & 0.1095 & 0.5200 & 0.9302 & 0.0300 & 0.0243 & 0.0e+00 & 0.1064\\
\texttt{toxicity\_mean} & 0.0245 & 0.0227 & 0.0400 & 0.4497 & 0.0225 & 0.0220 & 0.0600 & 0.3510 & 0.0110 & 0.0081 & 0.0e+00 & 0.1136\\
\texttt{severe\_toxicity\_mean} & 1.1e-04 & 6.0e-05 & 0.0600 & 0.3609 & 1.1e-04 & 5.9e-05 & 0.0600 & 0.2248 & 7.1e-05 & 3.7e-05 & 0.0200 & 0.1088\\
\texttt{obscene\_mean} & 0.0140 & 0.0116 & 0.0800 & 0.4977 & 0.0124 & 0.0116 & 0.0600 & 0.2646 & 0.0072 & 0.0055 & 0.0e+00 & 0.1144\\
\texttt{threat\_mean} & 8.3e-04 & 4.5e-04 & 0.0600 & 0.0393 & 0.0013 & 6.1e-04 & 0.0600 & 0.2358 & 0.0011 & 4.8e-04 & 0.0e+00 & 0.1144\\
\texttt{aggression\_score\_mean} & 0.0082 & 0.0073 & 0.0400 & 0.4498 & 0.0076 & 0.0071 & 0.0600 & 0.3480 & 0.0038 & 0.0028 & 0.0e+00 & 0.1088\\
\texttt{length\_std} & 36.10 & 33.16 & 0.0e+00 & 0.8052 & 22.69 & 22.08 & 0.0400 & 0.4338 & 11.30 & 9.356 & 0.0e+00 & 0.1296\\
\texttt{length\_cv} & 0.6555 & 0.6532 & 0.0e+00 & 0.8563 & 0.4917 & 0.5062 & 0.0e+00 & 0.7775 & 0.1186 & 0.1145 & 0.0e+00 & 0.1280\\
\texttt{avg\_depth} & 0.9854 & 0.9365 & 0.0400 & 0.8515 & 1.031 & 0.9594 & 0.1200 & 0.8639 & 0.2469 & 0.2245 & 0.0400 & 0.1144\\
\texttt{structural\_virality} & 1.834 & 1.778 & 0.0e+00 & 0.8453 & 1.834 & 1.778 & 0.0e+00 & 0.8453 & 0.3730 & 0.4083 & 0.0400 & 0.1104\\
\bottomrule
\end{tabular}%
}
\caption{Per-metric discrepancy comparison for the camera domain. Lower is better for all reported statistics. The final block gives the same-domain median real-vs.-real repeated-sample reference from the 200 within-domain resampling runs, which serves as the calibration target for judging whether a baseline is still outside normal within-domain variation.}
\label{tab:appendix_oasis_camera_distances}
\end{table}

\subsection{Headphones}
\begin{table}[H]
\centering
\scriptsize
\setlength{\tabcolsep}{4pt}
\renewcommand{\arraystretch}{0.92}
\resizebox{\linewidth}{!}{%
\begin{tabular}{lcccccc}
\toprule
Metric & \multicolumn{2}{c}{GPT-4o-mini} & \multicolumn{2}{c}{GPT-5-mini} & \multicolumn{2}{c}{Repeated real-vs.-real}\\
\cmidrule(lr){2-3}\cmidrule(lr){4-5}\cmidrule(lr){6-7}
& MWU $p$ & KS $p$ & MWU $p$ & KS $p$ & Med. MWU $p$ & Med. KS $p$\\
\midrule
\texttt{self\_bleu\_4} & 2.1e-24 & 1.6e-38 & 1.9e-09 & 3.6e-11 & 0.469 & 0.710\\
\texttt{self\_bertscore\_mean\_f1} & 1.1e-26 & 4.7e-49 & 6.8e-13 & 1.2e-25 & 0.473 & 0.710\\
\texttt{semantic\_mean\_cosine} & 1.1e-26 & 8.2e-51 & 7.7e-16 & 1.6e-29 & 0.531 & 0.710\\
\texttt{mean\_story\_probability} & 1.9e-20 & 1.3e-23 & 1.6e-19 & 1.8e-21 & 0.548 & 0.475\\
\texttt{toxicity\_mean} & 3.4e-17 & 4.0e-21 & 1.2e-05 & 5.3e-05 & 0.473 & 0.710\\
\texttt{severe\_toxicity\_mean} & 2.6e-18 & 1.6e-25 & 2.5e-06 & 5.9e-08 & 0.449 & 0.475\\
\texttt{obscene\_mean} & 1.1e-17 & 7.0e-20 & 5.2e-05 & 4.0e-06 & 0.522 & 0.710\\
\texttt{threat\_mean} & 2.9e-15 & 2.0e-21 & 2.4e-08 & 2.9e-10 & 0.479 & 0.710\\
\texttt{aggression\_score\_mean} & 1.7e-16 & 7.2e-21 & 1.3e-05 & 1.0e-04 & 0.548 & 0.710\\
\texttt{length\_std} & 2.3e-12 & 1.6e-21 & 4.3e-09 & 1.2e-11 & 0.485 & 0.710\\
\texttt{length\_cv} & 1.0e-16 & 1.8e-33 & 5.4e-13 & 1.9e-16 & 0.528 & 0.710\\
\texttt{avg\_depth} & 9.8e-20 & 3.8e-28 & 2.1e-21 & 3.8e-28 & 0.474 & 0.710\\
\texttt{structural\_virality} & 9.5e-20 & 3.8e-28 & 9.5e-20 & 3.8e-28 & 0.451 & 0.710\\
\bottomrule
\end{tabular}%
}
\caption{Per-metric significance comparison for the headphones domain. Lower baseline $p$-values indicate that generated and held-out real threads remain easier to distinguish. The final block gives the same-domain median real-vs.-real repeated-sample reference from the 200 within-domain resampling runs.}
\label{tab:appendix_oasis_headphones_pvalues}
\end{table}

\begin{table}[H]
\centering
\scriptsize
\setlength{\tabcolsep}{4pt}
\renewcommand{\arraystretch}{0.92}
\resizebox{\linewidth}{!}{%
\begin{tabular}{lcccccccccccc}
\toprule
Metric & \multicolumn{4}{c}{GPT-4o-mini} & \multicolumn{4}{c}{GPT-5-mini} & \multicolumn{4}{c}{Repeated real-vs.-real}\\
\cmidrule(lr){2-5}\cmidrule(lr){6-9}\cmidrule(lr){10-13}
& $W_1$ & Quant. err. & Emp. fail & $|\delta_{\mathrm{Cliff}}|$ & $W_1$ & Quant. err. & Emp. fail & $|\delta_{\mathrm{Cliff}}|$ & Med. $W_1$ & Med. quant. err. & Med. emp. fail & Med. $|\delta_{\mathrm{Cliff}}|$\\
\midrule
\texttt{self\_bleu\_4} & 0.0812 & 0.0850 & 0.6735 & 0.9164 & 0.0281 & 0.0272 & 0.2041 & 0.5395 & 0.0086 & 0.0070 & 0.0400 & 0.1168\\
\texttt{self\_bertscore\_mean\_f1} & 0.2395 & 0.2932 & 0.9796 & 0.9609 & 0.1143 & 0.1011 & 0.7959 & 0.6456 & 0.0374 & 0.0556 & 0.0e+00 & 0.1080\\
\texttt{semantic\_mean\_cosine} & 0.5464 & 0.5719 & 0.9796 & 0.9609 & 0.3821 & 0.3609 & 0.8163 & 0.7243 & 0.0412 & 0.0448 & 0.0e+00 & 0.1056\\
\texttt{mean\_story\_probability} & 0.1898 & 0.1833 & 0.3061 & 0.8333 & 0.1797 & 0.1841 & 0.4694 & 0.8126 & 0.0466 & 0.0439 & 0.0400 & 0.1136\\
\texttt{toxicity\_mean} & 0.0383 & 0.0337 & 0.0816 & 0.7583 & 0.0279 & 0.0258 & 0.1429 & 0.3944 & 0.0150 & 0.0114 & 0.0400 & 0.1104\\
\texttt{severe\_toxicity\_mean} & 3.0e-04 & 1.5e-04 & 0.1224 & 0.7850 & 2.9e-04 & 1.5e-04 & 0.1429 & 0.4233 & 2.0e-04 & 1.1e-04 & 0.0400 & 0.1104\\
\texttt{obscene\_mean} & 0.0181 & 0.0162 & 0.0612 & 0.7700 & 0.0151 & 0.0160 & 0.1429 & 0.3639 & 0.0093 & 0.0070 & 0.0e+00 & 0.1248\\
\texttt{threat\_mean} & 0.0013 & 3.7e-04 & 0.0408 & 0.7101 & 0.0012 & 3.5e-04 & 0.1837 & 0.5019 & 0.0012 & 4.1e-04 & 0.0400 & 0.1096\\
\texttt{aggression\_score\_mean} & 0.0128 & 0.0116 & 0.0816 & 0.7414 & 0.0095 & 0.0093 & 0.1429 & 0.3918 & 0.0053 & 0.0039 & 0.0400 & 0.1120\\
\texttt{length\_std} & 21.35 & 19.62 & 0.0e+00 & 0.6308 & 30.14 & 28.78 & 0.2857 & 0.5276 & 8.059 & 6.760 & 0.0e+00 & 0.1232\\
\texttt{length\_cv} & 0.6314 & 0.6033 & 0.0e+00 & 0.7462 & 0.4236 & 0.3835 & 0.0e+00 & 0.6485 & 0.1355 & 0.1417 & 0.0e+00 & 0.1168\\
\texttt{avg\_depth} & 0.8610 & 0.8311 & 0.0e+00 & 0.8038 & 1.020 & 1.031 & 0.2041 & 0.8438 & 0.2175 & 0.1864 & 0.0e+00 & 0.1120\\
\texttt{structural\_virality} & 1.702 & 1.665 & 0.0e+00 & 0.8038 & 1.702 & 1.665 & 0.0e+00 & 0.8038 & 0.3645 & 0.3563 & 0.0e+00 & 0.1096\\
\bottomrule
\end{tabular}%
}
\caption{Per-metric discrepancy comparison for the headphones domain. Lower is better for all reported statistics. The final block gives the same-domain median real-vs.-real repeated-sample reference from the 200 within-domain resampling runs, which serves as the calibration target for judging whether a baseline is still outside normal within-domain variation.}
\label{tab:appendix_oasis_headphones_distances}
\end{table}


\section{Full Prompt-Adjustment Case Study}
\label{app:oasis_improvement_case_study}

Section~\ref{sec:results} reports the uncalibrated OASIS baselines in the main paper and uses repeated real-vs.-real references to show that current simulations remain far from the real Reddit thread distribution. For completeness, this appendix also reports the full before/after comparison for the subset of domain--model pairs with prompt-adjusted runs. Before denotes the uncalibrated OASIS baseline, After denotes the prompt-adjusted simulator, and $\Delta\%$ is the relative percentage change from Before to After.

\begin{table}[H]
\centering
\scriptsize
\setlength{\tabcolsep}{2.2pt}
\renewcommand{\arraystretch}{0.82}
\resizebox{\textwidth}{!}{%
\begin{tabular}{ll|ccc|ccc|ccc|ccc|ccc}
\toprule
\textbf{Domain}
& \textbf{Model}
& \multicolumn{3}{c|}{$\mathbf{W_1}$}
& \multicolumn{3}{c|}{\textbf{Quant. err.}}
& \multicolumn{3}{c|}{\textbf{Emp. fail}}
& \multicolumn{3}{c|}{\textbf{Abs. med. gap}}
& \multicolumn{3}{c}{$\mathbf{|\delta_{\mathrm{Cliff}}|}$} \\
\cmidrule(lr){3-5}
\cmidrule(lr){6-8}
\cmidrule(lr){9-11}
\cmidrule(lr){12-14}
\cmidrule(lr){15-17}
&
& \textbf{Before} & \textbf{After} & $\mathbf{\Delta\%}$
& \textbf{Before} & \textbf{After} & $\mathbf{\Delta\%}$
& \textbf{Before} & \textbf{After} & $\mathbf{\Delta\%}$
& \textbf{Before} & \textbf{After} & $\mathbf{\Delta\%}$
& \textbf{Before} & \textbf{After} & $\mathbf{\Delta\%}$ \\
\midrule

Laptop
& GPT-4o-mini
& $1.190$ & $\mathbf{1.108}$ & $\mathbf{-6.9}$
& $1.129$ & $\mathbf{1.088}$ & $\mathbf{-3.7}$
& $0.107$ & $0.108$ & $+0.6$
& $0.871$ & $\mathbf{0.833}$ & $\mathbf{-4.4}$
& $0.676$ & $0.706$ & $+4.4$ \\
\midrule
\multirow{2}{*}{Credit Card}
& GPT-4o-mini
& $1.629$ & $\mathbf{1.507}$ & $\mathbf{-7.5}$
& $1.480$ & $\mathbf{1.390}$ & $\mathbf{-6.1}$
& $0.121$ & $\mathbf{0.119}$ & $\mathbf{-1.5}$
& $1.207$ & $\mathbf{1.095}$ & $\mathbf{-9.2}$
& $0.712$ & $0.771$ & $+8.3$ \\

& GPT-5-mini
& $3.617$ & $\mathbf{3.472}$ & $\mathbf{-4.0}$
& $3.422$ & $3.491$ & $+2.0$
& $0.142$ & $0.149$ & $+5.1$
& $3.936$ & $\mathbf{3.847}$ & $\mathbf{-2.3}$
& $0.322$ & $0.395$ & $+22.6$ \\
\midrule
Cellphone
& GPT-4o-mini
& $1.855$ & $1.868$ & $+0.7$
& $1.891$ & $\mathbf{1.889}$ & $\mathbf{-0.1}$
& $0.114$ & $0.116$ & $+2.0$
& $1.445$ & $\mathbf{1.421}$ & $\mathbf{-1.6}$
& $0.819$ & $\mathbf{0.792}$ & $\mathbf{-3.3}$ \\
\midrule
Camera
& GPT-4o-mini
& $2.514$ & $\mathbf{2.362}$ & $\mathbf{-6.0}$
& $2.383$ & $\mathbf{2.203}$ & $\mathbf{-7.6}$
& $0.174$ & $0.178$ & $+2.1$
& $2.114$ & $\mathbf{1.945}$ & $\mathbf{-8.0}$
& $0.608$ & $0.641$ & $+5.4$ \\
\midrule
Headphones
& GPT-4o-mini
& $1.319$ & $\mathbf{1.206}$ & $\mathbf{-8.6}$
& $1.329$ & $\mathbf{1.218}$ & $\mathbf{-8.3}$
& $0.116$ & $\mathbf{0.114}$ & $\mathbf{-1.0}$
& $1.049$ & $\mathbf{0.905}$ & $\mathbf{-13.7}$
& $0.872$ & $\mathbf{0.870}$ & $\mathbf{-0.2}$ \\

\bottomrule
\end{tabular}
}
\caption{Full RedditSimBench before/after comparison for the lightweight prompt-based improvement procedure on the subset of domain--model pairs with prompt-adjusted runs. GPT-4o-mini is reported on Laptop, Credit Card, Cellphone, Camera, and Headphones; GPT-5-mini is currently reported on Credit Card. $W_1$ is average Wasserstein distance, Quant. err. is average quantile error, Emp. fail is empirical fail rate, Abs. med. gap is average absolute median gap across metrics, and $|\delta_{\mathrm{Cliff}}|$ is average absolute Cliff's delta across metrics. Lower is better for all reported discrepancy metrics, so negative $\Delta\%$ indicates improvement. Bold marks improved After and $\Delta\%$ entries.}
\label{tab:appendix_oasis_calibration_results}
\end{table}

% \input{sections/appendix_unified_baseline_pvalue_table}
