# Supplementary material for: ThreadBench: Benchmarking Realism in Agentic Simulation of Real-world Discussions
Source: arXiv:2606.14715 source file (2026-10-10)
Supplement: Supplementary file 4 [file appendix_unified_baseline_table.tex]

\clearpage
\begin{landscape}
{\scriptsize
\setlength{\tabcolsep}{2.2pt}
\renewcommand{\arraystretch}{0.90}
\begin{longtable}{@{}L{1.50cm}L{3.00cm}L{3.10cm}*{12}{r}@{}}
\caption{Full unified OASIS baseline comparison on ThreadBench across all five domains, all five currently evaluated models, and the 13 core metrics. Lower is better for $W_1$, quantile error, empirical fail rate, and $|\delta_{\mathrm{Cliff}}|$; larger $p$-values indicate that generated and held-out real threads are harder to distinguish. The repeated real-vs.-real columns give the same-domain median reference from the 200 within-domain resampling runs used for calibration.}
\label{tab:appendix_oasis_baseline_full}\\
\toprule
Domain & Model & Metric & \multicolumn{6}{c}{Baseline} & \multicolumn{6}{c}{Repeated real-vs.-real median}\\
\cmidrule(lr){4-9}\cmidrule(lr){10-15}
& & & MWU $p$ & KS $p$ & $W_1$ & \shortstack{Quant.\\err.} & \shortstack{Emp.\\fail} & $|\delta_{\mathrm{Cliff}}|$ & MWU $p$ & KS $p$ & $W_1$ & \shortstack{Quant.\\err.} & \shortstack{Emp.\\fail} & $|\delta_{\mathrm{Cliff}}|$\\
\midrule
\endfirsthead
\multicolumn{15}{l}{\small\itshape Table~\ref{tab:appendix_oasis_baseline_full} continued from previous page.}\\
\toprule
Domain & Model & Metric & \multicolumn{6}{c}{Baseline} & \multicolumn{6}{c}{Repeated real-vs.-real median}\\
\cmidrule(lr){4-9}\cmidrule(lr){10-15}
& & & MWU $p$ & KS $p$ & $W_1$ & \shortstack{Quant.\\err.} & \shortstack{Emp.\\fail} & $|\delta_{\mathrm{Cliff}}|$ & MWU $p$ & KS $p$ & $W_1$ & \shortstack{Quant.\\err.} & \shortstack{Emp.\\fail} & $|\delta_{\mathrm{Cliff}}|$\\
\midrule
\endhead
\midrule
\multicolumn{15}{r}{\small\itshape Continued on next page.}\\
\endfoot
\bottomrule
\endlastfoot
Laptop & GPT-4o-mini & \texttt{self\_bleu\_4} & 1.9e-16 & 3.2e-31 & 0.110 & 0.108 & 0.843 & 0.725 & 0.516 & 0.710 & 0.0088 & 0.0073 & 0.0e+00 & 0.1328\\
Laptop & GPT-4o-mini & \texttt{self\_bertscore\_mean\_f1} & 6.5e-17 & 1.4e-34 & 0.214 & 0.190 & 0.863 & 0.737 & 0.491 & 0.593 & 0.0399 & 0.0563 & 0.0e+00 & 0.1216\\
Laptop & GPT-4o-mini & \texttt{semantic\_mean\_cosine} & 4.3e-17 & 1.4e-34 & 0.482 & 0.446 & 0.863 & 0.741 & 0.567 & 0.710 & 0.0453 & 0.0479 & 0.0e+00 & 0.1184\\
Laptop & GPT-4o-mini & \texttt{mean\_story\_probability} & 3.4e-22 & 7.2e-24 & 0.172 & 0.158 & 0.118 & 0.855 & 0.516 & 0.710 & 0.0509 & 0.0418 & 0.0e+00 & 0.1184\\
Laptop & GPT-4o-mini & \texttt{toxicity\_mean} & 1.9e-11 & 1.8e-11 & 0.0240 & 0.0207 & 0.0784 & 0.593 & 0.441 & 0.475 & 0.0140 & 0.0102 & 0.0e+00 & 0.1200\\
Laptop & GPT-4o-mini & \texttt{severe\_toxicity\_mean} & 1.2e-16 & 1.5e-18 & 1.3e-04 & 5.1e-05 & 0.118 & 0.731 & 0.516 & 0.710 & 9.3e-05 & 4.2e-05 & 0.0e+00 & 0.1264\\
Laptop & GPT-4o-mini & \texttt{obscene\_mean} & 1.2e-10 & 1.6e-10 & 0.0126 & 0.0097 & 0.0784 & 0.569 & 0.467 & 0.710 & 0.0093 & 0.0059 & 0.0e+00 & 0.1224\\
Laptop & GPT-4o-mini & \texttt{threat\_mean} & 1.8e-17 & 7.5e-19 & 4.1e-04 & 5.4e-05 & 0.118 & 0.751 & 0.528 & 0.710 & 5.0e-04 & 4.5e-05 & 0.0400 & 0.1200\\
Laptop & GPT-4o-mini & \texttt{aggression\_score\_mean} & 2.4e-11 & 1.4e-11 & 0.0080 & 0.0068 & 0.0784 & 0.590 & 0.557 & 0.710 & 0.0048 & 0.0034 & 0.0e+00 & 0.1280\\
Laptop & GPT-4o-mini & \texttt{length\_std} & 2.0e-08 & 1.6e-17 & 18.81 & 17.51 & 0.0e+00 & 0.495 & 0.566 & 0.710 & 7.610 & 7.163 & 0.0e+00 & 0.1056\\
Laptop & GPT-4o-mini & \texttt{length\_cv} & 3.4e-17 & 8.1e-33 & 0.556 & 0.517 & 0.0e+00 & 0.743 & 0.482 & 0.710 & 0.1225 & 0.1297 & 0.0e+00 & 0.1096\\
Laptop & GPT-4o-mini & \texttt{avg\_depth} & 1.0e-20 & 2.6e-28 & 0.965 & 0.859 & 0.0784 & 0.810 & 0.471 & 0.710 & 0.2262 & 0.2078 & 0.0400 & 0.1072\\
Laptop & GPT-4o-mini & \texttt{structural\_virality} & 4.6e-20 & 2.6e-28 & 1.543 & 1.476 & 0.0e+00 & 0.794 & 0.452 & 0.710 & 0.3424 & 0.3437 & 0.0e+00 & 0.1120\\
\midrule
Laptop & GPT-5-mini & \texttt{self\_bleu\_4} & 6.7e-12 & 2.1e-17 & 0.0400 & 0.0395 & 0.220 & 0.610 & 0.516 & 0.710 & 0.0088 & 0.0073 & 0.0e+00 & 0.1328\\
Laptop & GPT-5-mini & \texttt{self\_bertscore\_mean\_f1} & 2.2e-16 & 8.7e-34 & 0.134 & 0.118 & 0.860 & 0.730 & 0.491 & 0.593 & 0.0399 & 0.0563 & 0.0e+00 & 0.1216\\
Laptop & GPT-5-mini & \texttt{semantic\_mean\_cosine} & 2.4e-16 & 6.4e-32 & 0.368 & 0.344 & 0.860 & 0.729 & 0.567 & 0.710 & 0.0453 & 0.0479 & 0.0e+00 & 0.1184\\
Laptop & GPT-5-mini & \texttt{mean\_story\_probability} & 8.9e-23 & 4.4e-25 & 0.171 & 0.165 & 0.620 & 0.874 & 0.516 & 0.710 & 0.0509 & 0.0418 & 0.0e+00 & 0.1184\\
Laptop & GPT-5-mini & \texttt{toxicity\_mean} & 0.0057 & 1.0e-03 & 0.0216 & 0.0196 & 0.120 & 0.246 & 0.441 & 0.475 & 0.0140 & 0.0102 & 0.0e+00 & 0.1200\\
Laptop & GPT-5-mini & \texttt{severe\_toxicity\_mean} & 0.179 & 0.0034 & 1.3e-04 & 5.0e-05 & 0.120 & 0.120 & 0.516 & 0.710 & 9.3e-05 & 4.2e-05 & 0.0e+00 & 0.1264\\
Laptop & GPT-5-mini & \texttt{obscene\_mean} & 0.0692 & 0.0018 & 0.0124 & 0.0097 & 0.120 & 0.162 & 0.467 & 0.710 & 0.0093 & 0.0059 & 0.0e+00 & 0.1224\\
Laptop & GPT-5-mini & \texttt{threat\_mean} & 0.0019 & 1.7e-04 & 3.8e-04 & 4.8e-05 & 0.120 & 0.276 & 0.528 & 0.710 & 5.0e-04 & 4.5e-05 & 0.0400 & 0.1200\\
Laptop & GPT-5-mini & \texttt{aggression\_score\_mean} & 0.0068 & 0.0011 & 0.0073 & 0.0065 & 0.120 & 0.241 & 0.557 & 0.710 & 0.0048 & 0.0034 & 0.0e+00 & 0.1280\\
Laptop & GPT-5-mini & \texttt{length\_std} & 4.0e-08 & 1.5e-10 & 35.54 & 34.03 & 0.240 & 0.488 & 0.566 & 0.710 & 7.610 & 7.163 & 0.0e+00 & 0.1056\\
Laptop & GPT-5-mini & \texttt{length\_cv} & 1.2e-09 & 4.1e-13 & 0.338 & 0.309 & 0.0e+00 & 0.540 & 0.482 & 0.710 & 0.1225 & 0.1297 & 0.0e+00 & 0.1096\\
Laptop & GPT-5-mini & \texttt{avg\_depth} & 9.3e-21 & 7.0e-28 & 1.007 & 1.059 & 0.120 & 0.819 & 0.471 & 0.710 & 0.2262 & 0.2078 & 0.0400 & 0.1072\\
Laptop & GPT-5-mini & \texttt{structural\_virality} & 9.6e-20 & 7.0e-28 & 1.543 & 1.476 & 0.0e+00 & 0.794 & 0.452 & 0.710 & 0.3424 & 0.3437 & 0.0e+00 & 0.1120\\
\midrule
Laptop & Gemini-3.1-Flash-Lite-Preview & \texttt{self\_bleu\_4} & 6.4e-06 & 2.5e-09 & 0.0120 & 0.0132 & 0.0e+00 & 0.398 & 0.516 & 0.710 & 0.0088 & 0.0073 & 0.0e+00 & 0.1328\\
Laptop & Gemini-3.1-Flash-Lite-Preview & \texttt{self\_bertscore\_mean\_f1} & 5.5e-23 & 1.4e-42 & 0.122 & 0.189 & 0.940 & 0.870 & 0.491 & 0.593 & 0.0399 & 0.0563 & 0.0e+00 & 0.1216\\
Laptop & Gemini-3.1-Flash-Lite-Preview & \texttt{semantic\_mean\_cosine} & 2.0e-19 & 1.1e-29 & 0.248 & 0.287 & 0.240 & 0.795 & 0.567 & 0.710 & 0.0453 & 0.0479 & 0.0e+00 & 0.1184\\
Laptop & Gemini-3.1-Flash-Lite-Preview & \texttt{mean\_story\_probability} & 5.6e-24 & 4.5e-27 & 0.176 & 0.170 & 0.700 & 0.891 & 0.516 & 0.710 & 0.0509 & 0.0418 & 0.0e+00 & 0.1184\\
Laptop & Gemini-3.1-Flash-Lite-Preview & \texttt{toxicity\_mean} & 1.1e-09 & 1.1e-12 & 0.0344 & 0.0308 & 0.0600 & 0.538 & 0.441 & 0.475 & 0.0140 & 0.0102 & 0.0e+00 & 0.1200\\
Laptop & Gemini-3.1-Flash-Lite-Preview & \texttt{severe\_toxicity\_mean} & 0.151 & 2.1e-04 & 1.2e-04 & 4.7e-05 & 0.0400 & 0.127 & 0.516 & 0.710 & 9.3e-05 & 4.2e-05 & 0.0e+00 & 0.1264\\
Laptop & Gemini-3.1-Flash-Lite-Preview & \texttt{obscene\_mean} & 0.0041 & 3.8e-07 & 0.0106 & 0.0081 & 0.0400 & 0.253 & 0.467 & 0.710 & 0.0093 & 0.0059 & 0.0e+00 & 0.1224\\
Laptop & Gemini-3.1-Flash-Lite-Preview & \texttt{threat\_mean} & 4.6e-04 & 7.5e-08 & 2.7e-04 & 1.3e-05 & 0.0600 & 0.309 & 0.528 & 0.710 & 5.0e-04 & 4.5e-05 & 0.0400 & 0.1200\\
Laptop & Gemini-3.1-Flash-Lite-Preview & \texttt{aggression\_score\_mean} & 3.3e-09 & 1.5e-12 & 0.0105 & 0.0089 & 0.0600 & 0.522 & 0.557 & 0.710 & 0.0048 & 0.0034 & 0.0e+00 & 0.1280\\
Laptop & Gemini-3.1-Flash-Lite-Preview & \texttt{length\_std} & 0.0312 & 5.2e-05 & 13.92 & 14.67 & 0.0e+00 & 0.190 & 0.566 & 0.710 & 7.610 & 7.163 & 0.0e+00 & 0.1056\\
Laptop & Gemini-3.1-Flash-Lite-Preview & \texttt{length\_cv} & 5.3e-14 & 6.8e-25 & 0.458 & 0.444 & 0.0e+00 & 0.663 & 0.482 & 0.710 & 0.1225 & 0.1297 & 0.0e+00 & 0.1096\\
Laptop & Gemini-3.1-Flash-Lite-Preview & \texttt{avg\_depth} & 3.6e-20 & 3.5e-28 & 0.905 & 0.845 & 0.0400 & 0.799 & 0.471 & 0.710 & 0.2262 & 0.2078 & 0.0400 & 0.1072\\
Laptop & Gemini-3.1-Flash-Lite-Preview & \texttt{structural\_virality} & 7.8e-20 & 3.5e-28 & 1.510 & 1.459 & 0.0e+00 & 0.790 & 0.452 & 0.710 & 0.3424 & 0.3437 & 0.0e+00 & 0.1120\\
\midrule
Laptop & DeepSeek-Chat & \texttt{self\_bleu\_4} & 1.1e-04 & 5.3e-05 & 0.0148 & 0.0140 & 0.0200 & 0.342 & 0.516 & 0.710 & 0.0088 & 0.0073 & 0.0e+00 & 0.1328\\
Laptop & DeepSeek-Chat & \texttt{self\_bertscore\_mean\_f1} & 9.2e-18 & 3.2e-32 & 0.0894 & 0.0800 & 0.840 & 0.757 & 0.491 & 0.593 & 0.0399 & 0.0563 & 0.0e+00 & 0.1216\\
Laptop & DeepSeek-Chat & \texttt{semantic\_mean\_cosine} & 2.9e-18 & 1.2e-34 & 0.390 & 0.353 & 0.880 & 0.768 & 0.567 & 0.710 & 0.0453 & 0.0479 & 0.0e+00 & 0.1184\\
Laptop & DeepSeek-Chat & \texttt{mean\_story\_probability} & 2.1e-13 & 1.9e-11 & 0.142 & 0.137 & 0.240 & 0.648 & 0.516 & 0.710 & 0.0509 & 0.0418 & 0.0e+00 & 0.1184\\
Laptop & DeepSeek-Chat & \texttt{toxicity\_mean} & 0.637 & 0.0597 & 0.0078 & 0.0085 & 0.100 & 0.0417 & 0.441 & 0.475 & 0.0140 & 0.0102 & 0.0e+00 & 0.1200\\
Laptop & DeepSeek-Chat & \texttt{severe\_toxicity\_mean} & 0.174 & 0.0526 & 1.2e-04 & 4.7e-05 & 0.0800 & 0.120 & 0.516 & 0.710 & 9.3e-05 & 4.2e-05 & 0.0e+00 & 0.1264\\
Laptop & DeepSeek-Chat & \texttt{obscene\_mean} & 0.872 & 0.0791 & 0.0111 & 0.0083 & 0.0800 & 0.0143 & 0.467 & 0.710 & 0.0093 & 0.0059 & 0.0e+00 & 0.1224\\
Laptop & DeepSeek-Chat & \texttt{threat\_mean} & 0.0210 & 0.0053 & 3.3e-04 & 3.6e-05 & 0.0800 & 0.204 & 0.528 & 0.710 & 5.0e-04 & 4.5e-05 & 0.0400 & 0.1200\\
Laptop & DeepSeek-Chat & \texttt{aggression\_score\_mean} & 0.668 & 0.0473 & 0.0031 & 0.0031 & 0.0800 & 0.0379 & 0.557 & 0.710 & 0.0048 & 0.0034 & 0.0e+00 & 0.1280\\
Laptop & DeepSeek-Chat & \texttt{length\_std} & 0.0020 & 4.2e-04 & 11.94 & 11.21 & 0.0200 & 0.273 & 0.566 & 0.710 & 7.610 & 7.163 & 0.0e+00 & 0.1056\\
Laptop & DeepSeek-Chat & \texttt{length\_cv} & 8.1e-12 & 2.8e-17 & 0.385 & 0.353 & 0.0e+00 & 0.602 & 0.482 & 0.710 & 0.1225 & 0.1297 & 0.0e+00 & 0.1096\\
Laptop & DeepSeek-Chat & \texttt{avg\_depth} & 1.6e-20 & 3.5e-28 & 0.945 & 0.845 & 0.0800 & 0.807 & 0.471 & 0.710 & 0.2262 & 0.2078 & 0.0400 & 0.1072\\
Laptop & DeepSeek-Chat & \texttt{structural\_virality} & 7.8e-20 & 3.5e-28 & 1.510 & 1.459 & 0.0e+00 & 0.790 & 0.452 & 0.710 & 0.3424 & 0.3437 & 0.0e+00 & 0.1120\\
\midrule
Laptop & DeepSeek-V4-Flash & \texttt{self\_bleu\_4} & 0.0357 & 0.0086 & 0.0112 & 0.0116 & 0.0e+00 & 0.280 & 0.516 & 0.710 & 0.0088 & 0.0073 & 0.0e+00 & 0.1328\\
Laptop & DeepSeek-V4-Flash & \texttt{self\_bertscore\_mean\_f1} & 4.8e-13 & 1.7e-21 & 0.142 & 0.177 & 0.850 & 0.965 & 0.491 & 0.593 & 0.0399 & 0.0563 & 0.0e+00 & 0.1216\\
Laptop & DeepSeek-V4-Flash & \texttt{semantic\_mean\_cosine} & 1.2e-13 & 4.5e-26 & 0.438 & 0.456 & 1.000 & 0.989 & 0.567 & 0.710 & 0.0453 & 0.0479 & 0.0e+00 & 0.1184\\
Laptop & DeepSeek-V4-Flash & \texttt{mean\_story\_probability} & 0.0115 & 0.0362 & 0.0864 & 0.0839 & 0.100 & 0.337 & 0.516 & 0.710 & 0.0509 & 0.0418 & 0.0e+00 & 0.1184\\
Laptop & DeepSeek-V4-Flash & \texttt{toxicity\_mean} & 0.188 & 0.132 & 0.0087 & 0.0033 & 0.0e+00 & 0.176 & 0.441 & 0.475 & 0.0140 & 0.0102 & 0.0e+00 & 0.1200\\
Laptop & DeepSeek-V4-Flash & \texttt{severe\_toxicity\_mean} & 0.626 & 0.424 & 1.1e-04 & 4.5e-05 & 0.0e+00 & 0.0652 & 0.516 & 0.710 & 9.3e-05 & 4.2e-05 & 0.0e+00 & 0.1264\\
Laptop & DeepSeek-V4-Flash & \texttt{obscene\_mean} & 0.224 & 0.0916 & 0.0073 & 0.0051 & 0.0e+00 & 0.162 & 0.467 & 0.710 & 0.0093 & 0.0059 & 0.0e+00 & 0.1224\\
Laptop & DeepSeek-V4-Flash & \texttt{threat\_mean} & 0.314 & 0.0632 & 3.5e-04 & 3.6e-05 & 0.0e+00 & 0.134 & 0.528 & 0.710 & 5.0e-04 & 4.5e-05 & 0.0400 & 0.1200\\
Laptop & DeepSeek-V4-Flash & \texttt{aggression\_score\_mean} & 0.192 & 0.151 & 0.0029 & 9.6e-04 & 0.0e+00 & 0.174 & 0.557 & 0.710 & 0.0048 & 0.0034 & 0.0e+00 & 0.1280\\
Laptop & DeepSeek-V4-Flash & \texttt{length\_std} & 1.2e-08 & 5.1e-09 & 37.95 & 37.70 & 0.0500 & 0.761 & 0.566 & 0.710 & 7.610 & 7.163 & 0.0e+00 & 0.1056\\
Laptop & DeepSeek-V4-Flash & \texttt{length\_cv} & 8.5e-04 & 1.0e-04 & 0.307 & 0.293 & 0.0e+00 & 0.445 & 0.482 & 0.710 & 0.1225 & 0.1297 & 0.0e+00 & 0.1096\\
Laptop & DeepSeek-V4-Flash & \texttt{avg\_depth} & 2.3e-09 & 8.9e-13 & 0.865 & 0.845 & 0.0e+00 & 0.790 & 0.471 & 0.710 & 0.2262 & 0.2078 & 0.0400 & 0.1072\\
Laptop & DeepSeek-V4-Flash & \texttt{structural\_virality} & 2.3e-09 & 8.9e-13 & 1.510 & 1.459 & 0.0e+00 & 0.790 & 0.452 & 0.710 & 0.3424 & 0.3437 & 0.0e+00 & 0.1120\\
\midrule
Credit Card & GPT-4o-mini & \texttt{self\_bleu\_4} & 2.1e-33 & 6.6e-76 & 0.136 & 0.136 & 1.000 & 0.993 & 0.528 & 0.710 & 0.0058 & 0.0047 & 0.0e+00 & 0.1008\\
Credit Card & GPT-4o-mini & \texttt{self\_bertscore\_mean\_f1} & 7.3e-34 & 3.4e-105 & 0.257 & 0.233 & 1.000 & 1.000 & 0.525 & 0.710 & 0.0276 & 0.0148 & 0.0e+00 & 0.1088\\
Credit Card & GPT-4o-mini & \texttt{semantic\_mean\_cosine} & 7.8e-34 & 1.8e-98 & 0.573 & 0.569 & 1.000 & 1.000 & 0.449 & 0.710 & 0.0423 & 0.0417 & 0.0400 & 0.1056\\
Credit Card & GPT-4o-mini & \texttt{mean\_story\_probability} & 1.8e-27 & 1.7e-41 & 0.156 & 0.149 & 0.360 & 0.895 & 0.473 & 0.710 & 0.0464 & 0.0419 & 0.0400 & 0.1104\\
Credit Card & GPT-4o-mini & \texttt{toxicity\_mean} & 4.0e-14 & 1.3e-13 & 0.0181 & 0.0150 & 0.0200 & 0.623 & 0.541 & 0.710 & 0.0106 & 0.0082 & 0.0e+00 & 0.1168\\
Credit Card & GPT-4o-mini & \texttt{severe\_toxicity\_mean} & 3.7e-25 & 1.1e-26 & 7.6e-05 & 2.7e-05 & 0.420 & 0.854 & 0.522 & 0.710 & 6.4e-05 & 2.6e-05 & 0.0e+00 & 0.1168\\
Credit Card & GPT-4o-mini & \texttt{obscene\_mean} & 2.9e-17 & 2.2e-16 & 0.0097 & 0.0066 & 0.120 & 0.697 & 0.473 & 0.710 & 0.0067 & 0.0047 & 0.0e+00 & 0.1232\\
Credit Card & GPT-4o-mini & \texttt{threat\_mean} & 1.7e-18 & 3.7e-21 & 2.7e-04 & 3.7e-05 & 0.100 & 0.724 & 0.528 & 0.710 & 2.1e-04 & 2.6e-05 & 0.0e+00 & 0.1104\\
Credit Card & GPT-4o-mini & \texttt{aggression\_score\_mean} & 1.1e-13 & 2.3e-13 & 0.0060 & 0.0049 & 0.0200 & 0.612 & 0.509 & 0.710 & 0.0037 & 0.0028 & 0.0e+00 & 0.1184\\
Credit Card & GPT-4o-mini & \texttt{length\_std} & 4.5e-17 & 1.1e-29 & 25.20 & 22.56 & 0.0e+00 & 0.692 & 0.506 & 0.710 & 8.796 & 7.126 & 0.0e+00 & 0.1136\\
Credit Card & GPT-4o-mini & \texttt{length\_cv} & 5.7e-24 & 1.7e-47 & 0.582 & 0.563 & 0.0e+00 & 0.832 & 0.485 & 0.710 & 0.1099 & 0.1050 & 0.0e+00 & 0.1120\\
Credit Card & GPT-4o-mini & \texttt{avg\_depth} & 1.1e-23 & 6.4e-37 & 0.941 & 0.913 & 0.0e+00 & 0.824 & 0.559 & 0.710 & 0.2217 & 0.2014 & 0.0400 & 0.0944\\
Credit Card & GPT-4o-mini & \texttt{structural\_virality} & 9.4e-24 & 6.4e-37 & 1.688 & 1.642 & 0.0e+00 & 0.824 & 0.470 & 0.710 & 0.3284 & 0.3347 & 0.0e+00 & 0.0984\\
\midrule
Credit Card & GPT-5-mini & \texttt{self\_bleu\_4} & 1.5e-13 & 3.1e-27 & 0.0558 & 0.0511 & 0.574 & 0.552 & 0.528 & 0.710 & 0.0058 & 0.0047 & 0.0e+00 & 0.1008\\
Credit Card & GPT-5-mini & \texttt{self\_bertscore\_mean\_f1} & 3.1e-17 & 6.5e-34 & 0.144 & 0.175 & 0.738 & 0.631 & 0.525 & 0.710 & 0.0276 & 0.0148 & 0.0e+00 & 0.1088\\
Credit Card & GPT-5-mini & \texttt{semantic\_mean\_cosine} & 8.2e-18 & 5.5e-39 & 0.344 & 0.349 & 0.803 & 0.643 & 0.449 & 0.710 & 0.0423 & 0.0417 & 0.0400 & 0.1056\\
Credit Card & GPT-5-mini & \texttt{mean\_story\_probability} & 1.8e-11 & 4.4e-12 & 0.0931 & 0.0899 & 0.443 & 0.503 & 0.473 & 0.710 & 0.0464 & 0.0419 & 0.0400 & 0.1104\\
Credit Card & GPT-5-mini & \texttt{toxicity\_mean} & 0.251 & 0.0798 & 0.0087 & 0.0096 & 0.148 & 0.0859 & 0.541 & 0.710 & 0.0106 & 0.0082 & 0.0e+00 & 0.1168\\
Credit Card & GPT-5-mini & \texttt{severe\_toxicity\_mean} & 0.438 & 0.0278 & 7.1e-05 & 2.5e-05 & 0.180 & 0.0580 & 0.522 & 0.710 & 6.4e-05 & 2.6e-05 & 0.0e+00 & 0.1168\\
Credit Card & GPT-5-mini & \texttt{obscene\_mean} & 0.780 & 0.0194 & 0.0079 & 0.0058 & 0.115 & 0.0209 & 0.473 & 0.710 & 0.0067 & 0.0047 & 0.0e+00 & 0.1232\\
Credit Card & GPT-5-mini & \texttt{threat\_mean} & 6.8e-05 & 0.0021 & 2.6e-04 & 3.2e-05 & 0.197 & 0.298 & 0.528 & 0.710 & 2.1e-04 & 2.6e-05 & 0.0e+00 & 0.1104\\
Credit Card & GPT-5-mini & \texttt{aggression\_score\_mean} & 0.272 & 0.0753 & 0.0029 & 0.0037 & 0.131 & 0.0821 & 0.509 & 0.710 & 0.0037 & 0.0028 & 0.0e+00 & 0.1184\\
Credit Card & GPT-5-mini & \texttt{length\_std} & 8.6e-07 & 3.0e-11 & 38.96 & 37.20 & 0.262 & 0.368 & 0.506 & 0.710 & 8.796 & 7.126 & 0.0e+00 & 0.1136\\
Credit Card & GPT-5-mini & \texttt{length\_cv} & 1.3e-20 & 1.2e-23 & 0.412 & 0.399 & 0.0e+00 & 0.696 & 0.485 & 0.710 & 0.1099 & 0.1050 & 0.0e+00 & 0.1120\\
Credit Card & GPT-5-mini & \texttt{avg\_depth} & 9.1e-30 & 1.1e-44 & 1.055 & 1.113 & 0.115 & 0.844 & 0.559 & 0.710 & 0.2217 & 0.2014 & 0.0400 & 0.0944\\
Credit Card & GPT-5-mini & \texttt{structural\_virality} & 1.6e-28 & 1.1e-44 & 1.688 & 1.642 & 0.0e+00 & 0.824 & 0.470 & 0.710 & 0.3284 & 0.3347 & 0.0e+00 & 0.0984\\
\midrule
Credit Card & Gemini-3.1-Flash-Lite-Preview & \texttt{self\_bleu\_4} & 8.6e-06 & 2.6e-08 & 0.0098 & 0.0084 & 0.0e+00 & 0.367 & 0.528 & 0.710 & 0.0058 & 0.0047 & 0.0e+00 & 0.1008\\
Credit Card & Gemini-3.1-Flash-Lite-Preview & \texttt{self\_bertscore\_mean\_f1} & 3.7e-28 & 7.5e-47 & 0.0884 & 0.0753 & 0.720 & 0.907 & 0.525 & 0.710 & 0.0276 & 0.0148 & 0.0e+00 & 0.1088\\
Credit Card & Gemini-3.1-Flash-Lite-Preview & \texttt{semantic\_mean\_cosine} & 6.4e-19 & 5.2e-24 & 0.166 & 0.167 & 0.0200 & 0.732 & 0.449 & 0.710 & 0.0423 & 0.0417 & 0.0400 & 0.1056\\
Credit Card & Gemini-3.1-Flash-Lite-Preview & \texttt{mean\_story\_probability} & 4.6e-28 & 2.1e-31 & 0.155 & 0.151 & 0.740 & 0.905 & 0.473 & 0.710 & 0.0464 & 0.0419 & 0.0400 & 0.1104\\
Credit Card & Gemini-3.1-Flash-Lite-Preview & \texttt{toxicity\_mean} & 8.2e-10 & 3.6e-11 & 0.0252 & 0.0261 & 0.0600 & 0.506 & 0.541 & 0.710 & 0.0106 & 0.0082 & 0.0e+00 & 0.1168\\
Credit Card & Gemini-3.1-Flash-Lite-Preview & \texttt{severe\_toxicity\_mean} & 0.0038 & 3.6e-06 & 7.2e-05 & 2.5e-05 & 0.0200 & 0.238 & 0.522 & 0.710 & 6.4e-05 & 2.6e-05 & 0.0e+00 & 0.1168\\
Credit Card & Gemini-3.1-Flash-Lite-Preview & \texttt{obscene\_mean} & 0.0020 & 3.5e-08 & 0.0084 & 0.0063 & 0.0200 & 0.255 & 0.473 & 0.710 & 0.0067 & 0.0047 & 0.0e+00 & 0.1232\\
Credit Card & Gemini-3.1-Flash-Lite-Preview & \texttt{threat\_mean} & 1.5e-06 & 7.2e-11 & 2.5e-04 & 2.2e-05 & 0.0200 & 0.397 & 0.528 & 0.710 & 2.1e-04 & 2.6e-05 & 0.0e+00 & 0.1104\\
Credit Card & Gemini-3.1-Flash-Lite-Preview & \texttt{aggression\_score\_mean} & 1.8e-09 & 7.5e-11 & 0.0077 & 0.0080 & 0.0600 & 0.496 & 0.509 & 0.710 & 0.0037 & 0.0028 & 0.0e+00 & 0.1184\\
Credit Card & Gemini-3.1-Flash-Lite-Preview & \texttt{length\_std} & 1.7e-07 & 6.7e-11 & 18.14 & 16.67 & 0.0e+00 & 0.431 & 0.506 & 0.710 & 8.796 & 7.126 & 0.0e+00 & 0.1136\\
Credit Card & Gemini-3.1-Flash-Lite-Preview & \texttt{length\_cv} & 1.7e-21 & 5.0e-35 & 0.482 & 0.451 & 0.0e+00 & 0.785 & 0.485 & 0.710 & 0.1099 & 0.1050 & 0.0e+00 & 0.1120\\
Credit Card & Gemini-3.1-Flash-Lite-Preview & \texttt{avg\_depth} & 5.6e-24 & 3.6e-37 & 0.964 & 0.913 & 0.0200 & 0.830 & 0.559 & 0.710 & 0.2217 & 0.2014 & 0.0400 & 0.0944\\
Credit Card & Gemini-3.1-Flash-Lite-Preview & \texttt{structural\_virality} & 7.5e-24 & 3.6e-37 & 1.695 & 1.644 & 0.0e+00 & 0.826 & 0.470 & 0.710 & 0.3284 & 0.3347 & 0.0e+00 & 0.0984\\
\midrule
Credit Card & DeepSeek-Chat & \texttt{self\_bleu\_4} & 3.5e-07 & 4.8e-05 & 0.0159 & 0.0164 & 0.0857 & 0.500 & 0.528 & 0.710 & 0.0058 & 0.0047 & 0.0e+00 & 0.1008\\
Credit Card & DeepSeek-Chat & \texttt{self\_bertscore\_mean\_f1} & 4.7e-20 & 4.7e-26 & 0.0954 & 0.0717 & 0.400 & 0.901 & 0.525 & 0.710 & 0.0276 & 0.0148 & 0.0e+00 & 0.1088\\
Credit Card & DeepSeek-Chat & \texttt{semantic\_mean\_cosine} & 3.0e-22 & 2.2e-39 & 0.361 & 0.363 & 0.886 & 0.953 & 0.449 & 0.710 & 0.0423 & 0.0417 & 0.0400 & 0.1056\\
Credit Card & DeepSeek-Chat & \texttt{mean\_story\_probability} & 0.0017 & 0.0173 & 0.0748 & 0.0788 & 0.0857 & 0.309 & 0.473 & 0.710 & 0.0464 & 0.0419 & 0.0400 & 0.1104\\
Credit Card & DeepSeek-Chat & \texttt{toxicity\_mean} & 0.187 & 0.0320 & 0.0075 & 0.0061 & 0.0e+00 & 0.130 & 0.541 & 0.710 & 0.0106 & 0.0082 & 0.0e+00 & 0.1168\\
Credit Card & DeepSeek-Chat & \texttt{severe\_toxicity\_mean} & 0.930 & 0.149 & 7.1e-05 & 2.6e-05 & 0.0e+00 & 0.0086 & 0.522 & 0.710 & 6.4e-05 & 2.6e-05 & 0.0e+00 & 0.1168\\
Credit Card & DeepSeek-Chat & \texttt{obscene\_mean} & 0.178 & 0.0064 & 0.0071 & 0.0059 & 0.0e+00 & 0.132 & 0.473 & 0.710 & 0.0067 & 0.0047 & 0.0e+00 & 0.1232\\
Credit Card & DeepSeek-Chat & \texttt{threat\_mean} & 0.312 & 0.0094 & 2.6e-04 & 2.8e-05 & 0.0e+00 & 0.0993 & 0.528 & 0.710 & 2.1e-04 & 2.6e-05 & 0.0e+00 & 0.1104\\
Credit Card & DeepSeek-Chat & \texttt{aggression\_score\_mean} & 0.173 & 0.0141 & 0.0028 & 0.0020 & 0.0e+00 & 0.134 & 0.509 & 0.710 & 0.0037 & 0.0028 & 0.0e+00 & 0.1184\\
Credit Card & DeepSeek-Chat & \texttt{length\_std} & 1.6e-06 & 8.8e-07 & 22.21 & 20.99 & 0.0e+00 & 0.472 & 0.506 & 0.710 & 8.796 & 7.126 & 0.0e+00 & 0.1136\\
Credit Card & DeepSeek-Chat & \texttt{length\_cv} & 4.2e-11 & 2.1e-17 & 0.351 & 0.324 & 0.0e+00 & 0.648 & 0.485 & 0.710 & 0.1099 & 0.1050 & 0.0e+00 & 0.1120\\
Credit Card & DeepSeek-Chat & \texttt{avg\_depth} & 3.3e-17 & 2.3e-26 & 0.944 & 0.913 & 0.0e+00 & 0.826 & 0.559 & 0.710 & 0.2217 & 0.2014 & 0.0400 & 0.0944\\
Credit Card & DeepSeek-Chat & \texttt{structural\_virality} & 3.0e-17 & 2.3e-26 & 1.695 & 1.644 & 0.0e+00 & 0.826 & 0.470 & 0.710 & 0.3284 & 0.3347 & 0.0e+00 & 0.0984\\
\midrule
Credit Card & DeepSeek-V4-Flash & \texttt{self\_bleu\_4} & 8.9e-07 & 1.2e-06 & 0.0137 & 0.0128 & 0.0952 & 0.441 & 0.528 & 0.710 & 0.0058 & 0.0047 & 0.0e+00 & 0.1008\\
Credit Card & DeepSeek-V4-Flash & \texttt{self\_bertscore\_mean\_f1} & 1.5e-20 & 2.4e-29 & 0.0785 & 0.0654 & 0.286 & 0.834 & 0.525 & 0.710 & 0.0276 & 0.0148 & 0.0e+00 & 0.1088\\
Credit Card & DeepSeek-V4-Flash & \texttt{semantic\_mean\_cosine} & 1.2e-24 & 1.8e-40 & 0.347 & 0.359 & 0.810 & 0.920 & 0.449 & 0.710 & 0.0423 & 0.0417 & 0.0400 & 0.1056\\
Credit Card & DeepSeek-V4-Flash & \texttt{mean\_story\_probability} & 0.296 & 0.286 & 0.0260 & 0.0171 & 0.143 & 0.0939 & 0.473 & 0.710 & 0.0464 & 0.0419 & 0.0400 & 0.1104\\
Credit Card & DeepSeek-V4-Flash & \texttt{toxicity\_mean} & 0.0311 & 1.8e-04 & 0.0078 & 0.0068 & 0.0e+00 & 0.194 & 0.541 & 0.710 & 0.0106 & 0.0082 & 0.0e+00 & 0.1168\\
Credit Card & DeepSeek-V4-Flash & \texttt{severe\_toxicity\_mean} & 0.440 & 0.0868 & 6.8e-05 & 2.2e-05 & 0.0238 & 0.0694 & 0.522 & 0.710 & 6.4e-05 & 2.6e-05 & 0.0e+00 & 0.1168\\
Credit Card & DeepSeek-V4-Flash & \texttt{obscene\_mean} & 0.0141 & 0.0027 & 0.0038 & 0.0032 & 0.0e+00 & 0.221 & 0.473 & 0.710 & 0.0067 & 0.0047 & 0.0e+00 & 0.1232\\
Credit Card & DeepSeek-V4-Flash & \texttt{threat\_mean} & 0.705 & 0.0920 & 2.6e-04 & 2.5e-05 & 0.0e+00 & 0.0340 & 0.528 & 0.710 & 2.1e-04 & 2.6e-05 & 0.0e+00 & 0.1104\\
Credit Card & DeepSeek-V4-Flash & \texttt{aggression\_score\_mean} & 0.0271 & 1.2e-04 & 0.0025 & 0.0022 & 0.0e+00 & 0.199 & 0.509 & 0.710 & 0.0037 & 0.0028 & 0.0e+00 & 0.1184\\
Credit Card & DeepSeek-V4-Flash & \texttt{length\_std} & 8.6e-06 & 1.1e-06 & 15.21 & 16.68 & 0.0238 & 0.400 & 0.506 & 0.710 & 8.796 & 7.126 & 0.0e+00 & 0.1136\\
Credit Card & DeepSeek-V4-Flash & \texttt{length\_cv} & 1.6e-15 & 1.7e-23 & 0.412 & 0.407 & 0.0e+00 & 0.716 & 0.485 & 0.710 & 0.1099 & 0.1050 & 0.0e+00 & 0.1120\\
Credit Card & DeepSeek-V4-Flash & \texttt{avg\_depth} & 2.7e-20 & 1.9e-31 & 0.944 & 0.913 & 0.0e+00 & 0.826 & 0.559 & 0.710 & 0.2217 & 0.2014 & 0.0400 & 0.0944\\
Credit Card & DeepSeek-V4-Flash & \texttt{structural\_virality} & 2.4e-20 & 1.9e-31 & 1.695 & 1.644 & 0.0e+00 & 0.826 & 0.470 & 0.710 & 0.3284 & 0.3347 & 0.0e+00 & 0.0984\\
\midrule
Cellphone & GPT-4o-mini & \texttt{self\_bleu\_4} & 9.7e-19 & 8.1e-32 & 0.0698 & 0.0774 & 0.455 & 0.816 & 0.503 & 0.710 & 0.0089 & 0.0069 & 0.0e+00 & 0.1320\\
Cellphone & GPT-4o-mini & \texttt{self\_bertscore\_mean\_f1} & 1.5e-20 & 4.9e-40 & 0.182 & 0.202 & 0.932 & 0.858 & 0.475 & 0.710 & 0.0385 & 0.0382 & 0.0e+00 & 0.1200\\
Cellphone & GPT-4o-mini & \texttt{semantic\_mean\_cosine} & 6.0e-21 & 1.8e-40 & 0.470 & 0.506 & 0.932 & 0.867 & 0.482 & 0.475 & 0.0389 & 0.0397 & 0.0e+00 & 0.1160\\
Cellphone & GPT-4o-mini & \texttt{mean\_story\_probability} & 4.1e-24 & 3.4e-30 & 0.199 & 0.190 & 0.750 & 0.936 & 0.464 & 0.475 & 0.0433 & 0.0412 & 0.0e+00 & 0.1120\\
Cellphone & GPT-4o-mini & \texttt{toxicity\_mean} & 1.9e-22 & 4.1e-29 & 0.0233 & 0.0219 & 0.341 & 0.900 & 0.516 & 0.710 & 0.0084 & 0.0068 & 0.0e+00 & 0.1136\\
Cellphone & GPT-4o-mini & \texttt{severe\_toxicity\_mean} & 1.1e-22 & 1.4e-28 & 8.8e-05 & 3.3e-05 & 0.477 & 0.906 & 0.500 & 0.710 & 5.1e-05 & 2.3e-05 & 0.0e+00 & 0.1216\\
Cellphone & GPT-4o-mini & \texttt{obscene\_mean} & 4.5e-22 & 4.3e-28 & 0.0119 & 0.0107 & 0.341 & 0.892 & 0.554 & 0.710 & 0.0053 & 0.0049 & 0.0e+00 & 0.1144\\
Cellphone & GPT-4o-mini & \texttt{threat\_mean} & 1.6e-21 & 2.2e-27 & 2.9e-04 & 7.9e-05 & 0.432 & 0.880 & 0.551 & 0.710 & 1.4e-04 & 5.8e-05 & 0.0e+00 & 0.1040\\
Cellphone & GPT-4o-mini & \texttt{aggression\_score\_mean} & 1.9e-22 & 1.2e-29 & 0.0077 & 0.0073 & 0.341 & 0.900 & 0.541 & 0.710 & 0.0029 & 0.0025 & 0.0e+00 & 0.1168\\
Cellphone & GPT-4o-mini & \texttt{length\_std} & 2.7e-15 & 2.6e-27 & 27.67 & 24.86 & 0.0e+00 & 0.730 & 0.491 & 0.475 & 9.183 & 7.239 & 0.0e+00 & 0.1192\\
Cellphone & GPT-4o-mini & \texttt{length\_cv} & 8.6e-20 & 1.3e-35 & 0.697 & 0.688 & 0.0e+00 & 0.841 & 0.458 & 0.710 & 0.1211 & 0.1296 & 0.0e+00 & 0.1136\\
Cellphone & GPT-4o-mini & \texttt{avg\_depth} & 1.6e-19 & 2.9e-28 & 0.964 & 0.892 & 0.0455 & 0.827 & 0.484 & 0.475 & 0.2115 & 0.2111 & 0.0e+00 & 0.1136\\
Cellphone & GPT-4o-mini & \texttt{structural\_virality} & 3.3e-19 & 2.9e-28 & 1.840 & 1.784 & 0.0e+00 & 0.818 & 0.498 & 0.710 & 0.3649 & 0.3836 & 0.0e+00 & 0.1104\\
\midrule
Cellphone & GPT-5-mini & \texttt{self\_bleu\_4} & 7.4e-21 & 2.3e-32 & 0.0618 & 0.0656 & 0.379 & 0.766 & 0.503 & 0.710 & 0.0089 & 0.0069 & 0.0e+00 & 0.1320\\
Cellphone & GPT-5-mini & \texttt{self\_bertscore\_mean\_f1} & 5.0e-25 & 2.0e-45 & 0.135 & 0.151 & 0.914 & 0.845 & 0.475 & 0.710 & 0.0385 & 0.0382 & 0.0e+00 & 0.1200\\
Cellphone & GPT-5-mini & \texttt{semantic\_mean\_cosine} & 3.8e-26 & 1.5e-50 & 0.437 & 0.473 & 0.931 & 0.865 & 0.482 & 0.475 & 0.0389 & 0.0397 & 0.0e+00 & 0.1160\\
Cellphone & GPT-5-mini & \texttt{mean\_story\_probability} & 2.1e-28 & 8.7e-32 & 0.192 & 0.189 & 0.638 & 0.904 & 0.464 & 0.475 & 0.0433 & 0.0412 & 0.0e+00 & 0.1120\\
Cellphone & GPT-5-mini & \texttt{toxicity\_mean} & 2.5e-04 & 1.3e-05 & 0.0151 & 0.0158 & 0.0862 & 0.300 & 0.516 & 0.710 & 0.0084 & 0.0068 & 0.0e+00 & 0.1136\\
Cellphone & GPT-5-mini & \texttt{severe\_toxicity\_mean} & 0.0271 & 0.0023 & 8.3e-05 & 3.0e-05 & 0.0690 & 0.181 & 0.500 & 0.710 & 5.1e-05 & 2.3e-05 & 0.0e+00 & 0.1216\\
Cellphone & GPT-5-mini & \texttt{obscene\_mean} & 0.0022 & 2.4e-05 & 0.0102 & 0.0105 & 0.0517 & 0.251 & 0.554 & 0.710 & 0.0053 & 0.0049 & 0.0e+00 & 0.1144\\
Cellphone & GPT-5-mini & \texttt{threat\_mean} & 3.0e-05 & 9.7e-05 & 2.6e-04 & 6.0e-05 & 0.0862 & 0.341 & 0.551 & 0.710 & 1.4e-04 & 5.8e-05 & 0.0e+00 & 0.1040\\
Cellphone & GPT-5-mini & \texttt{aggression\_score\_mean} & 3.6e-04 & 4.2e-05 & 0.0049 & 0.0053 & 0.0862 & 0.292 & 0.541 & 0.710 & 0.0029 & 0.0025 & 0.0e+00 & 0.1168\\
Cellphone & GPT-5-mini & \texttt{length\_std} & 2.6e-14 & 1.1e-14 & 38.59 & 40.47 & 0.259 & 0.623 & 0.491 & 0.475 & 9.183 & 7.239 & 0.0e+00 & 0.1192\\
Cellphone & GPT-5-mini & \texttt{length\_cv} & 1.2e-20 & 2.2e-28 & 0.505 & 0.499 & 0.0e+00 & 0.762 & 0.458 & 0.710 & 0.1211 & 0.1296 & 0.0e+00 & 0.1136\\
Cellphone & GPT-5-mini & \texttt{avg\_depth} & 1.3e-24 & 1.3e-35 & 0.970 & 0.892 & 0.0517 & 0.828 & 0.484 & 0.475 & 0.2115 & 0.2111 & 0.0e+00 & 0.1136\\
Cellphone & GPT-5-mini & \texttt{structural\_virality} & 3.6e-24 & 1.3e-35 & 1.840 & 1.784 & 0.0e+00 & 0.818 & 0.498 & 0.710 & 0.3649 & 0.3836 & 0.0e+00 & 0.1104\\
\midrule
Cellphone & Gemini-3.1-Flash-Lite-Preview & \texttt{self\_bleu\_4} & 1.0e-04 & 6.2e-08 & 0.0105 & 0.0099 & 0.0e+00 & 0.339 & 0.503 & 0.710 & 0.0089 & 0.0069 & 0.0e+00 & 0.1320\\
Cellphone & Gemini-3.1-Flash-Lite-Preview & \texttt{self\_bertscore\_mean\_f1} & 3.0e-26 & 3.5e-50 & 0.115 & 0.103 & 0.980 & 0.925 & 0.475 & 0.710 & 0.0385 & 0.0382 & 0.0e+00 & 0.1200\\
Cellphone & Gemini-3.1-Flash-Lite-Preview & \texttt{semantic\_mean\_cosine} & 4.8e-24 & 3.9e-35 & 0.231 & 0.237 & 0.440 & 0.883 & 0.482 & 0.475 & 0.0389 & 0.0397 & 0.0e+00 & 0.1160\\
Cellphone & Gemini-3.1-Flash-Lite-Preview & \texttt{mean\_story\_probability} & 7.5e-28 & 5.8e-35 & 0.202 & 0.192 & 0.860 & 0.955 & 0.464 & 0.475 & 0.0433 & 0.0412 & 0.0e+00 & 0.1120\\
Cellphone & Gemini-3.1-Flash-Lite-Preview & \texttt{toxicity\_mean} & 3.9e-07 & 2.4e-06 & 0.0306 & 0.0241 & 0.0600 & 0.443 & 0.516 & 0.710 & 0.0084 & 0.0068 & 0.0e+00 & 0.1136\\
Cellphone & Gemini-3.1-Flash-Lite-Preview & \texttt{severe\_toxicity\_mean} & 0.639 & 0.0339 & 6.6e-05 & 2.7e-05 & 0.0200 & 0.0410 & 0.500 & 0.710 & 5.1e-05 & 2.3e-05 & 0.0e+00 & 0.1216\\
Cellphone & Gemini-3.1-Flash-Lite-Preview & \texttt{obscene\_mean} & 0.683 & 8.5e-04 & 0.0087 & 0.0099 & 0.0200 & 0.0358 & 0.554 & 0.710 & 0.0053 & 0.0049 & 0.0e+00 & 0.1144\\
Cellphone & Gemini-3.1-Flash-Lite-Preview & \texttt{threat\_mean} & 0.817 & 0.0264 & 2.8e-04 & 4.3e-05 & 0.0800 & 0.0202 & 0.551 & 0.710 & 1.4e-04 & 5.8e-05 & 0.0e+00 & 0.1040\\
Cellphone & Gemini-3.1-Flash-Lite-Preview & \texttt{aggression\_score\_mean} & 1.7e-06 & 1.6e-05 & 0.0092 & 0.0069 & 0.100 & 0.417 & 0.541 & 0.710 & 0.0029 & 0.0025 & 0.0e+00 & 0.1168\\
Cellphone & Gemini-3.1-Flash-Lite-Preview & \texttt{length\_std} & 6.1e-11 & 4.4e-16 & 20.07 & 18.20 & 0.0e+00 & 0.571 & 0.491 & 0.475 & 9.183 & 7.239 & 0.0e+00 & 0.1192\\
Cellphone & Gemini-3.1-Flash-Lite-Preview & \texttt{length\_cv} & 5.2e-20 & 1.6e-37 & 0.591 & 0.577 & 0.0e+00 & 0.799 & 0.458 & 0.710 & 0.1211 & 0.1296 & 0.0e+00 & 0.1136\\
Cellphone & Gemini-3.1-Flash-Lite-Preview & \texttt{avg\_depth} & 1.7e-21 & 1.7e-31 & 0.938 & 0.892 & 0.0200 & 0.822 & 0.484 & 0.475 & 0.2115 & 0.2111 & 0.0e+00 & 0.1136\\
Cellphone & Gemini-3.1-Flash-Lite-Preview & \texttt{structural\_virality} & 2.3e-21 & 1.7e-31 & 1.840 & 1.784 & 0.0e+00 & 0.818 & 0.498 & 0.710 & 0.3649 & 0.3836 & 0.0e+00 & 0.1104\\
\midrule
Cellphone & DeepSeek-Chat & \texttt{self\_bleu\_4} & 4.3e-04 & 6.7e-04 & 0.0133 & 0.0138 & 0.0222 & 0.322 & 0.503 & 0.710 & 0.0089 & 0.0069 & 0.0e+00 & 0.1320\\
Cellphone & DeepSeek-Chat & \texttt{self\_bertscore\_mean\_f1} & 1.2e-14 & 1.8e-27 & 0.0960 & 0.141 & 0.733 & 0.705 & 0.475 & 0.710 & 0.0385 & 0.0382 & 0.0e+00 & 0.1200\\
Cellphone & DeepSeek-Chat & \texttt{semantic\_mean\_cosine} & 7.7e-16 & 1.3e-31 & 0.358 & 0.360 & 0.867 & 0.737 & 0.482 & 0.475 & 0.0389 & 0.0397 & 0.0e+00 & 0.1160\\
Cellphone & DeepSeek-Chat & \texttt{mean\_story\_probability} & 3.6e-18 & 3.1e-20 & 0.170 & 0.170 & 0.511 & 0.795 & 0.464 & 0.475 & 0.0433 & 0.0412 & 0.0e+00 & 0.1120\\
Cellphone & DeepSeek-Chat & \texttt{toxicity\_mean} & 0.0220 & 0.0299 & 0.0106 & 0.0115 & 0.0667 & 0.209 & 0.516 & 0.710 & 0.0084 & 0.0068 & 0.0e+00 & 0.1136\\
Cellphone & DeepSeek-Chat & \texttt{severe\_toxicity\_mean} & 0.0031 & 0.0033 & 8.4e-05 & 3.0e-05 & 0.0889 & 0.270 & 0.500 & 0.710 & 5.1e-05 & 2.3e-05 & 0.0e+00 & 0.1216\\
Cellphone & DeepSeek-Chat & \texttt{obscene\_mean} & 0.0295 & 0.0176 & 0.0096 & 0.0094 & 0.0e+00 & 0.199 & 0.554 & 0.710 & 0.0053 & 0.0049 & 0.0e+00 & 0.1144\\
Cellphone & DeepSeek-Chat & \texttt{threat\_mean} & 9.5e-04 & 0.0011 & 9.1e-04 & 5.5e-05 & 0.111 & 0.302 & 0.551 & 0.710 & 1.4e-04 & 5.8e-05 & 0.0e+00 & 0.1040\\
Cellphone & DeepSeek-Chat & \texttt{aggression\_score\_mean} & 0.0223 & 0.0125 & 0.0038 & 0.0043 & 0.0444 & 0.209 & 0.541 & 0.710 & 0.0029 & 0.0025 & 0.0e+00 & 0.1168\\
Cellphone & DeepSeek-Chat & \texttt{length\_std} & 0.157 & 0.0126 & 11.95 & 11.89 & 0.0444 & 0.129 & 0.491 & 0.475 & 9.183 & 7.239 & 0.0e+00 & 0.1192\\
Cellphone & DeepSeek-Chat & \texttt{length\_cv} & 1.7e-17 & 2.3e-24 & 0.536 & 0.548 & 0.0e+00 & 0.778 & 0.458 & 0.710 & 0.1211 & 0.1296 & 0.0e+00 & 0.1136\\
Cellphone & DeepSeek-Chat & \texttt{avg\_depth} & 1.5e-19 & 1.1e-28 & 0.918 & 0.892 & 0.0e+00 & 0.818 & 0.484 & 0.475 & 0.2115 & 0.2111 & 0.0e+00 & 0.1136\\
Cellphone & DeepSeek-Chat & \texttt{structural\_virality} & 1.4e-19 & 1.1e-28 & 1.840 & 1.784 & 0.0e+00 & 0.818 & 0.498 & 0.710 & 0.3649 & 0.3836 & 0.0e+00 & 0.1104\\
\midrule
Cellphone & DeepSeek-V4-Flash & \texttt{self\_bleu\_4} & 0.0080 & 0.0170 & 0.0083 & 0.0097 & 0.0200 & 0.231 & 0.503 & 0.710 & 0.0089 & 0.0069 & 0.0e+00 & 0.1320\\
Cellphone & DeepSeek-V4-Flash & \texttt{self\_bertscore\_mean\_f1} & 2.3e-20 & 4.8e-37 & 0.0836 & 0.0973 & 0.800 & 0.807 & 0.475 & 0.710 & 0.0385 & 0.0382 & 0.0e+00 & 0.1200\\
Cellphone & DeepSeek-V4-Flash & \texttt{semantic\_mean\_cosine} & 6.0e-22 & 1.9e-41 & 0.390 & 0.430 & 0.920 & 0.840 & 0.482 & 0.475 & 0.0389 & 0.0397 & 0.0e+00 & 0.1160\\
Cellphone & DeepSeek-V4-Flash & \texttt{mean\_story\_probability} & 5.1e-08 & 3.9e-08 & 0.105 & 0.0987 & 0.180 & 0.476 & 0.464 & 0.475 & 0.0433 & 0.0412 & 0.0e+00 & 0.1120\\
Cellphone & DeepSeek-V4-Flash & \texttt{toxicity\_mean} & 0.0481 & 0.0351 & 0.0125 & 0.0142 & 0.0200 & 0.173 & 0.516 & 0.710 & 0.0084 & 0.0068 & 0.0e+00 & 0.1136\\
Cellphone & DeepSeek-V4-Flash & \texttt{severe\_toxicity\_mean} & 0.0732 & 0.0037 & 8.3e-05 & 3.0e-05 & 0.0200 & 0.156 & 0.500 & 0.710 & 5.1e-05 & 2.3e-05 & 0.0e+00 & 0.1216\\
Cellphone & DeepSeek-V4-Flash & \texttt{obscene\_mean} & 0.157 & 4.5e-04 & 0.0094 & 0.0101 & 0.0200 & 0.124 & 0.554 & 0.710 & 0.0053 & 0.0049 & 0.0e+00 & 0.1144\\
Cellphone & DeepSeek-V4-Flash & \texttt{threat\_mean} & 7.4e-04 & 3.5e-06 & 2.6e-04 & 6.0e-05 & 0.0400 & 0.294 & 0.551 & 0.710 & 1.4e-04 & 5.8e-05 & 0.0e+00 & 0.1040\\
Cellphone & DeepSeek-V4-Flash & \texttt{aggression\_score\_mean} & 0.0428 & 0.0143 & 0.0046 & 0.0051 & 0.0200 & 0.177 & 0.541 & 0.710 & 0.0029 & 0.0025 & 0.0e+00 & 0.1168\\
Cellphone & DeepSeek-V4-Flash & \texttt{length\_std} & 1.4e-07 & 4.5e-09 & 24.24 & 22.37 & 0.180 & 0.459 & 0.491 & 0.475 & 9.183 & 7.239 & 0.0e+00 & 0.1192\\
Cellphone & DeepSeek-V4-Flash & \texttt{length\_cv} & 1.5e-18 & 8.6e-29 & 0.500 & 0.511 & 0.0e+00 & 0.767 & 0.458 & 0.710 & 0.1211 & 0.1296 & 0.0e+00 & 0.1136\\
Cellphone & DeepSeek-V4-Flash & \texttt{avg\_depth} & 1.7e-21 & 1.7e-31 & 0.938 & 0.892 & 0.0200 & 0.822 & 0.484 & 0.475 & 0.2115 & 0.2111 & 0.0e+00 & 0.1136\\
Cellphone & DeepSeek-V4-Flash & \texttt{structural\_virality} & 2.3e-21 & 1.7e-31 & 1.840 & 1.784 & 0.0e+00 & 0.818 & 0.498 & 0.710 & 0.3649 & 0.3836 & 0.0e+00 & 0.1104\\
\midrule
Camera & GPT-4o-mini & \texttt{self\_bleu\_4} & 3.4e-22 & 5.7e-44 & 0.0964 & 0.0996 & 0.933 & 0.859 & 0.547 & 0.710 & 0.0058 & 0.0046 & 0.0e+00 & 0.1208\\
Camera & GPT-4o-mini & \texttt{self\_bertscore\_mean\_f1} & 1.5e-22 & 2.8e-46 & 0.195 & 0.210 & 0.933 & 0.866 & 0.485 & 0.475 & 0.0300 & 0.0173 & 0.0e+00 & 0.0880\\
Camera & GPT-4o-mini & \texttt{semantic\_mean\_cosine} & 1.2e-22 & 8.6e-43 & 0.488 & 0.525 & 0.933 & 0.869 & 0.506 & 0.593 & 0.0411 & 0.0410 & 0.0e+00 & 0.0920\\
Camera & GPT-4o-mini & \texttt{mean\_story\_probability} & 1.8e-17 & 7.8e-23 & 0.103 & 0.101 & 0.0667 & 0.754 & 0.513 & 0.710 & 0.0300 & 0.0243 & 0.0e+00 & 0.1064\\
Camera & GPT-4o-mini & \texttt{toxicity\_mean} & 5.7e-07 & 1.3e-09 & 0.0241 & 0.0226 & 0.0444 & 0.444 & 0.482 & 0.710 & 0.0110 & 0.0081 & 0.0e+00 & 0.1136\\
Camera & GPT-4o-mini & \texttt{severe\_toxicity\_mean} & 1.0e-04 & 8.5e-08 & 1.1e-04 & 6.0e-05 & 0.0667 & 0.345 & 0.500 & 0.710 & 7.1e-05 & 3.7e-05 & 0.0200 & 0.1088\\
Camera & GPT-4o-mini & \texttt{obscene\_mean} & 3.6e-08 & 4.6e-09 & 0.0137 & 0.0117 & 0.0889 & 0.489 & 0.519 & 0.710 & 0.0072 & 0.0055 & 0.0e+00 & 0.1144\\
Camera & GPT-4o-mini & \texttt{threat\_mean} & 0.659 & 0.206 & 8.2e-04 & 4.3e-04 & 0.0667 & 0.0391 & 0.473 & 0.593 & 0.0011 & 4.8e-04 & 0.0e+00 & 0.1144\\
Camera & GPT-4o-mini & \texttt{aggression\_score\_mean} & 5.3e-07 & 1.0e-09 & 0.0081 & 0.0073 & 0.0444 & 0.445 & 0.577 & 0.710 & 0.0038 & 0.0028 & 0.0e+00 & 0.1088\\
Camera & GPT-4o-mini & \texttt{length\_std} & 1.4e-19 & 5.2e-32 & 36.00 & 33.13 & 0.0e+00 & 0.803 & 0.509 & 0.593 & 11.30 & 9.356 & 0.0e+00 & 0.1296\\
Camera & GPT-4o-mini & \texttt{length\_cv} & 6.0e-22 & 4.0e-42 & 0.655 & 0.661 & 0.0e+00 & 0.854 & 0.544 & 0.710 & 0.1186 & 0.1145 & 0.0e+00 & 0.1280\\
Camera & GPT-4o-mini & \texttt{avg\_depth} & 9.6e-22 & 1.6e-33 & 0.989 & 0.934 & 0.0222 & 0.846 & 0.462 & 0.475 & 0.2469 & 0.2245 & 0.0400 & 0.1144\\
Camera & GPT-4o-mini & \texttt{structural\_virality} & 1.3e-21 & 1.6e-33 & 1.841 & 1.789 & 0.0e+00 & 0.843 & 0.508 & 0.710 & 0.3730 & 0.4083 & 0.0400 & 0.1104\\
\midrule
Camera & GPT-5-mini & \texttt{self\_bleu\_4} & 1.2e-20 & 1.1e-31 & 0.0627 & 0.0635 & 0.795 & 0.835 & 0.547 & 0.710 & 0.0058 & 0.0046 & 0.0e+00 & 0.1208\\
Camera & GPT-5-mini & \texttt{self\_bertscore\_mean\_f1} & 6.8e-22 & 2.5e-44 & 0.128 & 0.136 & 0.932 & 0.862 & 0.485 & 0.475 & 0.0300 & 0.0173 & 0.0e+00 & 0.0880\\
Camera & GPT-5-mini & \texttt{semantic\_mean\_cosine} & 7.7e-22 & 5.1e-40 & 0.421 & 0.449 & 0.909 & 0.861 & 0.506 & 0.593 & 0.0411 & 0.0410 & 0.0e+00 & 0.0920\\
Camera & GPT-5-mini & \texttt{mean\_story\_probability} & 5.2e-25 & 6.4e-36 & 0.119 & 0.109 & 0.500 & 0.926 & 0.513 & 0.710 & 0.0300 & 0.0243 & 0.0e+00 & 0.1064\\
Camera & GPT-5-mini & \texttt{toxicity\_mean} & 8.3e-05 & 2.0e-08 & 0.0222 & 0.0221 & 0.0682 & 0.353 & 0.482 & 0.710 & 0.0110 & 0.0081 & 0.0e+00 & 0.1136\\
Camera & GPT-5-mini & \texttt{severe\_toxicity\_mean} & 0.0126 & 7.4e-06 & 1.1e-04 & 5.9e-05 & 0.0682 & 0.224 & 0.500 & 0.710 & 7.1e-05 & 3.7e-05 & 0.0200 & 0.1088\\
Camera & GPT-5-mini & \texttt{obscene\_mean} & 0.0028 & 7.6e-07 & 0.0121 & 0.0116 & 0.0682 & 0.268 & 0.519 & 0.710 & 0.0072 & 0.0055 & 0.0e+00 & 0.1144\\
Camera & GPT-5-mini & \texttt{threat\_mean} & 0.0061 & 0.0026 & 0.0013 & 5.9e-04 & 0.0682 & 0.246 & 0.473 & 0.593 & 0.0011 & 4.8e-04 & 0.0e+00 & 0.1144\\
Camera & GPT-5-mini & \texttt{aggression\_score\_mean} & 8.9e-05 & 4.3e-08 & 0.0075 & 0.0072 & 0.0682 & 0.351 & 0.577 & 0.710 & 0.0038 & 0.0028 & 0.0e+00 & 0.1088\\
Camera & GPT-5-mini & \texttt{length\_std} & 3.6e-06 & 8.9e-08 & 22.92 & 22.29 & 0.0455 & 0.415 & 0.509 & 0.593 & 11.30 & 9.356 & 0.0e+00 & 0.1296\\
Camera & GPT-5-mini & \texttt{length\_cv} & 7.7e-18 & 4.4e-23 & 0.491 & 0.499 & 0.0e+00 & 0.771 & 0.544 & 0.710 & 0.1186 & 0.1145 & 0.0e+00 & 0.1280\\
Camera & GPT-5-mini & \texttt{avg\_depth} & 1.2e-21 & 7.9e-33 & 1.035 & 0.934 & 0.0682 & 0.854 & 0.462 & 0.475 & 0.2469 & 0.2245 & 0.0400 & 0.1144\\
Camera & GPT-5-mini & \texttt{structural\_virality} & 3.5e-21 & 7.9e-33 & 1.841 & 1.789 & 0.0e+00 & 0.843 & 0.508 & 0.710 & 0.3730 & 0.4083 & 0.0400 & 0.1104\\
\midrule
Camera & Gemini-3.1-Flash-Lite-Preview & \texttt{self\_bleu\_4} & 4.0e-12 & 1.3e-19 & 0.0123 & 0.0100 & 0.0e+00 & 0.586 & 0.547 & 0.710 & 0.0058 & 0.0046 & 0.0e+00 & 0.1208\\
Camera & Gemini-3.1-Flash-Lite-Preview & \texttt{self\_bertscore\_mean\_f1} & 3.7e-29 & 2.2e-55 & 0.100 & 0.0849 & 0.940 & 0.946 & 0.485 & 0.475 & 0.0300 & 0.0173 & 0.0e+00 & 0.0880\\
Camera & Gemini-3.1-Flash-Lite-Preview & \texttt{semantic\_mean\_cosine} & 7.2e-22 & 5.0e-32 & 0.206 & 0.205 & 0.0800 & 0.811 & 0.506 & 0.593 & 0.0411 & 0.0410 & 0.0e+00 & 0.0920\\
Camera & Gemini-3.1-Flash-Lite-Preview & \texttt{mean\_story\_probability} & 7.5e-28 & 1.7e-34 & 0.118 & 0.109 & 0.580 & 0.924 & 0.513 & 0.710 & 0.0300 & 0.0243 & 0.0e+00 & 0.1064\\
Camera & Gemini-3.1-Flash-Lite-Preview & \texttt{toxicity\_mean} & 0.0503 & 0.0058 & 0.0080 & 0.0066 & 0.0600 & 0.165 & 0.482 & 0.710 & 0.0110 & 0.0081 & 0.0e+00 & 0.1136\\
Camera & Gemini-3.1-Flash-Lite-Preview & \texttt{severe\_toxicity\_mean} & 0.225 & 0.0046 & 8.8e-05 & 5.7e-05 & 0.0400 & 0.102 & 0.500 & 0.710 & 7.1e-05 & 3.7e-05 & 0.0200 & 0.1088\\
Camera & Gemini-3.1-Flash-Lite-Preview & \texttt{obscene\_mean} & 0.327 & 3.6e-04 & 0.0115 & 0.0109 & 0.0200 & 0.0828 & 0.519 & 0.710 & 0.0072 & 0.0055 & 0.0e+00 & 0.1144\\
Camera & Gemini-3.1-Flash-Lite-Preview & \texttt{threat\_mean} & 1.6e-04 & 6.6e-04 & 0.0015 & 0.0020 & 0.0800 & 0.319 & 0.473 & 0.593 & 0.0011 & 4.8e-04 & 0.0e+00 & 0.1144\\
Camera & Gemini-3.1-Flash-Lite-Preview & \texttt{aggression\_score\_mean} & 0.0746 & 0.0065 & 0.0023 & 0.0019 & 0.0400 & 0.151 & 0.577 & 0.710 & 0.0038 & 0.0028 & 0.0e+00 & 0.1088\\
Camera & Gemini-3.1-Flash-Lite-Preview & \texttt{length\_std} & 3.9e-07 & 4.7e-10 & 22.42 & 20.70 & 0.0e+00 & 0.428 & 0.509 & 0.593 & 11.30 & 9.356 & 0.0e+00 & 0.1296\\
Camera & Gemini-3.1-Flash-Lite-Preview & \texttt{length\_cv} & 1.5e-21 & 1.6e-36 & 0.529 & 0.513 & 0.0e+00 & 0.805 & 0.544 & 0.710 & 0.1186 & 0.1145 & 0.0e+00 & 0.1280\\
Camera & Gemini-3.1-Flash-Lite-Preview & \texttt{avg\_depth} & 7.7e-24 & 7.3e-37 & 0.986 & 0.934 & 0.0200 & 0.846 & 0.462 & 0.475 & 0.2469 & 0.2245 & 0.0400 & 0.1144\\
Camera & Gemini-3.1-Flash-Lite-Preview & \texttt{structural\_virality} & 1.1e-23 & 7.3e-37 & 1.841 & 1.789 & 0.0e+00 & 0.843 & 0.508 & 0.710 & 0.3730 & 0.4083 & 0.0400 & 0.1104\\
\midrule
Camera & DeepSeek-Chat & \texttt{self\_bleu\_4} & 9.8e-07 & 1.4e-09 & 0.0225 & 0.0215 & 0.120 & 0.413 & 0.547 & 0.710 & 0.0058 & 0.0046 & 0.0e+00 & 0.1208\\
Camera & DeepSeek-Chat & \texttt{self\_bertscore\_mean\_f1} & 1.5e-12 & 4.5e-28 & 0.128 & 0.155 & 0.700 & 0.598 & 0.485 & 0.475 & 0.0300 & 0.0173 & 0.0e+00 & 0.0880\\
Camera & DeepSeek-Chat & \texttt{semantic\_mean\_cosine} & 9.9e-13 & 2.6e-29 & 0.329 & 0.335 & 0.720 & 0.602 & 0.506 & 0.593 & 0.0411 & 0.0410 & 0.0e+00 & 0.0920\\
Camera & DeepSeek-Chat & \texttt{mean\_story\_probability} & 2.1e-18 & 4.5e-20 & 0.0963 & 0.0962 & 0.320 & 0.739 & 0.513 & 0.710 & 0.0300 & 0.0243 & 0.0e+00 & 0.1064\\
Camera & DeepSeek-Chat & \texttt{toxicity\_mean} & 0.0059 & 3.2e-04 & 0.0157 & 0.0130 & 0.120 & 0.232 & 0.482 & 0.710 & 0.0110 & 0.0081 & 0.0e+00 & 0.1136\\
Camera & DeepSeek-Chat & \texttt{severe\_toxicity\_mean} & 0.0021 & 2.7e-06 & 1.1e-04 & 6.0e-05 & 0.120 & 0.260 & 0.500 & 0.710 & 7.1e-05 & 3.7e-05 & 0.0200 & 0.1088\\
Camera & DeepSeek-Chat & \texttt{obscene\_mean} & 0.0023 & 5.5e-07 & 0.0129 & 0.0114 & 0.120 & 0.257 & 0.519 & 0.710 & 0.0072 & 0.0055 & 0.0e+00 & 0.1144\\
Camera & DeepSeek-Chat & \texttt{threat\_mean} & 0.0404 & 0.0053 & 8.6e-04 & 5.5e-04 & 0.140 & 0.173 & 0.473 & 0.593 & 0.0011 & 4.8e-04 & 0.0e+00 & 0.1144\\
Camera & DeepSeek-Chat & \texttt{aggression\_score\_mean} & 0.0034 & 4.3e-04 & 0.0058 & 0.0047 & 0.120 & 0.247 & 0.577 & 0.710 & 0.0038 & 0.0028 & 0.0e+00 & 0.1088\\
Camera & DeepSeek-Chat & \texttt{length\_std} & 0.0973 & 0.0343 & 11.73 & 8.514 & 0.0e+00 & 0.140 & 0.509 & 0.593 & 11.30 & 9.356 & 0.0e+00 & 0.1296\\
Camera & DeepSeek-Chat & \texttt{length\_cv} & 1.9e-22 & 1.8e-33 & 0.569 & 0.579 & 0.0e+00 & 0.823 & 0.544 & 0.710 & 0.1186 & 0.1145 & 0.0e+00 & 0.1280\\
Camera & DeepSeek-Chat & \texttt{avg\_depth} & 1.2e-24 & 7.3e-37 & 1.086 & 1.134 & 0.120 & 0.862 & 0.462 & 0.475 & 0.2469 & 0.2245 & 0.0400 & 0.1144\\
Camera & DeepSeek-Chat & \texttt{structural\_virality} & 1.1e-23 & 7.3e-37 & 1.841 & 1.789 & 0.0e+00 & 0.843 & 0.508 & 0.710 & 0.3730 & 0.4083 & 0.0400 & 0.1104\\
\midrule
Camera & DeepSeek-V4-Flash & \texttt{self\_bleu\_4} & 2.4e-09 & 5.0e-11 & 0.0204 & 0.0140 & 0.100 & 0.504 & 0.547 & 0.710 & 0.0058 & 0.0046 & 0.0e+00 & 0.1208\\
Camera & DeepSeek-V4-Flash & \texttt{self\_bertscore\_mean\_f1} & 2.1e-24 & 9.6e-41 & 0.0812 & 0.0839 & 0.840 & 0.860 & 0.485 & 0.475 & 0.0300 & 0.0173 & 0.0e+00 & 0.0880\\
Camera & DeepSeek-V4-Flash & \texttt{semantic\_mean\_cosine} & 5.5e-24 & 1.0e-42 & 0.341 & 0.358 & 0.620 & 0.853 & 0.506 & 0.593 & 0.0411 & 0.0410 & 0.0e+00 & 0.0920\\
Camera & DeepSeek-V4-Flash & \texttt{mean\_story\_probability} & 2.0e-07 & 8.3e-06 & 0.0612 & 0.0583 & 0.120 & 0.439 & 0.513 & 0.710 & 0.0300 & 0.0243 & 0.0e+00 & 0.1064\\
Camera & DeepSeek-V4-Flash & \texttt{toxicity\_mean} & 0.364 & 0.100 & 0.0187 & 0.0103 & 0.0600 & 0.0766 & 0.482 & 0.710 & 0.0110 & 0.0081 & 0.0e+00 & 0.1136\\
Camera & DeepSeek-V4-Flash & \texttt{severe\_toxicity\_mean} & 0.296 & 0.0057 & 9.0e-05 & 5.2e-05 & 0.0200 & 0.0882 & 0.500 & 0.710 & 7.1e-05 & 3.7e-05 & 0.0200 & 0.1088\\
Camera & DeepSeek-V4-Flash & \texttt{obscene\_mean} & 0.312 & 0.0011 & 0.0087 & 0.0091 & 0.0600 & 0.0853 & 0.519 & 0.710 & 0.0072 & 0.0055 & 0.0e+00 & 0.1144\\
Camera & DeepSeek-V4-Flash & \texttt{threat\_mean} & 0.766 & 0.0495 & 0.0012 & 4.9e-04 & 0.0200 & 0.0252 & 0.473 & 0.593 & 0.0011 & 4.8e-04 & 0.0e+00 & 0.1144\\
Camera & DeepSeek-V4-Flash & \texttt{aggression\_score\_mean} & 0.300 & 0.0598 & 0.0060 & 0.0025 & 0.0600 & 0.0876 & 0.577 & 0.710 & 0.0038 & 0.0028 & 0.0e+00 & 0.1088\\
Camera & DeepSeek-V4-Flash & \texttt{length\_std} & 0.0443 & 2.6e-04 & 12.32 & 9.013 & 0.0e+00 & 0.170 & 0.509 & 0.593 & 11.30 & 9.356 & 0.0e+00 & 0.1296\\
Camera & DeepSeek-V4-Flash & \texttt{length\_cv} & 1.9e-19 & 1.3e-25 & 0.481 & 0.489 & 0.0e+00 & 0.761 & 0.544 & 0.710 & 0.1186 & 0.1145 & 0.0e+00 & 0.1280\\
Camera & DeepSeek-V4-Flash & \texttt{avg\_depth} & 7.7e-24 & 7.3e-37 & 0.986 & 0.934 & 0.0200 & 0.846 & 0.462 & 0.475 & 0.2469 & 0.2245 & 0.0400 & 0.1144\\
Camera & DeepSeek-V4-Flash & \texttt{structural\_virality} & 1.1e-23 & 7.3e-37 & 1.841 & 1.789 & 0.0e+00 & 0.843 & 0.508 & 0.710 & 0.3730 & 0.4083 & 0.0400 & 0.1104\\
\midrule
Headphones & GPT-4o-mini & \texttt{self\_bleu\_4} & 1.6e-21 & 1.1e-33 & 0.0811 & 0.0851 & 0.651 & 0.908 & 0.469 & 0.710 & 0.0086 & 0.0070 & 0.0400 & 0.1168\\
Headphones & GPT-4o-mini & \texttt{self\_bertscore\_mean\_f1} & 1.1e-23 & 2.0e-46 & 0.239 & 0.293 & 0.977 & 0.956 & 0.473 & 0.710 & 0.0374 & 0.0556 & 0.0e+00 & 0.1080\\
Headphones & GPT-4o-mini & \texttt{semantic\_mean\_cosine} & 1.2e-23 & 1.7e-45 & 0.546 & 0.573 & 0.977 & 0.956 & 0.531 & 0.710 & 0.0412 & 0.0448 & 0.0e+00 & 0.1056\\
Headphones & GPT-4o-mini & \texttt{mean\_story\_probability} & 1.8e-18 & 5.2e-20 & 0.191 & 0.181 & 0.349 & 0.836 & 0.548 & 0.475 & 0.0466 & 0.0439 & 0.0400 & 0.1136\\
Headphones & GPT-4o-mini & \texttt{toxicity\_mean} & 1.4e-15 & 6.6e-19 & 0.0385 & 0.0339 & 0.0930 & 0.761 & 0.473 & 0.710 & 0.0150 & 0.0114 & 0.0400 & 0.1104\\
Headphones & GPT-4o-mini & \texttt{severe\_toxicity\_mean} & 2.7e-16 & 5.5e-22 & 3.0e-04 & 1.5e-04 & 0.140 & 0.781 & 0.449 & 0.475 & 2.0e-04 & 1.1e-04 & 0.0400 & 0.1104\\
Headphones & GPT-4o-mini & \texttt{obscene\_mean} & 7.4e-16 & 9.7e-18 & 0.0183 & 0.0167 & 0.0698 & 0.769 & 0.522 & 0.710 & 0.0093 & 0.0070 & 0.0e+00 & 0.1248\\
Headphones & GPT-4o-mini & \texttt{threat\_mean} & 6.3e-14 & 1.8e-19 & 0.0013 & 3.2e-04 & 0.0465 & 0.715 & 0.479 & 0.710 & 0.0012 & 4.1e-04 & 0.0400 & 0.1096\\
Headphones & GPT-4o-mini & \texttt{aggression\_score\_mean} & 6.5e-15 & 1.1e-18 & 0.0128 & 0.0116 & 0.0930 & 0.743 & 0.548 & 0.710 & 0.0053 & 0.0039 & 0.0400 & 0.1120\\
Headphones & GPT-4o-mini & \texttt{length\_std} & 1.0e-10 & 1.7e-18 & 21.38 & 19.54 & 0.0e+00 & 0.616 & 0.485 & 0.710 & 8.059 & 6.760 & 0.0e+00 & 0.1232\\
Headphones & GPT-4o-mini & \texttt{length\_cv} & 1.1e-14 & 2.4e-29 & 0.632 & 0.608 & 0.0e+00 & 0.736 & 0.528 & 0.710 & 0.1355 & 0.1417 & 0.0e+00 & 0.1168\\
Headphones & GPT-4o-mini & \texttt{avg\_depth} & 2.1e-17 & 1.7e-24 & 0.863 & 0.828 & 0.0e+00 & 0.796 & 0.474 & 0.710 & 0.2175 & 0.1864 & 0.0e+00 & 0.1120\\
Headphones & GPT-4o-mini & \texttt{structural\_virality} & 2.0e-17 & 1.7e-24 & 1.706 & 1.674 & 0.0e+00 & 0.796 & 0.451 & 0.710 & 0.3645 & 0.3563 & 0.0e+00 & 0.1096\\
\midrule
Headphones & GPT-5-mini & \texttt{self\_bleu\_4} & 7.3e-08 & 4.5e-10 & 0.0284 & 0.0263 & 0.209 & 0.513 & 0.469 & 0.710 & 0.0086 & 0.0070 & 0.0400 & 0.1168\\
Headphones & GPT-5-mini & \texttt{self\_bertscore\_mean\_f1} & 8.7e-13 & 5.3e-26 & 0.125 & 0.102 & 0.837 & 0.681 & 0.473 & 0.710 & 0.0374 & 0.0556 & 0.0e+00 & 0.1080\\
Headphones & GPT-5-mini & \texttt{semantic\_mean\_cosine} & 4.4e-13 & 2.6e-26 & 0.384 & 0.368 & 0.837 & 0.690 & 0.531 & 0.710 & 0.0412 & 0.0448 & 0.0e+00 & 0.1056\\
Headphones & GPT-5-mini & \texttt{mean\_story\_probability} & 1.6e-17 & 2.5e-19 & 0.181 & 0.186 & 0.488 & 0.812 & 0.548 & 0.475 & 0.0466 & 0.0439 & 0.0400 & 0.1136\\
Headphones & GPT-5-mini & \texttt{toxicity\_mean} & 2.1e-05 & 4.6e-05 & 0.0283 & 0.0263 & 0.163 & 0.406 & 0.473 & 0.710 & 0.0150 & 0.0114 & 0.0400 & 0.1104\\
Headphones & GPT-5-mini & \texttt{severe\_toxicity\_mean} & 1.1e-05 & 1.4e-07 & 3.0e-04 & 1.4e-04 & 0.163 & 0.420 & 0.449 & 0.475 & 2.0e-04 & 1.1e-04 & 0.0400 & 0.1104\\
Headphones & GPT-5-mini & \texttt{obscene\_mean} & 7.7e-05 & 7.7e-06 & 0.0153 & 0.0166 & 0.163 & 0.377 & 0.522 & 0.710 & 0.0093 & 0.0070 & 0.0e+00 & 0.1248\\
Headphones & GPT-5-mini & \texttt{threat\_mean} & 5.9e-08 & 8.5e-10 & 0.0012 & 3.2e-04 & 0.163 & 0.517 & 0.479 & 0.710 & 0.0012 & 4.1e-04 & 0.0400 & 0.1096\\
Headphones & GPT-5-mini & \texttt{aggression\_score\_mean} & 2.3e-05 & 4.9e-05 & 0.0096 & 0.0092 & 0.163 & 0.404 & 0.548 & 0.710 & 0.0053 & 0.0039 & 0.0400 & 0.1120\\
Headphones & GPT-5-mini & \texttt{length\_std} & 2.5e-07 & 8.9e-10 & 30.33 & 29.80 & 0.326 & 0.491 & 0.485 & 0.710 & 8.059 & 6.760 & 0.0e+00 & 0.1232\\
Headphones & GPT-5-mini & \texttt{length\_cv} & 3.2e-11 & 2.6e-14 & 0.425 & 0.384 & 0.0e+00 & 0.632 & 0.528 & 0.710 & 0.1355 & 0.1417 & 0.0e+00 & 0.1168\\
Headphones & GPT-5-mini & \texttt{avg\_depth} & 1.2e-18 & 1.7e-24 & 1.026 & 1.028 & 0.163 & 0.829 & 0.474 & 0.710 & 0.2175 & 0.1864 & 0.0e+00 & 0.1120\\
Headphones & GPT-5-mini & \texttt{structural\_virality} & 2.0e-17 & 1.7e-24 & 1.706 & 1.674 & 0.0e+00 & 0.796 & 0.451 & 0.710 & 0.3645 & 0.3563 & 0.0e+00 & 0.1096\\
\midrule
Headphones & Gemini-3.1-Flash-Lite-Preview & \texttt{self\_bleu\_4} & 0.0166 & 2.6e-05 & 0.0129 & 0.0134 & 0.0e+00 & 0.241 & 0.469 & 0.710 & 0.0086 & 0.0070 & 0.0400 & 0.1168\\
Headphones & Gemini-3.1-Flash-Lite-Preview & \texttt{self\_bertscore\_mean\_f1} & 2.8e-20 & 2.9e-37 & 0.134 & 0.187 & 0.974 & 0.927 & 0.473 & 0.710 & 0.0374 & 0.0556 & 0.0e+00 & 0.1080\\
Headphones & Gemini-3.1-Flash-Lite-Preview & \texttt{semantic\_mean\_cosine} & 1.8e-19 & 8.0e-31 & 0.300 & 0.322 & 0.816 & 0.908 & 0.531 & 0.710 & 0.0412 & 0.0448 & 0.0e+00 & 0.1056\\
Headphones & Gemini-3.1-Flash-Lite-Preview & \texttt{mean\_story\_probability} & 9.1e-23 & 4.3e-36 & 0.208 & 0.197 & 0.947 & 0.988 & 0.548 & 0.475 & 0.0466 & 0.0439 & 0.0400 & 0.1136\\
Headphones & Gemini-3.1-Flash-Lite-Preview & \texttt{toxicity\_mean} & 1.4e-05 & 5.2e-06 & 0.0335 & 0.0290 & 0.0263 & 0.437 & 0.473 & 0.710 & 0.0150 & 0.0114 & 0.0400 & 0.1104\\
Headphones & Gemini-3.1-Flash-Lite-Preview & \texttt{severe\_toxicity\_mean} & 0.325 & 2.2e-04 & 3.0e-04 & 1.4e-04 & 0.0263 & 0.0991 & 0.449 & 0.475 & 2.0e-04 & 1.1e-04 & 0.0400 & 0.1104\\
Headphones & Gemini-3.1-Flash-Lite-Preview & \texttt{obscene\_mean} & 0.525 & 3.1e-04 & 0.0142 & 0.0137 & 0.0263 & 0.0640 & 0.522 & 0.710 & 0.0093 & 0.0070 & 0.0e+00 & 0.1248\\
Headphones & Gemini-3.1-Flash-Lite-Preview & \texttt{threat\_mean} & 0.477 & 0.0517 & 0.0012 & 2.6e-04 & 0.0263 & 0.0716 & 0.479 & 0.710 & 0.0012 & 4.1e-04 & 0.0400 & 0.1096\\
Headphones & Gemini-3.1-Flash-Lite-Preview & \texttt{aggression\_score\_mean} & 4.9e-05 & 5.2e-06 & 0.0099 & 0.0079 & 0.0263 & 0.408 & 0.548 & 0.710 & 0.0053 & 0.0039 & 0.0400 & 0.1120\\
Headphones & Gemini-3.1-Flash-Lite-Preview & \texttt{length\_std} & 0.321 & 0.0079 & 11.94 & 11.18 & 0.0e+00 & 0.0999 & 0.485 & 0.710 & 8.059 & 6.760 & 0.0e+00 & 0.1232\\
Headphones & Gemini-3.1-Flash-Lite-Preview & \texttt{length\_cv} & 3.3e-12 & 5.3e-23 & 0.531 & 0.524 & 0.0e+00 & 0.700 & 0.528 & 0.710 & 0.1355 & 0.1417 & 0.0e+00 & 0.1168\\
Headphones & Gemini-3.1-Flash-Lite-Preview & \texttt{avg\_depth} & 6.3e-16 & 3.4e-22 & 0.890 & 0.828 & 0.0263 & 0.801 & 0.474 & 0.710 & 0.2175 & 0.1864 & 0.0e+00 & 0.1120\\
Headphones & Gemini-3.1-Flash-Lite-Preview & \texttt{structural\_virality} & 9.2e-16 & 3.4e-22 & 1.706 & 1.674 & 0.0e+00 & 0.796 & 0.451 & 0.710 & 0.3645 & 0.3563 & 0.0e+00 & 0.1096\\
\midrule
Headphones & DeepSeek-Chat & \texttt{self\_bleu\_4} & 7.6e-04 & 5.0e-04 & 0.0118 & 0.0128 & 0.0526 & 0.338 & 0.469 & 0.710 & 0.0086 & 0.0070 & 0.0400 & 0.1168\\
Headphones & DeepSeek-Chat & \texttt{self\_bertscore\_mean\_f1} & 5.7e-18 & 1.3e-28 & 0.109 & 0.176 & 0.842 & 0.868 & 0.473 & 0.710 & 0.0374 & 0.0556 & 0.0e+00 & 0.1080\\
Headphones & DeepSeek-Chat & \texttt{semantic\_mean\_cosine} & 5.6e-19 & 9.6e-32 & 0.435 & 0.481 & 0.921 & 0.895 & 0.531 & 0.710 & 0.0412 & 0.0448 & 0.0e+00 & 0.1056\\
Headphones & DeepSeek-Chat & \texttt{mean\_story\_probability} & 2.8e-09 & 5.1e-08 & 0.136 & 0.127 & 0.368 & 0.598 & 0.548 & 0.475 & 0.0466 & 0.0439 & 0.0400 & 0.1136\\
Headphones & DeepSeek-Chat & \texttt{toxicity\_mean} & 0.373 & 0.259 & 0.0161 & 0.0122 & 0.0263 & 0.0898 & 0.473 & 0.710 & 0.0150 & 0.0114 & 0.0400 & 0.1104\\
Headphones & DeepSeek-Chat & \texttt{severe\_toxicity\_mean} & 0.0494 & 0.0025 & 3.0e-04 & 1.4e-04 & 0.0263 & 0.198 & 0.449 & 0.475 & 2.0e-04 & 1.1e-04 & 0.0400 & 0.1104\\
Headphones & DeepSeek-Chat & \texttt{obscene\_mean} & 0.328 & 0.0215 & 0.0123 & 0.0138 & 0.0263 & 0.0985 & 0.522 & 0.710 & 0.0093 & 0.0070 & 0.0e+00 & 0.1248\\
Headphones & DeepSeek-Chat & \texttt{threat\_mean} & 0.0161 & 0.0021 & 0.0012 & 2.8e-04 & 0.0263 & 0.242 & 0.479 & 0.710 & 0.0012 & 4.1e-04 & 0.0400 & 0.1096\\
Headphones & DeepSeek-Chat & \texttt{aggression\_score\_mean} & 0.334 & 0.177 & 0.0059 & 0.0051 & 0.0263 & 0.0972 & 0.548 & 0.710 & 0.0053 & 0.0039 & 0.0400 & 0.1120\\
Headphones & DeepSeek-Chat & \texttt{length\_std} & 3.2e-04 & 6.4e-04 & 17.43 & 18.04 & 0.0789 & 0.362 & 0.485 & 0.710 & 8.059 & 6.760 & 0.0e+00 & 0.1232\\
Headphones & DeepSeek-Chat & \texttt{length\_cv} & 3.8e-10 & 1.0e-13 & 0.439 & 0.442 & 0.0e+00 & 0.629 & 0.528 & 0.710 & 0.1355 & 0.1417 & 0.0e+00 & 0.1168\\
Headphones & DeepSeek-Chat & \texttt{avg\_depth} & 6.3e-16 & 3.4e-22 & 0.890 & 0.828 & 0.0263 & 0.801 & 0.474 & 0.710 & 0.2175 & 0.1864 & 0.0e+00 & 0.1120\\
Headphones & DeepSeek-Chat & \texttt{structural\_virality} & 9.2e-16 & 3.4e-22 & 1.706 & 1.674 & 0.0e+00 & 0.796 & 0.451 & 0.710 & 0.3645 & 0.3563 & 0.0e+00 & 0.1096\\
\midrule
Headphones & DeepSeek-V4-Flash & \texttt{self\_bleu\_4} & 0.583 & 0.688 & 0.0058 & 0.0019 & 0.0e+00 & 0.0553 & 0.469 & 0.710 & 0.0086 & 0.0070 & 0.0400 & 0.1168\\
Headphones & DeepSeek-V4-Flash & \texttt{self\_bertscore\_mean\_f1} & 2.0e-12 & 3.5e-21 & 0.0799 & 0.0677 & 0.763 & 0.707 & 0.473 & 0.710 & 0.0374 & 0.0556 & 0.0e+00 & 0.1080\\
Headphones & DeepSeek-V4-Flash & \texttt{semantic\_mean\_cosine} & 9.6e-14 & 6.9e-26 & 0.383 & 0.353 & 0.868 & 0.748 & 0.531 & 0.710 & 0.0412 & 0.0448 & 0.0e+00 & 0.1056\\
Headphones & DeepSeek-V4-Flash & \texttt{mean\_story\_probability} & 2.0e-05 & 7.4e-07 & 0.109 & 0.0917 & 0.105 & 0.429 & 0.548 & 0.475 & 0.0466 & 0.0439 & 0.0400 & 0.1136\\
Headphones & DeepSeek-V4-Flash & \texttt{toxicity\_mean} & 0.232 & 0.0202 & 0.0226 & 0.0122 & 0.0789 & 0.120 & 0.473 & 0.710 & 0.0150 & 0.0114 & 0.0400 & 0.1104\\
Headphones & DeepSeek-V4-Flash & \texttt{severe\_toxicity\_mean} & 0.1000 & 0.0084 & 2.8e-04 & 1.4e-04 & 0.0526 & 0.166 & 0.449 & 0.475 & 2.0e-04 & 1.1e-04 & 0.0400 & 0.1104\\
Headphones & DeepSeek-V4-Flash & \texttt{obscene\_mean} & 0.551 & 0.0251 & 0.0104 & 0.0108 & 0.0789 & 0.0601 & 0.522 & 0.710 & 0.0093 & 0.0070 & 0.0e+00 & 0.1248\\
Headphones & DeepSeek-V4-Flash & \texttt{threat\_mean} & 0.0317 & 0.0058 & 0.0012 & 2.8e-04 & 0.0526 & 0.216 & 0.479 & 0.710 & 0.0012 & 4.1e-04 & 0.0400 & 0.1096\\
Headphones & DeepSeek-V4-Flash & \texttt{aggression\_score\_mean} & 0.218 & 0.0191 & 0.0071 & 0.0055 & 0.132 & 0.124 & 0.548 & 0.710 & 0.0053 & 0.0039 & 0.0400 & 0.1120\\
Headphones & DeepSeek-V4-Flash & \texttt{length\_std} & 0.0023 & 0.0011 & 19.66 & 18.20 & 0.211 & 0.306 & 0.485 & 0.710 & 8.059 & 6.760 & 0.0e+00 & 0.1232\\
Headphones & DeepSeek-V4-Flash & \texttt{length\_cv} & 2.7e-11 & 3.0e-15 & 0.481 & 0.440 & 0.0e+00 & 0.669 & 0.528 & 0.710 & 0.1355 & 0.1417 & 0.0e+00 & 0.1168\\
Headphones & DeepSeek-V4-Flash & \texttt{avg\_depth} & 4.2e-16 & 3.4e-22 & 0.916 & 0.828 & 0.0526 & 0.807 & 0.474 & 0.710 & 0.2175 & 0.1864 & 0.0e+00 & 0.1120\\
Headphones & DeepSeek-V4-Flash & \texttt{structural\_virality} & 9.2e-16 & 3.4e-22 & 1.706 & 1.674 & 0.0e+00 & 0.796 & 0.451 & 0.710 & 0.3645 & 0.3563 & 0.0e+00 & 0.1096\\
\end{longtable}
}
\end{landscape}
