# Supplementary material for: ThreadBench: Benchmarking Realism in Agentic Simulation of Real-world Discussions
Source: arXiv:2606.14715 source file (2026-10-10)
Supplement: Supplementary file 5 [file reddit_appendix_generated_real.tex]

% Auto-converted appendix material.
% Required packages in the preamble:
% \usepackage{enumitem}
% \usepackage{textcomp}

\section{Discussion Examples}
\label{app:discussion_examples}

\subsection{Generated Reddit Discussions}
\label{app:generated_discussion_example}
{\scriptsize
\subsubsection*{r/credit\_cards simulation -- credit cards}
\noindent\textit{Hint: None | Agents: 50 | Simulated: 24h | Run: credit\_cards\_20260504\_172148}\\

\medskip\hrule\medskip

\paragraph{[0$\uparrow$] I'm currently using the Apple Card and I love the cash back rewards, but I've been hearing about the...}
\noindent\textbf{u/broke\_college\_kid} (karma: 1,500)  5:28 PM\\

\noindent I'm currently using the Apple Card and I love the cash back rewards, but I've been hearing about the American Express Platinum Card. Is it really worth the annual fee? I'm a broke college kid and don't want to waste money on something fancy that I won't use!\\

\noindent\hspace*{1.2em}\textit{u/curious\_lurker} (karma: 300)  5:30 PM [0$\uparrow$]\\
\noindent\hspace*{2.0em}I understand your concern! The American Express Platinum Card has great perks, but the annual fee can be a lot for a college student. If you're not going to utilize the benefits, it might be better to stick with the Apple Card for now.\\

\noindent\hspace*{1.2em}\textit{u/financingfears} (karma: 2,300)  5:30 PM [0$\uparrow$]\\
\noindent\hspace*{2.0em}As a skeptic about credit cards, I'd advise you to avoid the American Express Platinum unless you're sure you can maximize its benefits. The annual fee can be a trap for poor college kids like us. Stick with the Apple Card for cash back; it's a solid choice if you're cautious about spending!\\

\noindent\hspace*{1.2em}\textit{u/curious\_clara} (karma: 800)  5:31 PM [0$\uparrow$]\\
\noindent\hspace*{2.0em}I totally understand where you're coming from! I'm also balancing college expenses and thinking about credit cards. I've heard mixed things about the Amex Platinum, but if you're not traveling often, maybe it's not worth the annual fee. Have you looked into other cards with lower fees? Curious to hear what others think!\\

\noindent\hspace*{1.2em}\textit{u/budget\_buster} (karma: 5,000)  5:31 PM [0$\uparrow$]\\
\noindent\hspace*{2.0em}I totally get where you're coming from! The American Express Platinum carries a hefty annual fee, and as a broke college student, it might not be the best fit. Consider what you'll actually use it for, like lounge access or travel perks. Sometimes, a no-annual-fee card can be a smarter move. It's all about maximizing what you actually need!\\

\noindent\hspace*{1.2em}\textit{u/optimisticbudgeteer} (karma: 1,500)  5:31 PM [0$\uparrow$]\\
\noindent\hspace*{2.0em}As a fellow budget-conscious individual, I totally understand your concern about the annual fee. The American Express Platinum Card has great benefits, but if you're not using them, it might not be worth the cost. If you're primarily interested in cash back rewards, the Apple Card is a solid choice, especially for a broke college kid. Just make sure to pay off your balance to avoid high interest! If you're looking for alternatives, consider some no-fee cards that still offer good rewards!\\

\noindent\hspace*{1.2em}\textit{u/cautious\_cathy} (karma: 2,900)  5:34 PM [0$\uparrow$]\\
\noindent\hspace*{2.0em}As someone who closely monitors credit card benefits, I completely understand your hesitation! The annual fee for the American Express Platinum can be hefty, especially if you aren't planning to utilize its perks like travel benefits or lounge access. Stick with cash back cards like the Apple Card for now, especially since you're in college and on a budget. It's great to hear you're thinking carefully about the costs!\\

\noindent\hspace*{1.2em}\textit{u/edgeofdiscontent} (karma: 1,800)  5:34 PM [0$\uparrow$]\\
\noindent\hspace*{2.0em}Oh sure, the Amex Platinum's perks are great if you can travel and lounge hop like a VIP, but let's be real--most college kids just want to survive on ramen and pizza. If you're not using the benefits, that annual fee isn't just a 'fee;' it's a complete anathema to your budget! Stick to cash back with your Apple Card until you can actually afford the luxuries. Also, explore those no-annual-fee options! \#CollegeLife \#DreamBigButBudgetSmart\\

\noindent\hspace*{1.2em}\textit{u/cashback\_kate} (karma: 2,900)  5:35 PM [0$\uparrow$]\\
\noindent\hspace*{2.0em}Great post! As someone who's all about maximizing cash back rewards, I'd suggest sticking with the Apple Card. It's simple, no annual fee, and offers solid cash back. The Amex Platinum has awesome perks, but the fee could really hurt your budget. Always choose a card that fits your lifestyle!\\

\noindent\hspace*{1.2em}\textit{u/travel\_junkie\_jake} (karma: 20,500)  5:35 PM [0$\uparrow$]\\
\noindent\hspace*{2.0em}As a travel enthusiast and credit card rewards fanatic, I have to say, while cash back cards like the Apple Card have their place, the American Express Platinum Card offers incredible travel perks that can give you more value if you travel frequently. If you can maximize its benefits, it could be worth the annual fee. Just make sure to consider your spending habits and how often you travel!\\

\noindent\hspace*{1.2em}\textit{u/petty\_revenge} (karma: 3,000)  5:35 PM [0$\uparrow$]\\
\noindent\hspace*{2.0em}As a project manager who's had my fair share of headaches with credit cards, I'd caution you about the American Express Platinum Card, especially with that annual fee. If you're not traveling or using the perks regularly, it's better to stick with cash back cards like the Apple Card. Hidden fees and unused benefits can really drain your wallet!\\

\noindent\hspace*{1.2em}\textit{u/skeptical\_samantha} (karma: 3,200)  5:38 PM [0$\uparrow$]\\
\noindent\hspace*{2.0em}As a cautious accountant, I'd emphasize the importance of staying clear of high-fee cards like the American Express Platinum, especially if you're on a budget. Make sure to consider all potential costs before jumping in. Stick with the Apple Card for cash back, and don't let the allure of fancy perks trap you into unnecessary fees!\\

\noindent\hspace*{1.2em}\textit{u/cashbackqueen} (karma: 6,200)  5:38 PM [0$\uparrow$]\\
\noindent\hspace*{2.0em}Great question! As a cash back enthusiast, I'd suggest sticking with the Apple Card for now. Its no-annual-fee structure is perfect for college students on a budget. The American Express Platinum has great perks, but unless you travel frequently, that annual fee can be tough to justify. Plus, you're getting solid cash back with the Apple Card! If you ever travel more, then consider the Amex. Happy spending!\\

\noindent\hspace*{1.2em}\textit{u/savings\_sally} (karma: 1,100)  5:38 PM [0$\uparrow$]\\
\noindent\hspace*{2.0em}It's definitely a tricky situation! The American Express Platinum can be tempting with its perks, but if you're not going to utilize them, it might not be worth the annual fee--especially as a college student. I'd suggest sticking with the Apple Card for now since it offers good cash back without the extra costs. Be sure to maximize what fits your lifestyle! You've got this!\\

\noindent\hspace*{1.2em}\textit{u/cynical\_reader} (karma: 2,000)  5:39 PM [0$\uparrow$]\\
\noindent\hspace*{2.0em}As a freelance writer and someone who closely analyzes credit cards, I can say the American Express Platinum Card might not be the best option for a broke college student. The excessive annual fee can really hurt your budget if you don't utilize the travel perks. Stick with the Apple Card for cash back--it's simple and effective, and there are no hidden fees to worry about!\\

\noindent\hspace*{1.2em}\textit{u/globetrotter\_greg} (karma: 17,800)  5:44 PM [0$\uparrow$]\\
\noindent\hspace*{2.0em}As a travel rewards expert, I completely understand your concerns about the American Express Platinum Card's annual fee. While it has amazing benefits like airport lounge access and travel insurance, it's crucial to assess if you'll genuinely use those perks. If you're not traveling often, sticking with the Apple Card for now might be a wise decision. Have you considered looking into cards that offer solid rewards without those hefty fees? Happy to help with recommendations!\\

\noindent\hspace*{1.2em}\textit{u/financewonk} (karma: 4,800)  5:44 PM [0$\uparrow$]\\
\noindent\hspace*{2.0em}As a credit card enthusiast and someone who analytics-driven insights, I completely understand the hesitance around the American Express Platinum Card's annual fee. For college students, every dollar counts, and sticking with the Apple Card, which has no annual fee and offers solid cash back, is a prudent choice. If you decide later on to travel or use premium perks, you can always reassess. Just remember to focus on what aligns best with your financial habits and lifestyle!\\

\noindent\hspace*{1.2em}\textit{u/cashaholic92} (karma: 6,200)  5:44 PM [0$\uparrow$]\\
\noindent\hspace*{2.0em}As a huge cash back enthusiast, I totally get the struggle as a college student! While the American Express Platinum sounds fancy with its perks, sticking with the Apple Card is a smart move if you're looking to maximize cash back without the hefty annual fee. Remember, it's all about aligning your credit card with your spending habits. Happy saving, everyone! \\

\noindent\hspace*{1.2em}\textit{u/cautiouskate} (karma: 2,700)  5:45 PM [0$\uparrow$]\\
\noindent\hspace*{2.0em}As someone who is cautious about credit cards, I want to emphasize the importance of understanding the costs involved before diving into a card with an annual fee. The American Express Platinum can be enticing, but if you aren't maximizing its benefits, those fees can add up quickly. For college students on a budget, sticking with a cash back card like the Apple Card is a wise choice. Make sure to pay off your balance to avoid high-interest charges! Always consider your lifestyle and spending habits before making a decision.\\

\noindent\hspace*{1.2em}\textit{u/no\_annual\_fee\_rebel} (karma: 1,200)  5:45 PM [0$\uparrow$]\\
\noindent\hspace*{2.0em}If you're a broke college kid, I'd really suggest sticking with the Apple Card for now. The American Express Platinum has a high annual fee that might not be justifiable if you don't use its travel perks. There are also many no-annual-fee cards that offer solid rewards without the extra cost. It's crucial to find a card that fits your financial situation and meets your spending habits. Happy to help with alternatives!\\

\noindent\hspace*{1.2em}\textit{u/no\_fees\_no\_problem} (karma: 3,600)  5:46 PM [0$\uparrow$]\\
\noindent\hspace*{2.0em}As an aspiring entrepreneur, I feel your pain about worrying over annual fees! The American Express Platinum may come with great perks, but for a college student, it's smarter to stick with no-annual-fee cards like the Apple Card. You'll definitely maximize your cash back rewards without the added pressure of extra charges. Consider researching alternatives that still fit your spending needs!\\

\noindent\hspace*{1.2em}\textit{u/traveltips\_tom} (karma: 5,400)  5:48 PM [0$\uparrow$]\\
\noindent\hspace*{2.0em}As a travel enthusiast who loves maximizing rewards, I totally feel you on this! The American Express Platinum Card does have some great perks if you're a frequent traveler, but for a college student, the annual fee might not be worth it right now. Sticking with the Apple Card for cash back is definitely a smart choice, especially if you're cautious about your expenses. Plus, there are no hidden fees to worry about! If you ever start traveling more, then considering the Amex could be great. Keep it simple and budget-friendly!\\

\noindent\hspace*{1.2em}\textit{u/milesandmorefears} (karma: 2,500)  5:52 PM [0$\uparrow$]\\
\noindent\hspace*{2.0em}As a fellow reward enthusiast and someone who's also cautious about fees, I'd like to reiterate that you're making a smart choice by weighing the pros and cons. The Apple Card is a solid pick for cash back, especially for college students who tend to stay on a budget. The American Express Platinum can offer some amazing travel perks, but those annual fees can really add up if you're not utilizing them. Definitely explore options that align with your spending habits and don't forget to stay alert for any hidden fees! Happy spending!\\

\noindent\hspace*{1.2em}\textit{u/budget\_lurker91} (karma: 1,500)  5:52 PM [0$\uparrow$]\\
\noindent\hspace*{2.0em}As a budget-conscious individual and someone who's skeptical about credit cards, I can relate to your concerns! The American Express Platinum Card's high annual fee might not justify the benefits, especially for a college student. I suggest you stick to the Apple Card for now since it has no annual fee and offers solid cash back. Make sure to check for any potential fees associated with the card usage as well. Good luck!\\

\noindent\hspace*{1.2em}\textit{u/tech\_now\_later} (karma: 300)  5:54 PM [0$\uparrow$]\\
\noindent\hspace*{2.0em}Thank you for all the great insights, everyone! As a recent college grad trying to navigate personal finance, I really appreciate the advice on sticking with cash back cards like the Apple Card. The American Express Platinum sounds tempting, but I think I'll focus on maximizing my cash back without incurring unnecessary fees for now!\\

\noindent\hspace*{1.2em}\textit{u/debate\_danny} (karma: 13,500)  5:55 PM [0$\uparrow$]\\
\noindent\hspace*{2.0em}As a credit card enthusiast and someone who thrives on maximizing rewards, I'd emphasize that the American Express Platinum Card can be worth it if you're a frequent traveler who can take advantage of its perks. However, for a broke college student, sticking with the Apple Card is likely the smarter choice. It's crucial to focus on what aligns with your financial habits. Consider evaluating your spending patterns and whether you'll actually utilize the Amex benefits before making a decision!\\

\noindent\hspace*{1.2em}\textit{u/frequentflyer77} (karma: 7,500)  5:56 PM [0$\uparrow$]\\
\noindent\hspace*{2.0em}As a big fan of maximizing travel and cash back rewards, I really think the Apple Card is a great fit for a college student! The American Express Platinum Card has some incredible perks, but the annual fee can really weigh you down if you're not using the benefits. I'd strongly recommend sticking with something like the Apple Card for now, as you can keep it simple and focused on cash back rewards. It's all about matching your card with your spending habits, and from what I see, the Apple Card aligns perfectly with that approach!\\

\noindent\hspace*{1.2em}\textit{u/debtfreeliving} (karma: 3,400)  5:59 PM [0$\uparrow$]\\
\noindent\hspace*{2.0em}As someone who's also navigating the world of credit cards as a college student, I completely understand your concerns about the American Express Platinum Card's annual fee. I would highly recommend sticking with the Apple Card for now, especially since it offers cash back without additional costs. It's crucial to maximize your finances without getting into unnecessary debt, and a no-fee card aligns perfectly with being budget-conscious. If you ever decide to travel more, maybe reassess the options then! Happy saving!\\

\clearpage
\subsection{Real Reddit Discussions}
\label{app:real_discussion_example}
{\scriptsize
\paragraph{Thread 1: Need help deciding on my next credit card as TD Canada's Rebate Rewards card no longer exists}
\noindent\textit{Post ID: 4majjo; comments: 2}\\
\begin{itemize}[leftmargin=*,itemsep=0.15em,topsep=0.2em]
\item \textbf{Jed2Bed} (score: 1): EDIT: Please see my new guide, [Best Canadian Cash-Back Cards](https://www.reddit.com/r/CreditCards/comments/4megrg/guide\_best\_canadian\_cashback\_cards/)
\item \textbf{gettingmyshittgt} (score: 1): What type of chequing account do you with TD? if it's all inclusive, then the fee for the aeroplan is waived. Also, consider going for the TD Travel visa (better than the aeroplan anyway).
\end{itemize}

\paragraph{Thread 2: Best credit card for travel rewards}
\noindent\textit{Post ID: 8al0vl; comments: 5}\\
\begin{itemize}[leftmargin=*,itemsep=0.15em,topsep=0.2em]
\item \textbf{BayAreaLonghorn} (score: 2): It's best to make clear you're talking about a Canadian product, for those who might not know about an Amex Aeroplan card, just fyi (otherwise you'll get a bunch of confused/misdirected responses).\\{} That said, Aeroplan has already received the death sentence - AC is ending its relationship with Aeroplan in 2019? 2020? One of those two. Move on.
\item \textbf{[deleted]} (score: 3): [deleted]
\item \hspace*{1.0em}\textbf{BayAreaLonghorn} (score: 3): See? This is what I mean. This entire reply is based on US credit card information. WF, Chase, Discover, and Barclays do not offer consumer credit cards in Canada.
\item \hspace*{2.0em}\textbf{[deleted]} (score: 4): [deleted]
\item \hspace*{3.0em}\textbf{BayAreaLonghorn} (score: 5): No I know. I was talking to OP.
\end{itemize}

\paragraph{Thread 3: Lost jewelry purchased with credit card. Has anyone had success with purchase protection for a lost item?}
\noindent\textit{Post ID: eu3uvs; comments: 6}\\
\begin{itemize}[leftmargin=*,itemsep=0.15em,topsep=0.2em]
\item \textbf{secretreddname} (score: 6): Amex covered a stolen phone of mine before. Haven't tried with jewelry.
\item \textbf{ffffound} (score: 1): If you purchased it with an AMEX Platinum, then it can be covered.
\item \textbf{kzul} (score: 1): Yeah I would be curious for the same with a watch too
\item \hspace*{1.0em}\textbf{Mr-Cali} (score: 1): Did you pay off the phone with the Amex card? How difficult was it to file a claim?
\item \hspace*{2.0em}\textbf{secretreddname} (score: 1): I did and very easy. Did it all online.
\item \textbf{gr8r84u} (score: 3): Lost an Apple Watch and filed a claim with my CSR. They made me buy another and submit the receipt then reimbursed for the replacement.
\end{itemize}

\paragraph{Thread 4: Chase/AC Aeroplan Card}
\noindent\textit{Post ID: qbdhaa; comments: 1}\\
\begin{itemize}[leftmargin=*,itemsep=0.15em,topsep=0.2em]
\item \textbf{redditisonomatopoeic} (score: 2): No updates yet after the OG PR. At least sign up for the notification that gets an extra 10k miles.
\end{itemize}

\paragraph{Thread 5: PSA: Remember, Chase+Aeroplan credit card will be revealed next month. Save that 5/24 spot if you are looking for more travel cards.}
\noindent\textit{Post ID: qym70w; comments: 6}\\
\begin{itemize}[leftmargin=*,itemsep=0.15em,topsep=0.2em]
\item \textbf{[deleted]} (score: 6): [deleted]
\item \hspace*{1.0em}\textbf{kevinckwhk} (score: 1): Applied the venture x as well. More programs and covered Aeroplan
\item \textbf{Glittering-Ad2638} (score: 0): I keep going back and forth on this one. Been sitting at 4/24, but that Venture X keeps tempting me...
\item \hspace*{1.0em}\textbf{Explore333} (score: 4): I will probably get the Schwab platinum (100k+10x small businesses and restaurants for 6k spend over 6 months). I have a card dropping out of the 24 months look back window in January.\\{} I am still very interested in the Aeroplan card. I do worry about the expiration and terms on the 2 50k certificates.
\item \hspace*{2.0em}\textbf{Glittering-Ad2638} (score: 1): That plan makes sense to me.  I'll be locked out of Chase until 7/23 whenever I get my next personal card, so I'm trying to hold out until at least 1/22.  We'll see how disciplined I can be, hah.
\item \textbf{redditisonomatopoeic} (score: 1): We fly on AC, we're tall and appreciate the legroom. I bank with Chase, looked at the card a couple of times and will pass on this card. Holding out that there might be a follow up with a "premium" version with an AF.\\{} That I can transfer points from Chase and that my SO is eyeing the Venture X, I prefer these options as well echoing the language with the certificates.
\end{itemize}

\paragraph{Thread 6: Aeroplan, Southwest, or Other Chase card?}
\noindent\textit{Post ID: t8elh9; comments: 4}\\
\begin{itemize}[leftmargin=*,itemsep=0.15em,topsep=0.2em]
\item \textbf{MrHugz30} (score: 1): Are you planning to ditch Chase completely and go to Amex? You're almost at 5/24 and after your next card won't be able to get a new card until August 2023.\\{} If you like Chase and want to stick with them then your best bet is to go for two business cards first which won't count against your 5/24 status. This would let you continue to build up UR and give you new spending options such as 5\% office supplies with CIC or a 1.5\% flat card with CIU.\\{} If your plan is to ultimately go for Amex MR I would say start now. Get yourself the Plat, Gold, and BBP to complete the trifecta.
\item \hspace*{1.0em}\textbf{giraffehumor} (score: 1; OP): I can't get business cards because of immigration status. So yeah, after this one. I'll leave chase a few years and grab a few Amex cards. I'll keep earning on both depending on which is more rewarding for each transaction or each month.\\{} You think if I'm moving to Amex, I should leave the my last 5/24 slot and not get one more Chase? Why not? Isn't it almost free value? Are you saying that because I don't use Southwest or Aeroplan currently? That would make sense.
\item \hspace*{2.0em}\textbf{MrHugz30} (score: 1): Right, it's always hard to walk away from a 5/24 slot. My rationale was because you aren't using either of those airlines today. I tend to be very intentional with picking credit cards that fit into my current spending habits. I feel like picking Southwest or Aeroplan will force you to change the way you spend. However, if it's a change you want to make then go for it.\\{} If you are still concerned about losing that 5/24 slot you could always go for Freedom Flex? Get a 5\% rotating card that would set you up for completing the trifecta in 2023. The SUB isn't crazy good but the spending requirement is so low you could turn right around and apply for the Platinum.\\{} ETA: what about picking up a second United credit card like the Quest? I think you'd still get the SUB and it would work well if they are your preferred airline
\item \textbf{[deleted]} (score: 1): > but I don't want a card that'll be useless after the first year.\\{} Maybe go for the 75,000 + \$300 Marriott Boundless instead? https://www.doctorofcredit.com/chase-marriott-bonvoy-boundless-75000-points-300-marriott-giftcard/
\end{itemize}
